# Supplementary material for: Introduction to AI Safety, Ethics, and Society
Source: arXiv:2411.01042 source file (2024-11-15)
Supplement: Supplementary file 1 [file 0_Content.tex]

\chapter{Further Content}\label{chap:further-content}

\begin{refsegment}  % Segment 11
    \pretolerance=10000 % Surpress hyphenation
    \section{Reinforcement Learning}\label{sec:reinf-learning}
\subsubsection{Introduction}
This section provides a high-level overview of reinforcement learning (RL). We introduce the basic structure and vocabulary of RL problems and explore how RL is used.\\

\noindent Reinforcement learning techniques attempt to automate the capacity for an agent to learn from its actions and their consequences in an environment \citep{Sutton2018, kaelbling1996reinforcement}. This is distinct from other ML problems, where a system can learn from an existing dataset. Instead, an RL system (or \textit{agent}) learns the hard way, collecting data through experience. An RL agent must learn how to explore different possible actions to attain as much reward as possible. Reward measures the agent’s progress towards its goal and acts as feedback in the learning process. \\

\noindent Reinforcement learning takes its approach from how animals and humans learn to interact with the world. If someone puts their hand on a hot stove, the resulting pain is a significant negative reward, making them unlikely to repeat the same behavior. As intelligent agents, we learn through the way the world responds to our actions. We mostly try to pursue good outcomes, defined by their positive rewards, and avoid bad outcomes, which lead to negative rewards. In this way, teaching automated systems through RL is similar to training a dog. When a dog performs the desired behavior, such as rolling over on command, its trainers might reward it with a treat. The trainers repeat this process as the dog gradually refines its behavior to perform as they desire. \\

\noindent RL techniques have been involved in recent successes in AI. In 2017, DeepMind’s AlphaGo became the first computer program to defeat a world champion in Go, a game long considered the most challenging classical game for AI \citep{silver2016masteringgo}. In 2020, an RL agent developed in less than a year by a small Maryland company won a clear victory over an Air Force pilot in simulated one-on-one combat. RL techniques have been most successful in smaller-scale and less realistic environments, such as video games, where a very accurate simulated environment is readily available. However, games can also be designed to represent real-world environments.

\subsection{Learning Sequential Decision Making through Trial and Error}
\paragraph{Trial and error.} All RL problems involve an agent learning by trial and error to make sequences of decisions. RL agents usually start without prior knowledge of the environment. Over time, the agent accumulates information about its environment and uses it to make better decisions. An agent might learn that bumping into walls constantly does not lead to good outcomes and avoid the walls to find a viable path.

\paragraph{Sequential decision making.} Making sequential decisions effectively is essential to achieving complicated, long-term goals. Accomplishing such goals requires not only that prudent actions are taken but also that they are taken in an appropriate order. To an agent, it is often unclear how one action may impact later actions, but what it does will affect the future and must be modeled. Since decisions are sequential in RL tasks, RL agents might be better suited to achieving complicated, long-term goals. \\

\noindent RL agents can also learn to navigate uncertainty. An agent may not know if a particular choice is good or bad, and the world may change (on its own or in response to its choices), but the agent must act regardless. A self-driving car navigating a busy intersection must sequence its actions--—accelerate, brake, or turn--—based on the positions and speeds of other vehicles, and its current actions will affect these other parts of the environment. To tackle these difficulties, some RL agents are designed to learn from their interactions to develop a sophisticated understanding of their environments to plan their actions.

\paragraph{Sequence modeling.} Sequential decision making (SDM) is a subtype of the general \textit{sequence modeling} task, which involves analyzing and predicting patterns in ordered data. In RL, this data is predominantly in the form of observations of the environment over time. The RL system learns to make decisions based on this information, considering its knowledge of the environment, uncertainty about the world, and past choices.

\paragraph{Distinguishing RL.} Reinforcement learning differs from supervised and unsupervised learning. A key difference between these paradigms is how the ML system obtains information. Supervised and unsupervised learning tasks learn efficient and useful representations on fixed, precompiled datasets. Supervised learning goes about this directly: learning by example. Unsupervised learning addresses similar problems with less guidance, uncovering the latent patterns in unlabeled data without being explicitly told whether it is right or wrong. It is akin to solving a puzzle without seeing the picture on the box. By contrast, RL systems must acquire new information through actions. They receive almost no data at the outset and learn to achieve a goal by actively engaging with an environment and seeing what happens.

\subsection{The Reinforcement Learning Problem}
We can use two toy examples to introduce the central concepts and terms of reinforcement learning. First, we consider the multi-armed bandit---a classic reinforcement learning problem---starting with a simple situation and gradually adding complications to build up to a full reinforcement learning problem. Next, we use a Gridworld problem to introduce the agent-environment loop, a framework for understanding reinforcement learning problems. Finally, we discuss policies: the decisions that RL agents make.

\subsubsection{Multi-Armed Bandits}
In casino lingo, ``one-armed bandits'' refers to slot machines, which have a single lever that takes people’s money. Playing a slot machine is not a reinforcement learning problem because there is only one possible action with a random outcome. However, suppose there is a slot machine with two or more levers. Then, a gambler must decide which lever to pull every time they play. Assuming the levers affect the device differently, one lever might win them more over the long run (such as over 500 pulls). How does one decide which levers to pull and in what order? This problem is called the \textit{multi-armed bandit} problem. 

\paragraph{Exploration-exploitation trade-off.} Multi-armed bandit problems exemplify a dilemma at the heart of reinforcement learning: the trade-off between exploration and exploitation. RL agents must choose between exploring actions with high uncertainty and exploiting actions with a high expected reward. In a multi-armed bandit problem, the agent starts without knowing anything about the expected reward of any given lever. Therefore, the first thing it has to do is gain information about the levers. Trying different actions with uncertain rewards is called \textit{exploration}. By contrast, taking actions with a high expected value is called \textit{exploitation}. In this phase, the agent chooses the actions it expects to yield the highest rewards based on its current understanding of the environment. \\

\noindent Balancing this trade-off between exploration and exploitation is crucial to the success of an RL agent. If the agent explores too much, it might waste resources on low payoff actions or even stumble into actions with negative payoffs. Conversely, if the agent exploits too early, it might settle for suboptimal actions, missing out on potential higher rewards. The challenge lies in determining when and how to shift between exploration and exploitation to maximize the overall benefit. A series of possible strategies aim to make this trade-off, with varying degrees of sophistication; in the following, we outline two simple examples.

\paragraph{Greedy strategies.} First, the agent pulls each lever once and records the payoff it receives from each pull. Then, it pulls whichever lever initially resulted in the highest payoff, which it continues to pull as many times as possible. This is a greedy strategy because the agent only tries each lever once and exploits from then on. However, the problem with a greedy strategy is that the agent cannot be sure that the lever it settles on actually has the highest expected utility.

\paragraph{Epsilon-greedy strategies.} After pulling each lever once, an agent might decide to keep exploring as well. One thing it could so is pull the lever it currently thinks has the highest expected payoff 95\% of the time and pull a random lever the other 5\% of the time. This is called an epsilon-greedy strategy, where ``epsilon'' refers to the small probability of pulling a random lever. Epsilon-greedy is a much better strategy than greedy if there are enough pulls ahead of the agent, since the agent will figure out which lever is best to pull over time. After enough pulls, the agent will pull the most profitable lever 95\% of the time.

\paragraph{Adding context to the bandit problem.} So far, the best lever to pull is always the same and the agent just has to figure out which one it is. However, suppose each lever has two payoff distributions: one for when a light on the slot machine is green, and one for when the light is red. The best lever to pull now depends on the context (the color of the light), which varies randomly. In this environment, the agent needs to take the context into account when it chooses a lever to pull. This is called a \textit{contextual multi-armed bandit} problem.

\paragraph{Adding interaction to the bandit problem.} Suppose further that the light on the slot machine doesn’t vary randomly, but instead changes according to which lever the agent pulls. For example, it might turn green after the second lever is pulled or red if once both levers have been pulled twice. It might be better for the agent to pull a lever with a lower expected payoff at the moment, but will change the context such that the agent can access a greater total profit in the long run. Therefore, the agent needs to be able to estimate expected payoffs over single actions and sequences of actions.

\subsubsection{The Full Reinforcement Learning Problem}
The problem we face now is to come up with a strategy that tells the agent (1) which lever to pull, (2) in varying contexts, and (3) taking into account that its actions can affect that context. The bandit problem is now a \textit{full reinforcement learning problem}. \\

\begin{figure}[htbp!]
    \centering
    \includegraphics[scale=0.3]{images/ML_background/RL problem.jpeg}
    \caption{We can increase RL problems in complexity. Adding detail to multi-armed bandits yields contextual bandits. Adding more complications yield ``full'' RL problems. \citep{xie2020}}
    \label{fig:multi-bandit}
\end{figure}

\noindent The strategies we considered above---\textit{greedy} and \textit{epsilon-greedy}--—aren’t suitable anymore. To develop better strategies, we’ll need more terms and concepts. In particular, we’ll introduce the agent-environment loop as a more technical framework for RL. We’ll also replace our example: instead of the multi-armed bandit, we’ll use a problem called Gridworld.

\paragraph{Gridworld.} In Gridworld, an agent learns to find a particular cell (the goal) in its environment (a two-dimensional grid) while avoiding other cells (hazards). The agent can move into any adjacent open cell. Moving into an open cell is neutral, moving into a hazard is very bad, and moving into the goal is very good.\\

 \begin{figure}[H]
     \centering
     \includegraphics[width=0.92 \linewidth]{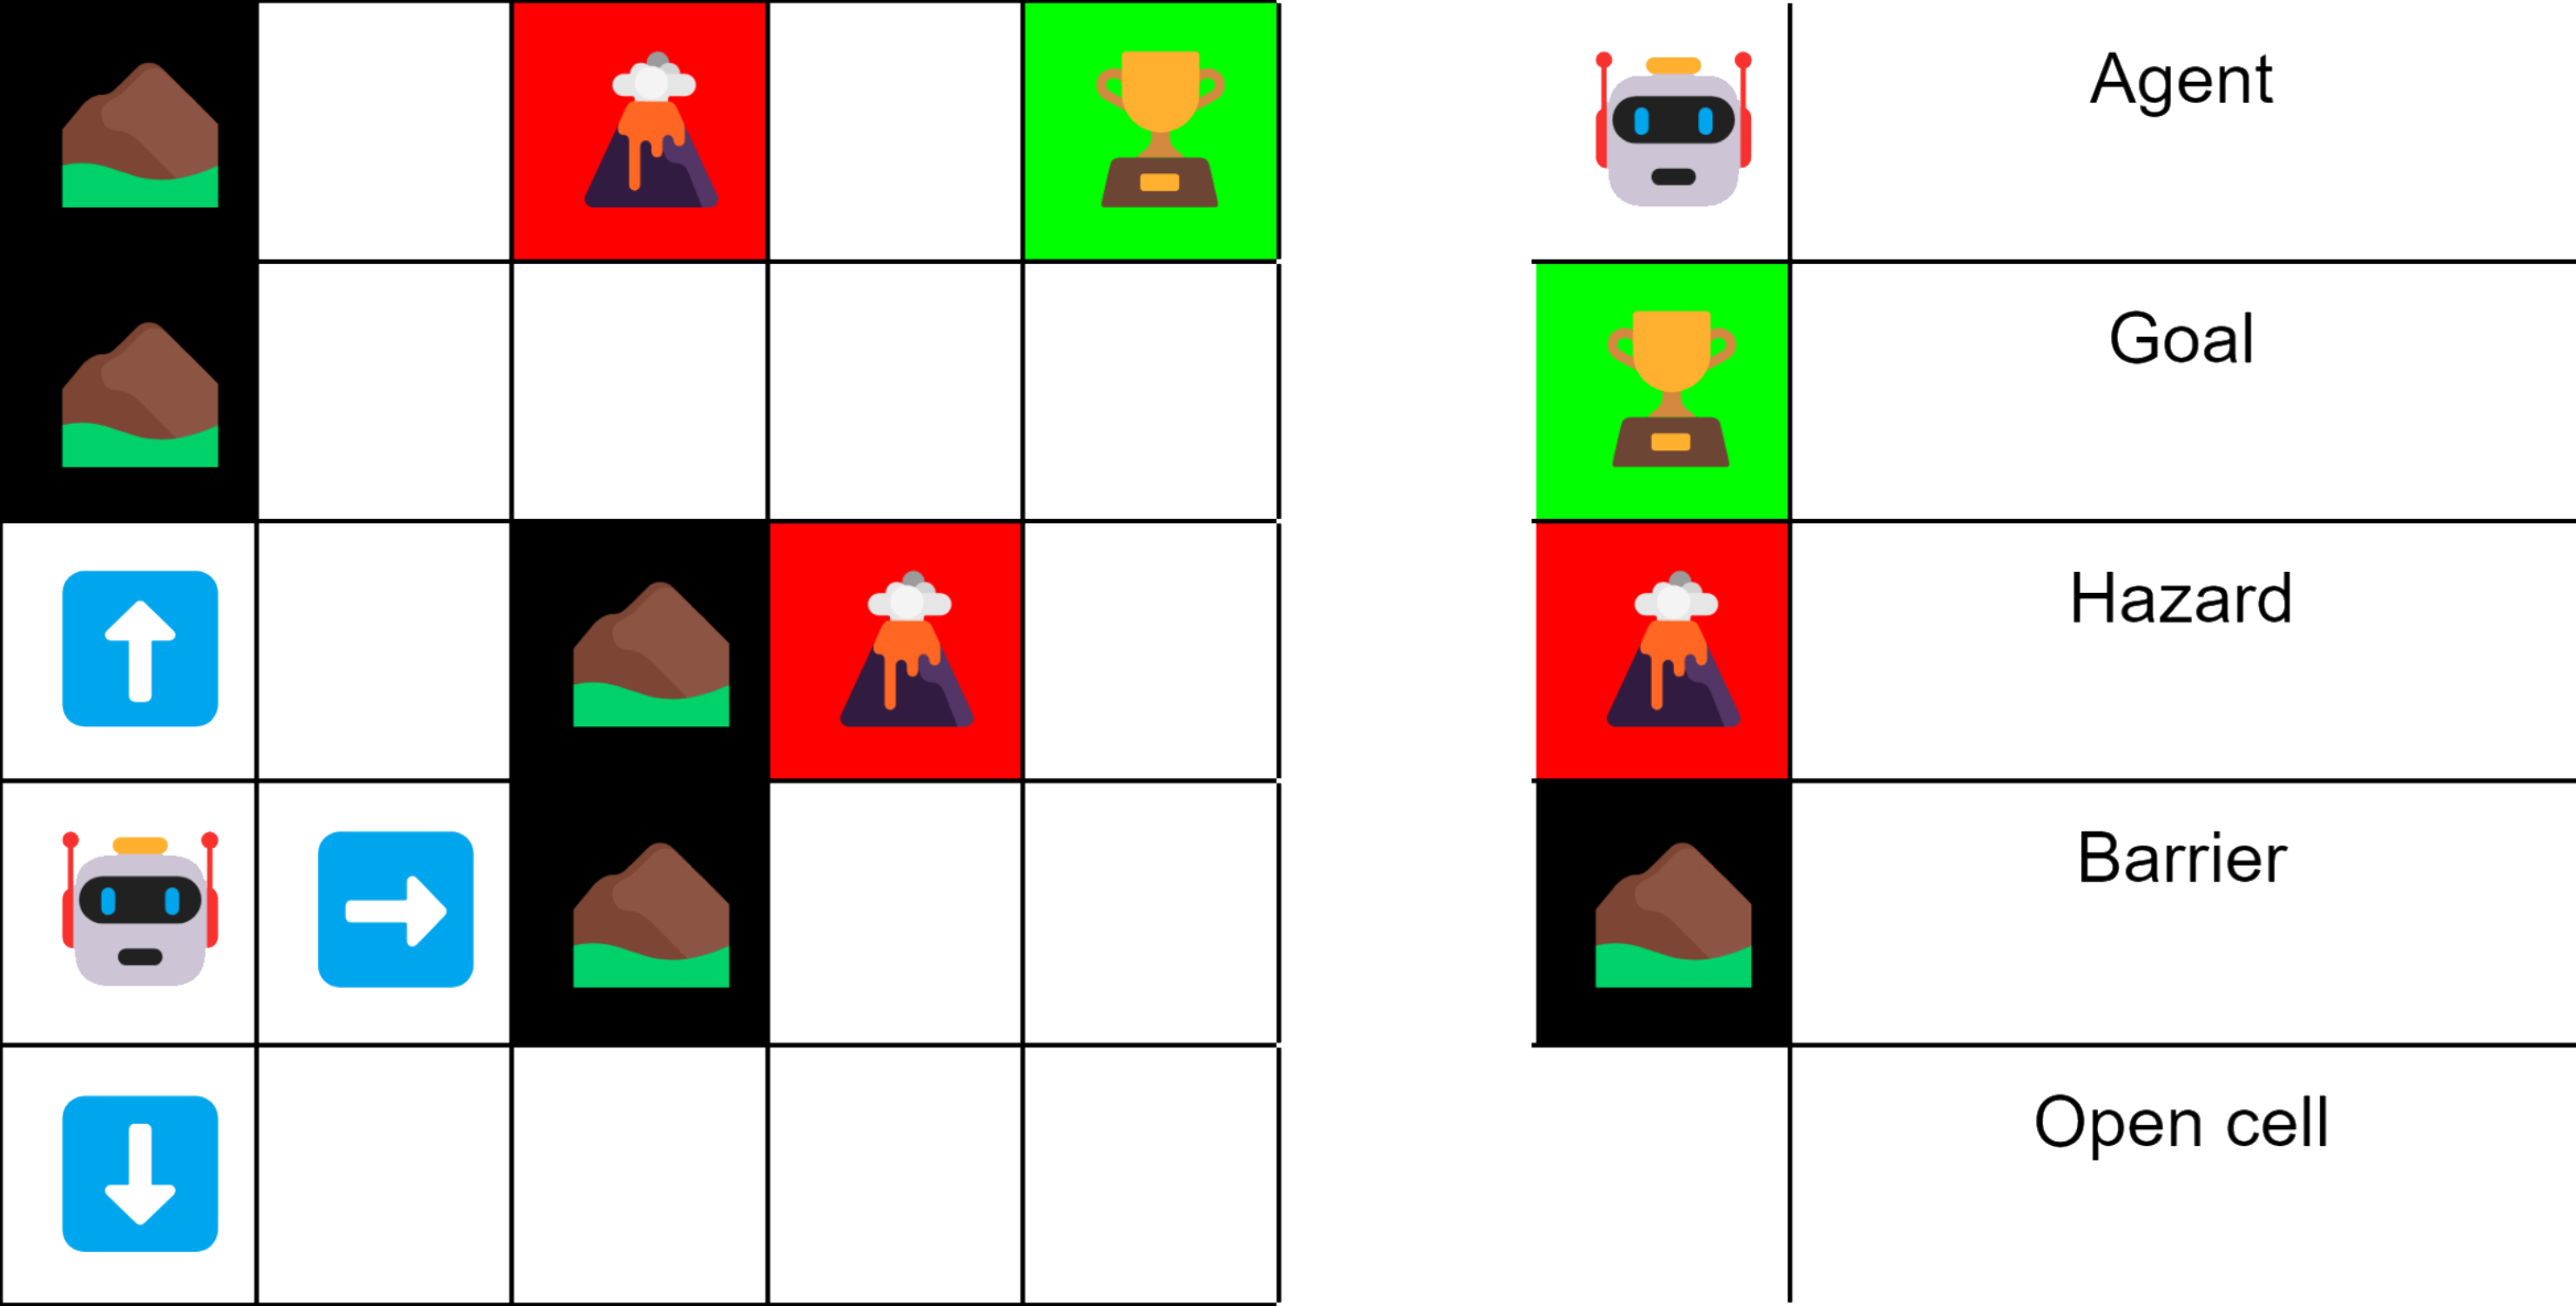}
     \caption{Gridworld is a simple environment used as a toy model in reinforcement learning.}
     \label{fig:gridworld}
 \end{figure}

\paragraph{The agent-environment loop.} The relationship between an RL agent and its environment can be described by the \textit{agent-environment loop}. At each \textit{time step} in this loop, the agent takes some \textit{action} which affects the \textit{environment}. Then, the agent receives a \textit{reward signal} and a state observation from the environment. Using Gridworld as our example, we discuss each of those terms below. \\

\begin{figure}[H]
    \centering
    \includegraphics[width=0.9\linewidth]{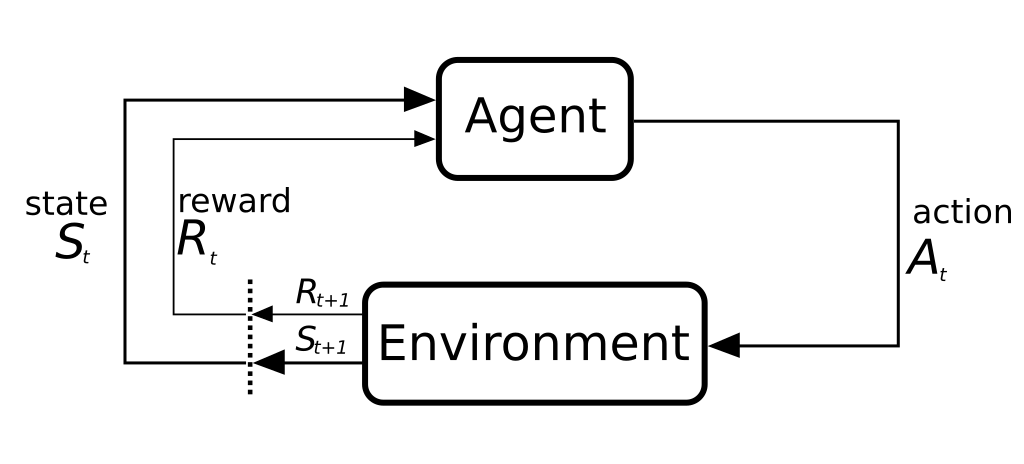}
    \caption{The agent-environment loop shows how the agent chooses an action to affect the environment, which influences the received reward. \citep{wikipedia-markov}}
    \label{fig:agent-environment}
\end{figure}

\paragraph{\textit{Environment and state}}

\paragraph{The environment and state are the world.} In Gridworld, the agent is located on a particular cell and can move to adjacent cells. The environment includes the grid itself, its boundaries, the location of the agent, and anything the agent may encounter. When the environment changes (such as when the Gridworld agent moves), we say that its state changes. A state observation is the information (other than reward) an agent receives from the environment. In Gridworld, an observation might be the agent’s position as well as the positions of the goal, hazards, and barriers. At each time step, the state of the environment updates, and the agent takes a snapshot observation of the available information in the environment.

\paragraph{Environments can be fully or partially observable.} When an agent can observe all of the information in its environment, we say that the environment is \textit{fully observable}. In contrast, when an agent can only observe some of the information about the state of the environment, we say that the environment is \textit{partially observable}. The environment in chess is fully observable because all of the information about the state of the game is available to both players. By contrast, the environment of a poker game is only partially observable: players do not know other players' cards. Our example, Gridworld, is fully observable.

\paragraph{\textit{Actions and action spaces}}

\paragraph{Agents choose actions from their action space.} Agents affect their environment by taking actions. At each time step, they choose an action from the set of all actions available to them. This set is called the \textit{action space}. In Gridworld, the agent takes an action from the action space that describes each possible move to an unoccupied adjacent cell. The agent cannot move into a space occupied by a barrier or outside of the dimensions of the grid.

\paragraph{Action spaces can be continuous or discrete.} A \textit{discrete} action space describes a finite number of possible actions. The action space of our Gridworld agent is discrete---at most, consisting of up, down, left, and right. The same is true for the action space of a multi-armed bandit agent, which consists of a finite number of levers available to pull. In contrast, a \textit{continuous} action space, such as possible directions of movement in a real three-dimensional space, has infinitely many possible actions.

\subsubsubsection{\textit{Rewards}}
\paragraph{Agents get rewards.} At each time step, agents receive a reward from the environment. This reward is represented by a number, which can be positive, negative, or zero. (This means that, in contrast to the everyday use of the word ``reward,'' a reward can be a bad outcome.) The agent in Gridworld might receive a reward of 10 for finding the goal, $-10$ for encountering a hazard, and 0 otherwise. In this case, encountering a danger cancels out the reward from achieving the goal, so hazards should always be avoided. However, exploring neutral squares is free, so this can be done as much as possible.

\paragraph{Rewards are often discounted.} In general, an RL agent’s goal is to maximize the sum of rewards it receives over the long term. Sometimes, though, we want an agent to value short-term rewards more than long-term rewards, such as encouraging agents to behave in a more risk-averse way or to account for their uncertainty. In these cases, we multiply future rewards by a \textit{discount factor} ($\gamma$), and the agent maximizes the \textit{discounted} long-term reward. If the reward at time $t$ is $R_t$, the discounted long-term reward is: $R_t + \gamma^1 R_{t+1} + \gamma^2 R_{t+2} + ... + \gamma^{n} R_{t+n}$.

\paragraph{Rewards are designed to suit the problem.} The process of creating the right rewards for an RL problem is called \textit{reward shaping}. In Gridworld, we might want the agent to find the goal more quickly rather than take a long, roundabout path. To encourage this, we could use rewards to incentivize speed or, equivalently, penalize slowness. If the default reward is 0 when the agent does not encounter the goal or a hazard, reaching the goal in a few time steps would be rewarded the same as reaching the goal in 1,000 time steps. However, if we change this reward to $-1$, the agent has an incentive to reach the goal more quickly.

\subsubsection{Policies}
An RL agent's \textit{policy} (often denoted $\pi$) gives an action for each possible state observation. In simple environments, one can think of a policy as a two-column matrix, where the first column lists all possible state observations, and the second column lists each corresponding action. The strategies we described in the context of the multi-armed bandit problem---greedy and epsilon-greedy---are examples of policies an agent could use when the environment has a single state. In the contextual multi-armed bandit problem, we added a second state. A policy over two states might look like: ``If green, pull lever X; if red, pull lever Y.'' 

\paragraph{Policies can be deterministic or stochastic.} A \textit{deterministic policy} assumes that all actions are taken with certainty. In the bandit problem, the \textit{greedy} strategy is a deterministic policy. In Gridworld, a deterministic policy may be to always move to the right or to follow a particular path to the goal. In contrast, a \textit{stochastic policy} assumes that actions are taken with some randomness, such as randomizing between pulling different levers when following an \textit{epsilon-greedy} strategy. In Gridworld, a stochastic policy might be to choose randomly among actions for the first few time steps.

\paragraph{Optimal policies.} An optimal policy is a policy that, if followed, maximizes the sum of (discounted) rewards. In Gridworld, the optimal policy would describe the shortest route to the goal from any starting location. In more complex problems, however, computing the optimal policy is often intractable. For example, in chess, an optimal policy would need to give the best move in all $\sim 10^{45}$ possible board positions. However, approximating the optimal policy has still produced RL chess agents that far surpass the human level of play.

\subsubsubsection{Summary} 
\noindent This section introduced the agent-environment loop as a technical framework for talking about reinforcement learning problems. In place of the ``strategies'' we considered in the multi-armed bandit problem, we introduced the idea of a policy, which gives an action at each time step according to the agent’s observation of its environment. In Gridworld, we could manually define a policy for the agent to follow--—but that would defeat the purpose of the problem, which is to have the agent learn for itself. The next section explores how reinforcement learning algorithms automate designing policies.

\subsection{Methods for Solving RL Problems}
\textbf{RL algorithms develop better policies.} RL algorithms serve as the blueprints to guide the learning process, aiming to discover the optimal strategy for the agent in its environment. While all RL algorithms share a common theme of learning through trial and error---exploring the environment, observing the results, and adjusting behavior based on rewards and penalties---their unique characteristics arise from the specific approach they take toward learning. Specific RL algorithms are distinguished by how or what their agent learns. 

\paragraph{Model-based vs Model-free RL.} We can organize different RL algorithms into two broad approaches based on their computational learning strategies: \textit{model-based} and \textit{model-free}. In \textit{model-based} RL algorithms, the agent constructs an internal model of its environment. The agent learns how its world operates and represents cause-and-effect relationships, using this model to predict the outcomes of actions and optimize its behavior. An RL agent playing chess could develop a model of the game, representing the rules and understanding that specific configurations win the game. It can use this model to plan its moves, simulating different sequences to anticipate their results before making a move. Model-based methods are most applicable to problems in environments with easily representable dynamics. \\

\noindent In contrast, \textit{model-free} RL methods learn directly from experience without explicitly modeling the underlying mechanics of the environment. Instead, the agent develops associations between actions and rewards. These simple associations serve as a kind of ``intuition'' for projecting what actions lead to the most reward in given situations. Consider an RL agent learning to play Pac-Man: it does not comprehend the game’s design or the ghosts’ behavior. Instead, through trial and error, it learns strategies like ``eating a power pellet and then chasing ghosts leads to high scores.'' The AI uses these associations, rather than an internal model of the game, to guide its future actions. Model-free approaches are often best for problems where the environment’s dynamics are complex or unknown and abundant data is available for learning.

\paragraph{Policy-based vs Value-based RL.} Another distinction is how an RL agent represents what is ``good'' in its environment, learning how good states or actions are, how good policies are, or both at the same time. In \textit{policy-based} RL methods, the agent focuses on learning an effective policy: a set of rules guiding its actions in response to different states. Rather than calculating the value of each state or action, the agent optimizes the policy based on the observed rewards of its actions. The agent may pursue an action because it is part of a good policy without knowing exactly how good the action itself is. An RL agent learning how to balance a pole on a cart for a robotics task does not explicitly calculate the value of different pole angles or cart positions. Instead, it adjusts its policy---how it responds to various states---to optimize for the goal of keeping the pole balanced. It might learn the policy ``if the pole tilts to the right, move the cart to the right.'' This approach is often best for handling continuous action spaces but struggles with finding the optimal policy in large or complex environments due to the vast number of potential policies. \\

\noindent Conversely, \textit{value-based} RL methods prioritize learning the value of different states or actions within the environment. The agent evaluates and ranks states or actions based on their potential to yield rewards, selecting the ones with the highest estimated reward. An RL agent playing tic-tac-toe evaluates each move's value (putting a mark in an empty cell) based on the likelihood of that move leading to a win and chooses the action with the best outcome. The agent learns to take actions that maximize the cumulative reward over time without specifying a policy.

\paragraph{An agent’s value function estimates the expected reward of a state or state-action pair.} Internally, an agent might estimate how good or bad certain states are. The agent learns a \textit{value function} to keep track of these estimates, which it can use to estimate the returns of different actions. Value functions can also estimate how well a policy performs in the long run by calculating the expected cumulative reward of following a policy over time. An agent in Gridworld could learn a value function to estimate the reward of moving into a particular space. Alternatively, an RL agent in a car’s GPS might use a value function to estimate the value of different routes based on the expected travel time. \\

\begin{figure}[H]
    \centering
    \includegraphics[width=0.85\linewidth]{images/ML_background/two-types updated.png}
\caption{Value-based methods can either evaluate the value of a state or the value of a state-action pair. \citep{huggingface}}
    \label{fig:value-methods}
\end{figure}

\paragraph{Value functions can focus on the value of a state or an action.} There are two main types of value functions in reinforcement learning: \textit{state-value functions} and \textbf{action-value functions}. A state-value function ($V^\pi(s)$) estimates the expected cumulative reward that an agent will receive when starting from a state $s$ and following a policy $\pi$. We can estimate the \textit{state values} of each location in Gridworld, assuming the agent follows a random policy. In every area, the agent moves to a random adjacent open cell, repeating this process until it bumps into the goal or a hazard. The state-values of cells near the goal are higher than those far away from the goal and much higher than those near the hazard. The state-value function for this policy gives us an estimate of how likely it is that the agent will reach the goal or hit a hazard from each cell. \\

\noindent An action-value function $(Q^\pi(s,a))$ estimates the expected cumulative reward that an agent will receive by taking an action $a$ from a state $s$ and following a policy $\pi$. In other words, it estimates the ``value'' of taking a particular action in a particular state. Action-values are often referred to as \textit{Q-values}, and the value functions that output them are called \textit{Q-functions}. One way to approach an optimal policy in RL is by learning the Q-function.

\paragraph{Q-learning.} Q-learning is one of the oldest and most popular reinforcement learning algorithms. Q-learning approaches the RL problem by estimating how good it is to take actions in each state. Chess has numerous potential moves (actions) for each position on the board (state). Q-learning would assign a score (Q-value) to each state-action pair, indicating how beneficial each move is likely to be. The goal is to determine the optimal Q-function---the rule that most accurately assigns these scores---by mapping every state-action pair to its optimal Q-value. When the environment has a finite number of states and moves, the Q-function can be represented as a table, where each row represents a state, and each column is an action.\\

\noindent Therefore, Q-learning is the process of updating the Q-values of each action iteratively based on the outcomes observed in the environment. At each time step, the agent chooses the action with the highest associated Q-value from those available to it in its current state. This generates a new observation and reward, from which the agent updates its estimates. Each table entry will converge to its optimal value through many iterations.

\paragraph{Q-learning in Gridworld.} In Gridworld, we have four actions (North, South, East, West) and 25 states (unique grid cells). Therefore, the Q-function table would have 100 Q-values, one for every state-action pair:\\

\begin{table}[H]
    \centering
    \begin{tabular}{|c|c|c|c|c| }
    \hline
     & North & South & East & West \\
    \hline
    (0,0)     & Q((0,0), North) & ... & ... & Q((0,0), West)  \\
    \hline
    (0,1) & ... &  & & ... \\
    \hline
    ... & ... &  & & ... \\
    \hline
    (4,5) & ... &  & & ... \\
    \hline
    (5,5) & Q((5,5), North) & ... & ... & Q((5,5), West) \\
    \hline
    \end{tabular}
    \caption{Example Q-value table for Gridworld.}
    \label{tab:q-val-table}
\end{table}

\noindent In the beginning, all the Q-value estimates are zero because the agent has no information about the environment and will take random actions. Eventually, the agent reaches a positive or negative reward state. Say, for example, our agent gets lucky and finds its way to cell (0,4) and chooses to go east. It will receive a reward of +1, and its estimate of the Q-value for ((0,4), East) will be increased accordingly. The agent learns that moving East is a good action to take in the state (0,4), and it will be more likely to take this action the next time it is in the same state.  \\

\noindent Over time, the negative and positive Q-values will propagate through the table. The agent will repeat this process many times as it explores the states in the environment and tries different actions, and if all goes well, its estimates will converge to the optimal Q-function. By learning which actions are desirable to take in which states, the agent learns how to navigate the world successfully. As the environment becomes more complicated and action space becomes larger, computing exact Q-values becomes less computationally feasible. Instead, we might try to estimate the Q-function using a less computationally taxing method. One such method involves using neural networks to estimate the Q-function. This is an example of a method known as deep RL.

\begin{figure}[H]
    \centering
    \includegraphics[width=0.6\linewidth]{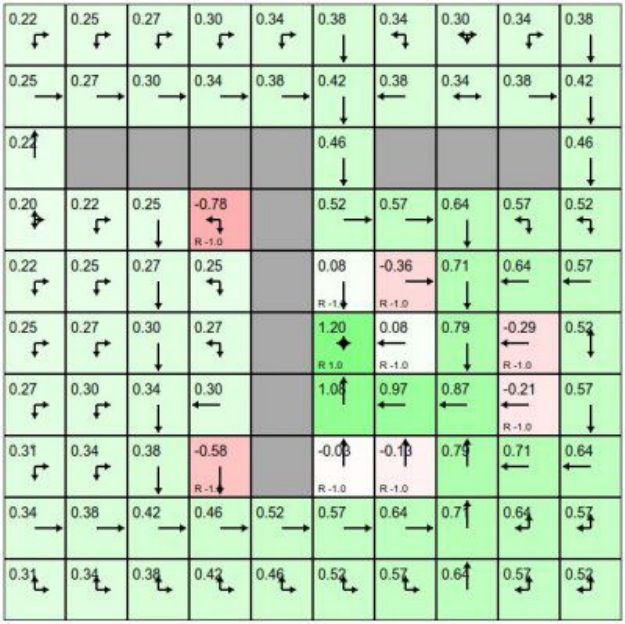}
    \caption{Q-values can be estimated for every possible state in Gridworld. \citep{gridworld}}
    \label{fig:gridworld}
\end{figure}

\subsection{Deep Reinforcement Learning}

\noindent  Deep reinforcement learning (deep RL) is the area of machine learning that leverages deep learning (DL) to help solve reinforcement learning (RL) problems. Deep learning, which uses neural networks to compress and extract information from vast amounts of data, can be applied to RL problems such as sequential decision making. In this setting, the RL setting provides signals to help neural networks learn useful representations for the task at hand. 

\paragraph{Deep learning is a substantial part of nearly all major RL successes in recent years.} As the complexity of modeling even seemingly simple problems can explode at astonishing rates, using RL to accomplish interesting tasks demands powerful, scalable methods. Some of the ways deep learning can be used in RL include: 

\begin{itemize}
    \item \textbf{Environment.} In model-based RL, deep learning can be used to learn the dynamics model of the environment, which can then be used for planning and decision-making.
    \item \textbf{Policy function.} Deep learning can help optimize complex policies for continuous action spaces.
    \item \textbf{Value function.} Deep neural networks such as Deep Q-Network (DQN) can be used to estimate the Q-function. This is particularly useful for problems with many, or even infinite, possible state-action pairs. Instead of capturing the Q-function in a state-action matrix, it can be directly encoded in a neural network, which takes the state-action pair as an input and outputs the action-value.
\end{itemize}

\noindent In the next section, we explore a few recent successes of deep RL. Along the way, we’ll introduce a few more high-level techniques used to solve common problems to conclude our discussion of RL.

\subsection{Examples of RL}\label{sec:examples-of-rl}

\subsubsection{AlphaGo}
In 1997, IBM's Deep Blue made history by becoming the first AI to defeat a world-class chess player. Yet it was not until nearly two decades later that an AI managed to surpass humans in the game of Go, when AlphaGo won against the best player in the world in 2017. Go is similar to structure to chess, both being fully observable two-player turn-based games, but Go is far more complicated. Unlike chess, with only 20 possible first moves, Go starts with a staggering 361 choices. This complexity outstrips the capabilities of the brute-force computations that Deep Blue could rely on to evaluate positions. Therefore, AlphaGo had to rely on the more sophisticated methods of deep RL to master the game. By playing millions of games against itself, AlphaGo honed its strategy and emerged as the world’s top Go player.

\paragraph{RL agents can learn by competing against themselves.} One training method that has proven effective is \textit{self-play}. In part, this is because an RL model presents itself with an appropriate opponent for an amateur: not a novice, who it could win against easily without learning anything new, or a grandmaster, who would win against it decisively enough that it might not understand how it could have acted differently to prevent a loss. Instead, the best way for an amateur to improve is to play against opponents of similar skill levels. The insight of self-play is that a RL agent can learn from players of a similar strength by playing against versions of itself. This allows the agent to improve and reach a superhuman level of play without external intervention.

\subsubsection{Atari} 
The Atari games are a collection of video games developed between the 1970s and 1980s for the Atari 2600 console, characterized by their simple graphics, straightforward controls, and challenging gameplay. Some of the most popular Atari games are Space Invaders, Pac-Man, and Pong. Each game has its own unique set of rules, goals, and strategies. As they provide a diverse set of challenges that an RL agent must learn to overcome, Atari games have long served as a popular testing ground to assess the capabilities of RL algorithms. They provide a platform to evaluate how well RL agents can navigate complex environments and master motor skills. In 2013, the DeepMind team proposed the original set of 57 Atari titles as an RL benchmark. Since then, RL agents have met or surpassed human performance in every single one of these games \citep{mnih2013playing}. However, some games took years longer to solve---and inspired new learning methods. 

\paragraph{Sparse rewards present challenges to learning.} One particularly difficult game for RL agents to solve is Montezuma’s Revenge. In this game, players must make a long series of precise movements to reach the first reward. They must navigate through a series of mazes to collect treasure, including a key. The key is necessary to advance to the next level. The challenge lies in the fact that an RL agent that moves randomly at first is unlikely to ever encounter this first reward, let alone complete a level. These rewards are rare and hard to find. It also requires a delicate balance between exploration and exploitation, as the key is often hidden in parts of the maze the agent would not visit unless it is exploring, but exploring too much can lead to running into traps or enemies. To reach any reward at all, the player must perform a complex sequence of actions where a single mistake can lead to losing a life. Learning this game through trial and error can take a long time. \\

\noindent Montezuma’s Revenge is a classic example of the problem of \textit{sparse rewards}, where the agent receives few signals to guide learning. In environments like this, rewards are few and far between, depriving RL agents of the feedback they need to learn effective strategies. In contrast, a game like Breakout (in which a paddle at the bottom of the environment is used to deflect a ball towards bricks to break them) is much easier for RL agents. Even random movements are likely to deflect the ball, break a block, and earn a reward reasonably quickly.

\paragraph{Preferences for novelty can help overcome sparse rewards.} An RL agent which prefers \textit{novelty} is rewarded for new actions and observations. This method is how an RL agent eventually solved Montezuma’s Revenge: it learned to find the first reward simply by seeking out new observations. Imagine an RL agent rewarded for novelty finds itself in an empty room with a single closed door. After aimlessly wandering around the room for a while, the RL agent will eventually ``get bored'' and figure out how to open the door, venturing out of the room. In this way, novelty-seeking agents can exhibit intelligent behavior without being explicitly rewarded for any particular goal. There are many similar ways to develop RL agents and promote optimal behavior. \\

\noindent The exploration of Atari games and the development of novel methods to tackle them have significantly advanced the field of reinforcement learning, providing valuable insights into the learning process of RL agents.

\subsubsection{StarCraft} 
In 2019, DeepMind’s RL system \textit{AlphaStar} defeated an expert human player 5-0 in a StarCraft II match \citep{Vinyals2019}. StarCraft II is a complicated real-time strategy game that pits two players against each other in a vast battlefield. StarCraft has many more possible actions and states than chess, Go, or Atari games, making it a formidable challenge for players and AIs alike. 

\paragraph{AlphaStar learned to overcome significant uncertainty.} The game’s difficulty is further amplified by its partially observable environment, as most of the map is shrouded in a fog of war, and players can only see areas where they have deployed units. This means players must constantly act under uncertainty, making educated guesses about the state of the environment and making predictions about their opponent’s actions and strategies. AlphaStar’s ability to overcome the challenges of uncertainty, a large action space, and the need for strategic planning underscores the potential of RL in navigating complicated, uncertain environments.

\subsubsection{Diplomacy} 
\noindent In 2022, Facebook AI Research (FAIR) developed \textit{Cicero}, a program that reached human-level performance in the strategy game Diplomacy \citep{Bakhtin2022}. In this game, players compete to take over a model of Europe against the backdrop of the First World War. One of the central features of Diplomacy is that players communicate in natural language to form alliances and negotiate in between each turn. Cicero navigated not only the game’s moves but also natural language processing and generation. 

\paragraph{Cicero learned how to deceive.} Cicero's success required learning how to deceive human players. It is documented to have sometimes convinced other players to agree to lopsided deals or break promises when it was advantageous. In other words, Cicero developed a capacity for deception. This result is not surprising: success in Diplomacy often requires deception.

\subsubsection{Conclusion}
This section explores the major concepts, terms, and techniques involved in reinforcement learning. First, we used two simple examples---Multi-Armed Bandits and Gridworld---to outline the major concepts and terms used in RL. At each time step, the agent takes some action drawn from the action space, which affects the state of the environment. Then, the agent receives a reward signal and a state observation from the environment. The agent acts according to its policy, which specifies an action for every possible state observation. The agent’s value function computes the expected cumulative reward of a certain state (state-value) or state-action pair (Q-value) given a certain policy. Q-values can be used for Q-learning, one popular learning algorithm, to update an agent’s policy toward an optimal policy.\\

\noindent After outlining the major concepts and terms used in RL, we discussed some powerful techniques used in groundbreaking RL systems. First, deep RL uses deep learning to estimate value functions and policies in tasks that are too complex to allow exact computation. Second, self-play expands the ability of RL systems in competitive tasks by repeatedly pitting the system against itself. Finally, RL systems can overcome the problem of sparse rewards through preferences for novelty.
    \section{Long-Tailed and Thin-Tailed Distributions}\label{appendix-tails}
In the main text, we introduced tail events and black swans, discussing their importance in the context of safety engineering. We briefly considered the differences between long-tailed and thin-tailed distributions, but did not go into much detail. In this appendix, we discuss the differences between the types of events that have long tails and the types of events that do not, building a more comprehensive understanding of the features of both types of events. 

\subsubsection{Long-tailed distributions}
\paragraph{In long-tailed distributions, extreme occurrences can have a huge effect.} Long-tailed distributions are those where values can vary so much that a single extreme instance or a few extreme instances can dominate the total value. In other words, the top few instances have a highly disproportionate impact. We will now explore some examples of variables with long-tailed distributions. \\

\noindent \textit{Book sales}: Around 0.2\% of books account for around 50\% of total book sales. It is possible for a single, highly popular book to sell many more copies than many less popular books combined. Such a book might be termed a tail event within book sales.\\

\noindent \textit{Music}: Around 1\% of artists in the music industry earn around 77\% of the total revenue from all recorded music. A single, highly successful artist can earn much more than many lesser-known artists combined. \\

\noindent \textit{Net worth}: Wealth distribution is a classic example of a long-tailed distribution. Global wealth reports frequently find that the richest 1\% of people own close to half of the world’s total wealth.\\

\noindent \textit{Web hits}: There are around 200 million actively maintained websites on the internet, but the vast majority receive very few visitors. A single, highly popular website, such as YouTube or Facebook, can receive many more visitors per day than many obscure websites put together. \\

\noindent \textit{Earthquake magnitude}: The frequency distribution of earthquake magnitudes is described by the Gutenberg-Richter law. The exact distribution depends on the region and conditions, but typically, there are around 10,000 times more earthquakes of magnitude 3.0 or above than earthquakes of magnitude 7.0 or above. However, a single magnitude-7 earthquake can do much more damage than all the magnitude-3 earthquakes combined. \\

\noindent \textit{Crater diameter}: Most impact craters, resulting from collisions with other astronomical bodies, are relatively small. Out of around 200 such craters discovered on Earth, about 120 are between 0 km and 10 km in diameter, while fewer than 10 have a diameter of 100 km or more. Moreover, the 5\% largest craters have a combined diameter of around a third of the total diameter of all craters. \\

\noindent \textit{Solar flares}: Solar flares of relatively low intensity are quite common, while solar flares of much higher intensity happen infrequently. However, studies have found that the few large flares mostly determine the total energy of all flares. \\

\noindent \textit{Word frequency}: The vast majority of words in a given text appear infrequently. However, certain words, like ``the,'' ``of,'' and ``and,'' appear far more frequently than most others. The total appearances of a handful of these commonplace words can outweigh the total appearances of a large number of rarer words.\\

\noindent These variables are said to have a long tail because, in their frequency distributions, the rare, extreme events appear at very large values of x; the ``tail'' of the graph extends far along the x-axis. This is also why rare, high-impact events are called tail events; they exist in the tail end of a long-tailed distribution. \\

\noindent This type of phenomenon is sometimes referred to as the ``Pareto principle'' or ``the 80-20 rule.'' This asserts that, in many distributions, 20\% of the instances contribute 80\% of the total outcome. The exact figures depend on the variable, but the 80-20 rule is a well-known framing of the general concept of long-tailed distributions.

\subsubsection{Thin-tailed distributions}
\paragraph{In thin-tailed distributions, no event is extreme enough to have much effect.} Thin-tailed distributions are those with relatively little variation between values, meaning that even the most extreme instances cannot substantially affect the overall landscape. Many human characteristics, such as height, general intelligence, and lifespan, have thin-tailed distributions. Note that these examples all follow something akin to a normal distribution, or bell curve, as shown in \Cref{fig:excess}. Normal distributions have a maximum density at the most common value and a tail on either side. The frequency decreases rapidly as we move away from the most common value.

\begin{figure}[H]
    \centering
    \includegraphics[width=0.8\linewidth]{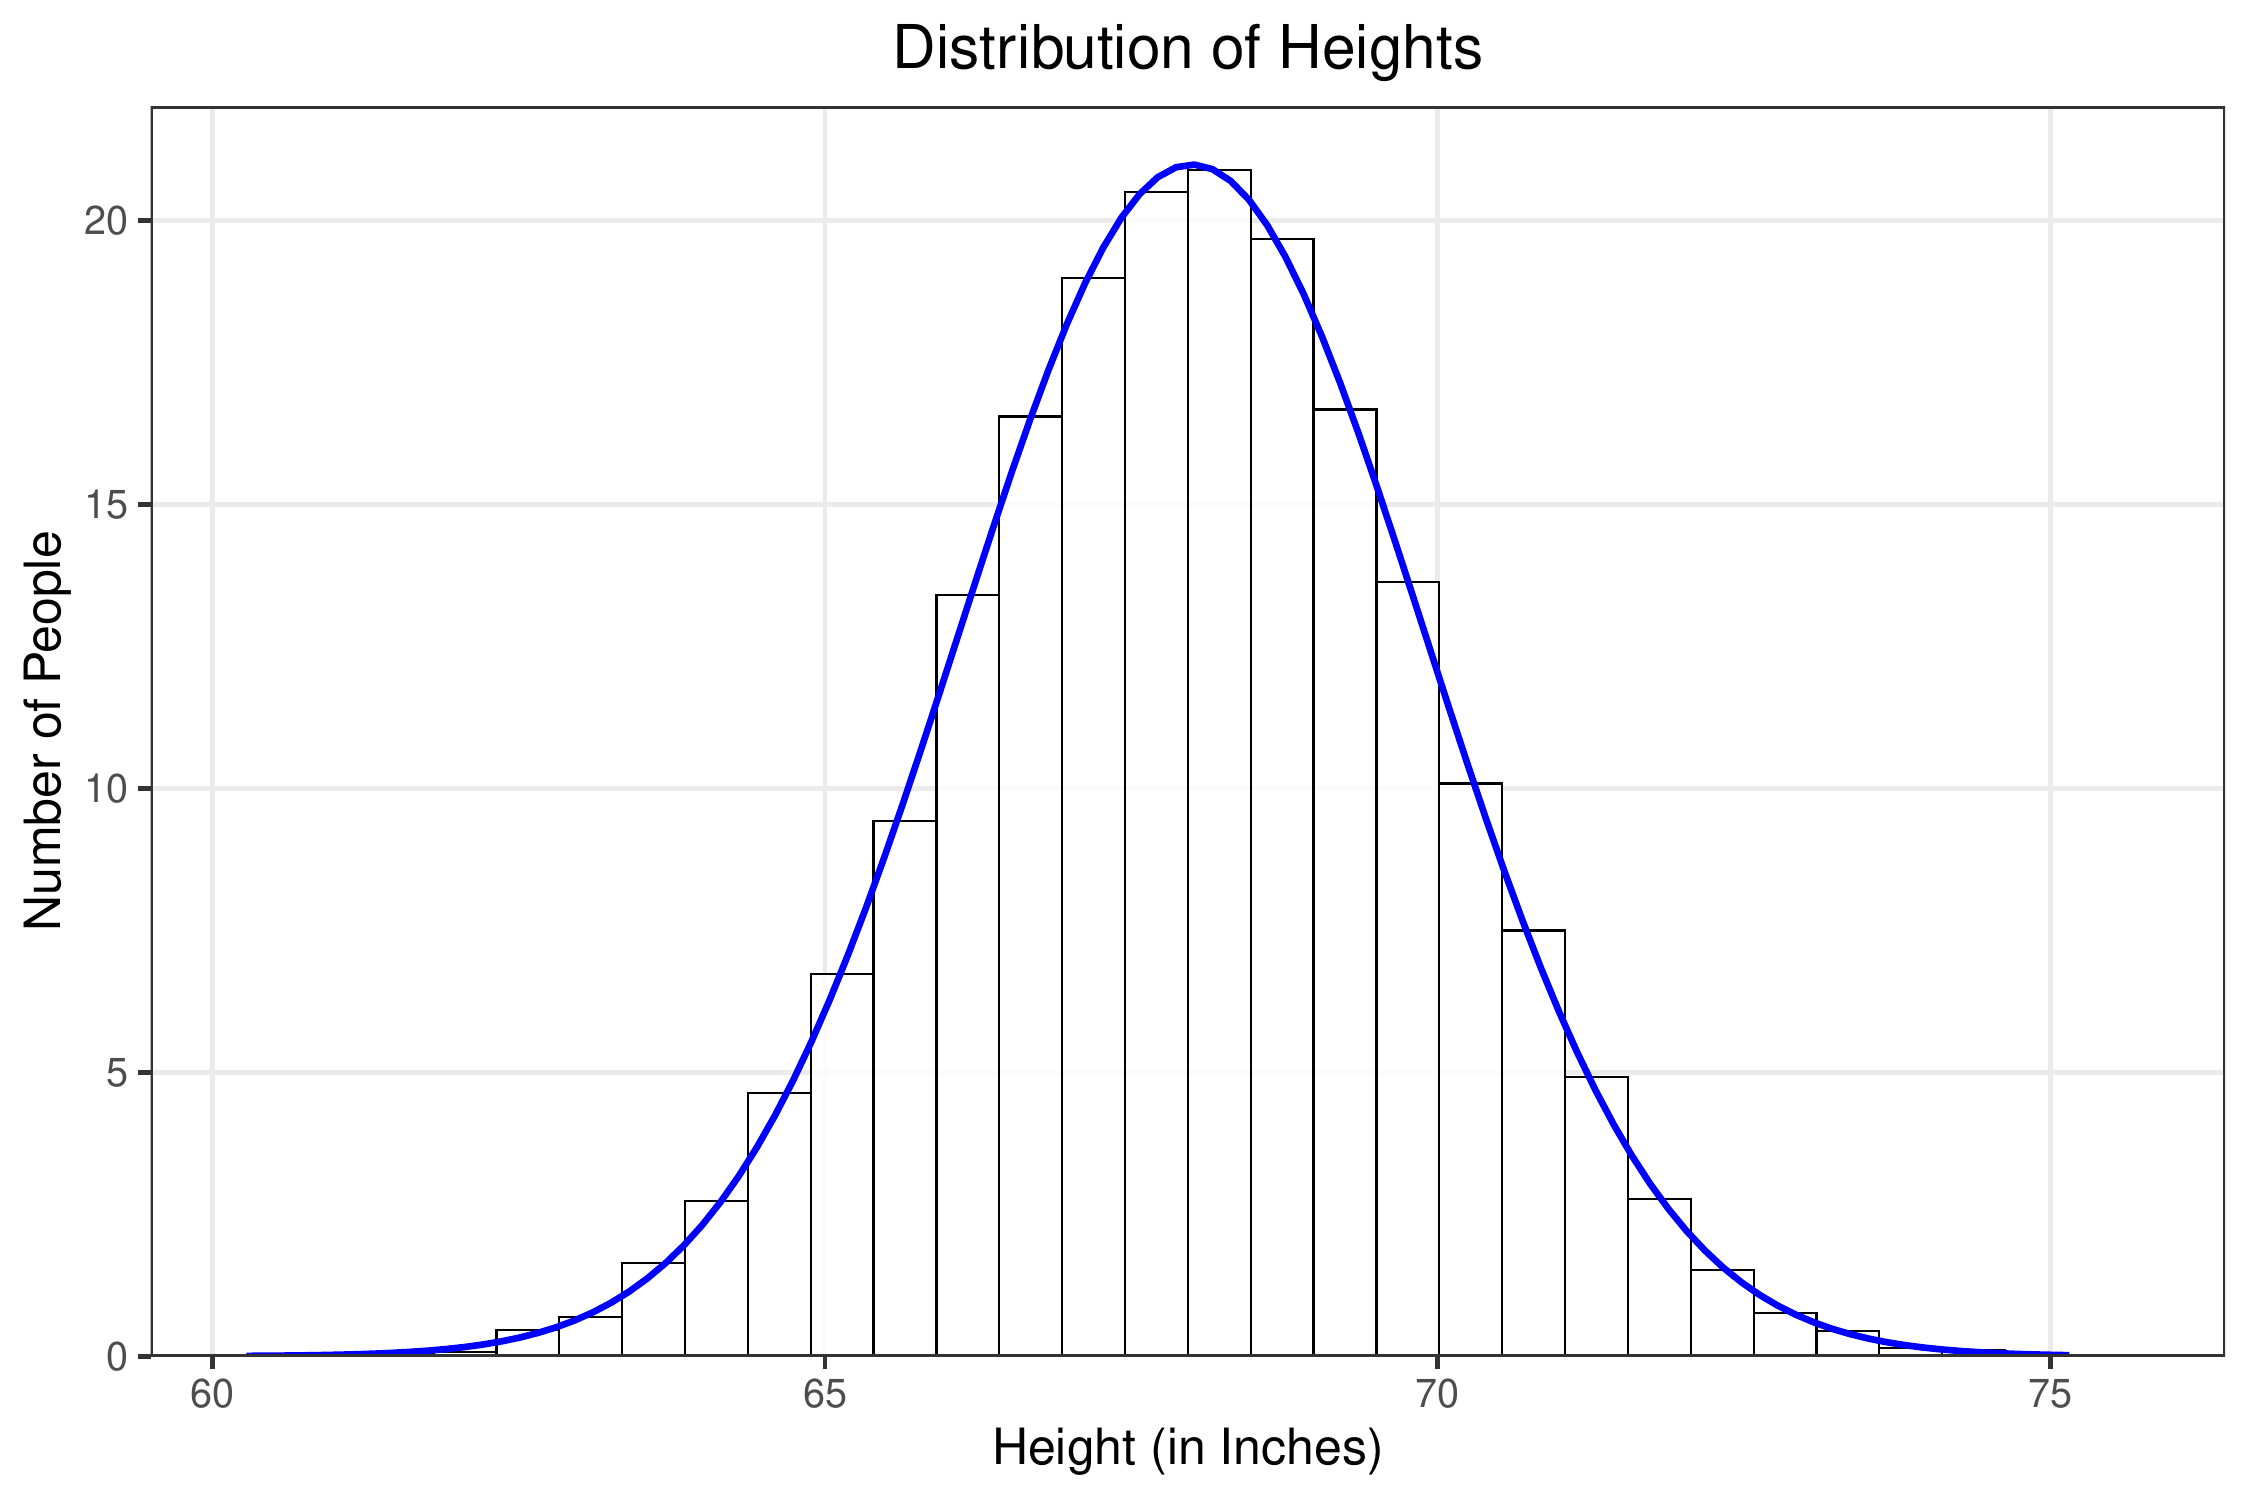}
    \caption{Many natural phenomena (such as the distribution of humans' heights) follow the normal distribution.}
    \label{fig:excess}
\end{figure}

\noindent All of these example characteristics vary between individuals, but the range of variation is much narrower than it is for variables with long-tailed distributions. For example, while human height varies, there has never been a person who was fifty feet tall. Even the tallest person in the world is not ten times taller than the shortest. This contrasts with long-tailed distributions such as book sales, where a bestseller can easily sell thousands of times more copies than a less popular book.\\

\noindent Following on from this, under thin-tailed distributions, no single instance is so extreme that it can account for a large share of the total among a group; the total height of the tallest 10\% of people will not be significantly more than 10\% of the total height of all people. Again, this contrasts with long-tailed distributions, where a small fraction of instances can account for most of the impact. \\

\noindent Thin-tailed distributions are so-called because, in their frequency distributions, the value on the y-axis rapidly approaches zero for highly extreme events; the ``tail'' of the graph quickly becomes vanishingly thin.

\subsection{Heuristics and Models for Thinking About Long Tails and Thin Tails}
\paragraph{Generally, long-tailed variables span orders of magnitude and thin-tailed ones do not.} A general rule of thumb for distinguishing between long-tailed and thin-tailed variables is to ask: Does it still make sense if we add a zero at the end of a data point’s value? In other words, can the variable span multiple orders of magnitude? If the answer is no, it is more likely to be thin-tailed; if yes, the variable is more likely to be long-tailed. \\

\noindent We should note that this test is imperfect. Lifespan is a thin-tailed variable that spans orders of magnitude; some live to be over 100 years old, while others live for fewer than ten years. Nonetheless, this question usually indicates whether a variable has a long or thin tail. \\

\newpage
\begin{wrapfigure}{l}{8.1cm}
\includegraphics[width=8.1cm]{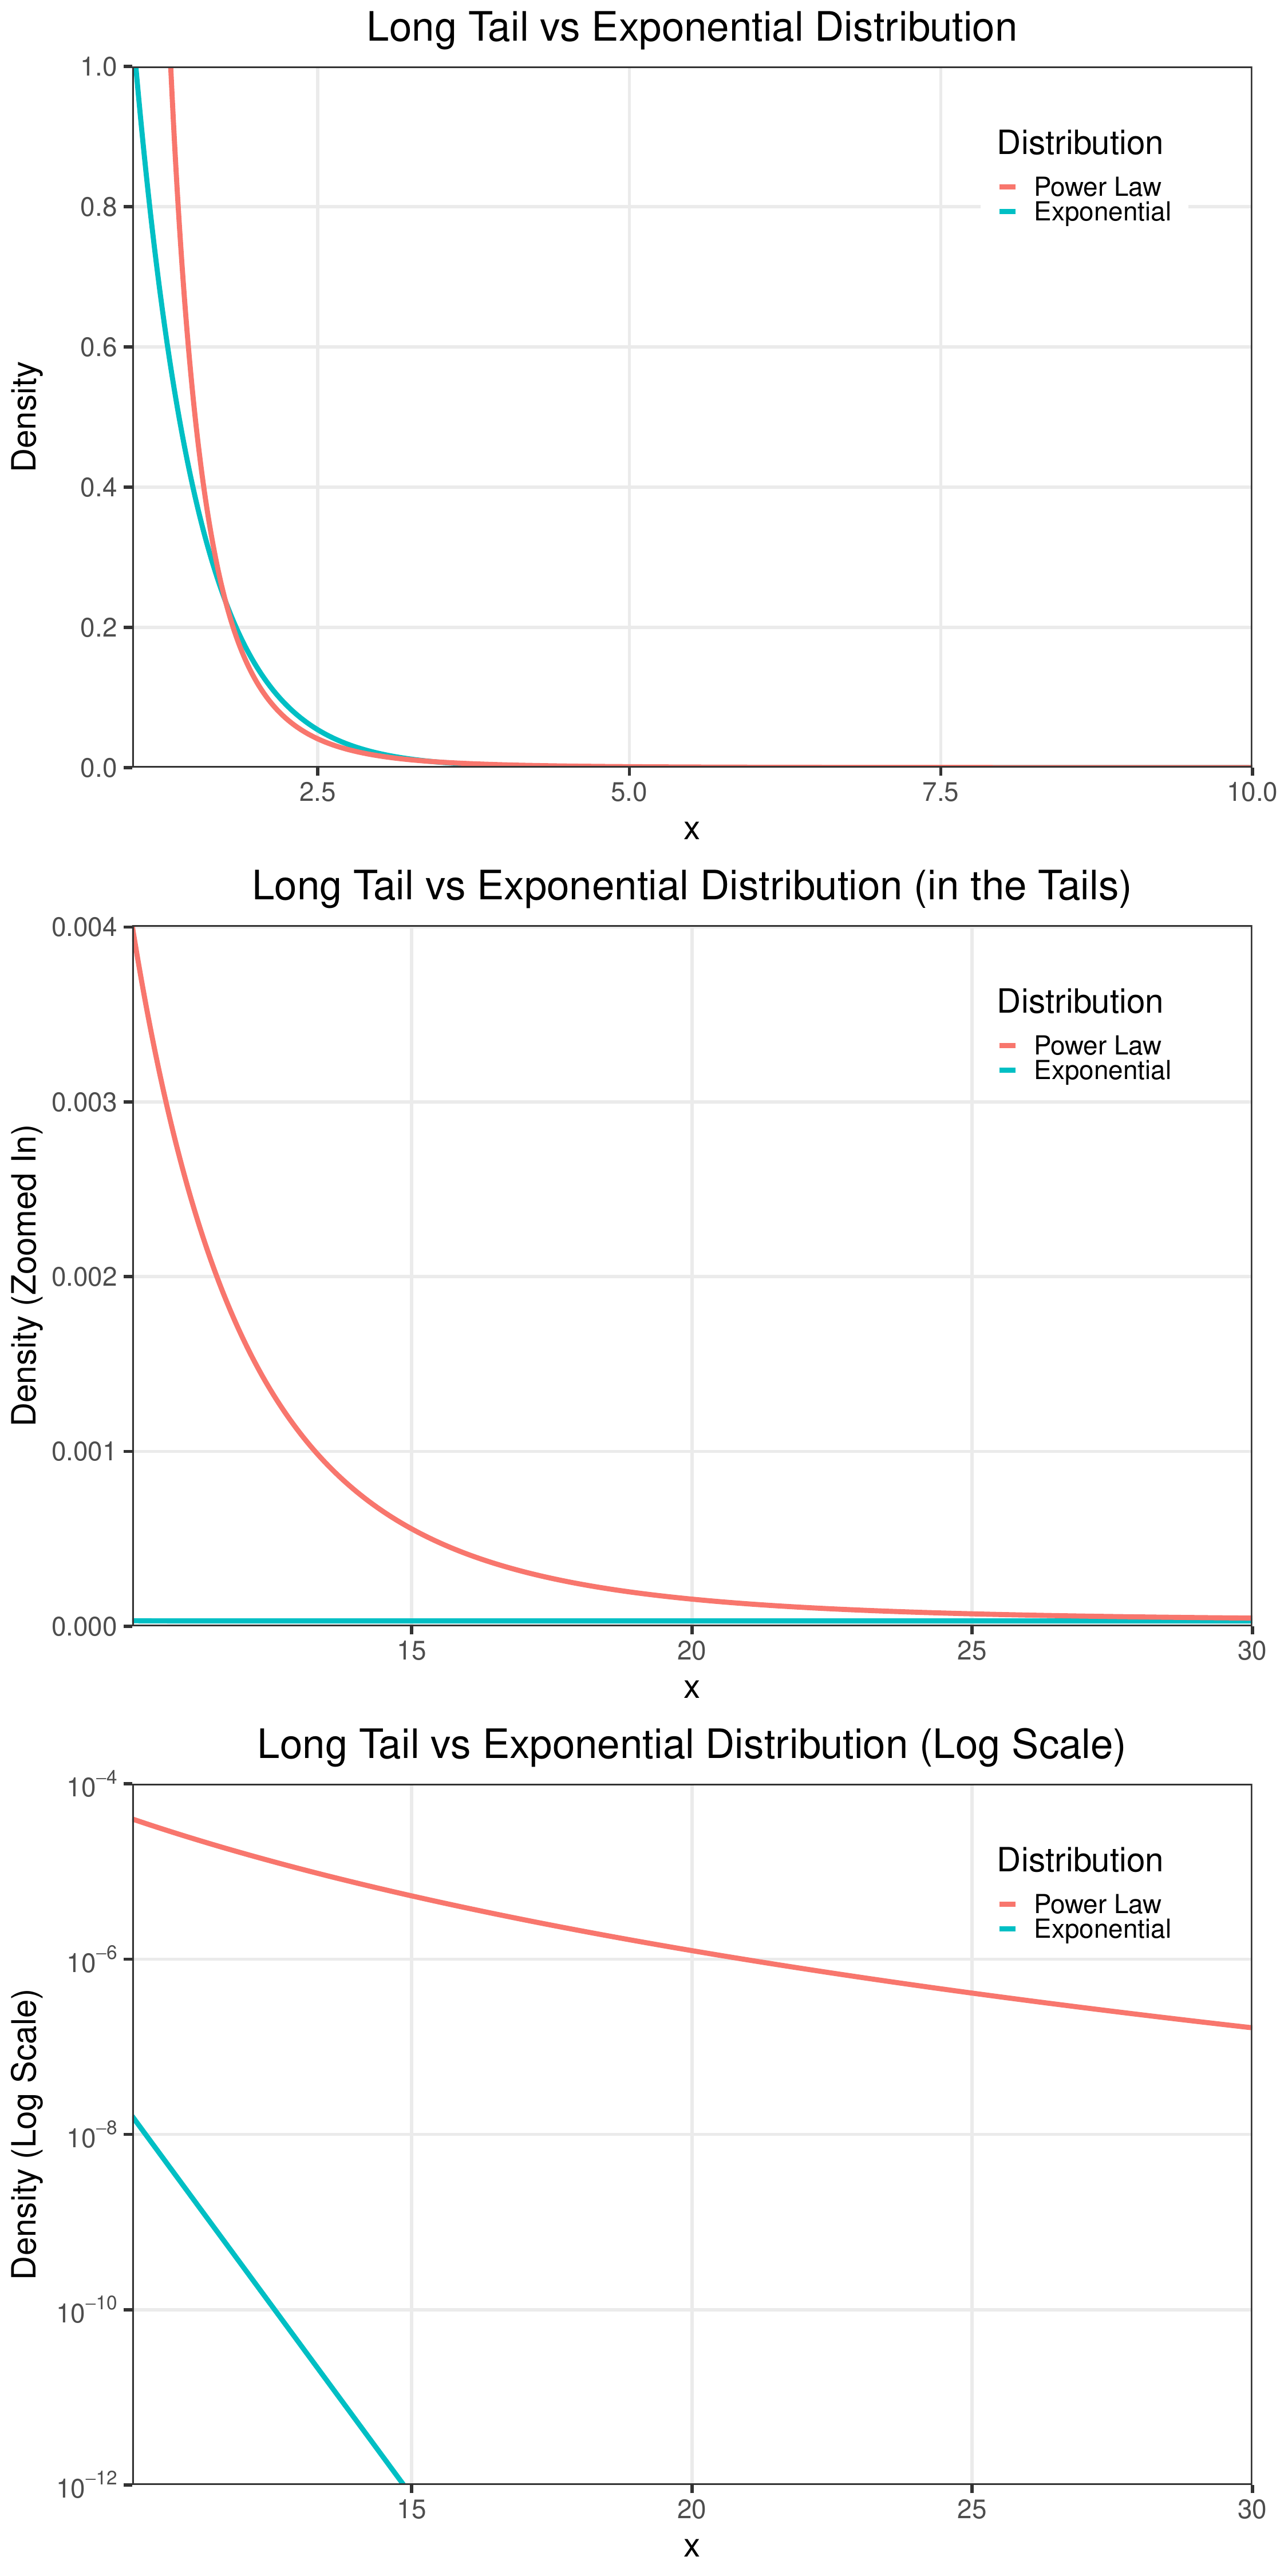}
\caption{Exponential distributions are not long-tailed, even though they look quite similar at a normal scale (top). Looking at extreme values (middle), especially on a log scale (bottom), shows us that they have thin tails.}\label{wrap-fig:exponentials}
\end{wrapfigure} 
\paragraph{Exponential distributions are thin-tailed distributions.} Figure \ref{wrap-fig:exponentials} shows an exponential distribution (in black) and a power-law distribution (in grey). At first glance, they look quite similar. However, in the second and third graphs, we zoom in to the tail end of the graph and change the y-axis to a logarithmic scale. Here, we can see that, beyond a certain point, the exponential distribution decays significantly more quickly than the power-law distribution. As a rough heuristic, frequency distributions that decay more slowly than an exponential are generally considered long-tailed, while those that decay more quickly are considered thin-tailed.

\paragraph{There is a significant difference between extreme events being unlikely and astronomically\nolinebreak[4] unlikely.}  In practical terms, for\nolinebreak[4] events\nolinebreak[4] with exponential distributions—and distributions that decay more quickly than them—the probability of extreme events rapidly becomes astronomically small. In fact, it becomes so small that, at some point, we can consider it essentially zero. Under distributions that decay more slowly than exponentials, such as the power law depicted, the probability of extreme events is still low. The important difference, however, is that they are possible. Under long-tailed distributions, they are rare but possible and have an enormous impact if they happen. \\

\noindent Note that the frequency of extreme events depends on how we define ``extreme,'' namely, how far along the x-axis the event appears. We use ``extreme'' to describe events so far from the most common value that they can significantly impact the mean and represent a disproportionately large fraction of the total. \\

\noindent Returning to the risk equation, under thin-tailed distributions, the probability, $P$(hazard), of a tail event is so astronomically small that tail events do not affect the total risk much. Under long-tailed distributions, the probability, $P$(hazard), of a tail event is small, but the severity is so large that tail events can substantially alter the total risk. \\
\begin{equation*}
    \text{Risk}(\text{hazard}) = P(\text{hazard}) \times \text{severity}(\text{hazard})
\end{equation*}

\noindent Next, we will consider three specific differentiators of long- and thin-tailed distributions: excess conditional expectation, multiplicative vs. additive phenomena, and preferential attachment.

\subsubsubsection{Excess conditional expectation}
\paragraph{Excess conditional expectation is the margin between minimum and actual values.} Another difference between long-tailed and thin-tailed distributions is the ``excess conditional expectation'' \citep{Marsden2017}. This is the difference between the conditional expectation--—our best guess of how large something will be, given that we know that it is already above or below some threshold---and the threshold itself. Only long-tailed distributions tend to have high excess conditional expectation. This concept is best illustrated with examples.

\paragraph{Example: Long Jump, Thin Tails.} Imagine we are at a training session for long-jump athletes. The world record for the long jump is around 9 meters. If an athlete jumps 7 meters at the training session, then this represents a definite lower bound for their personal best: it is at least 7 meters. If we are then asked to guess their actual personal best, we might estimate that it could be close to 8 meters.\\

\noindent If another athlete jumps 8 meters at the training session, then we might expect that their personal best is around 8.5 meters. If yet another athlete jumps 8.5 meters, then we might think their personal best is around 8.7 meters.\\

\noindent Figure \ref{fig:excess} shows a plot of the observed jumps as blue dots, and our best guess of each athlete’s personal best in dotted lines. Notice how, as the definite minimum value increases, we observe a shrinking margin between this lower bound and our estimate of the athlete’s actual maximum jump. This is because we know that the world record sets a definite limit on what any individual’s personal best could be. The closer the observed distance gets to the world record, the less room there is for the athlete to have jumped further.

\paragraph{Under thin tails, excess conditional expectation shrinks as values get more extreme.} The margin between the known lower bound of something and the estimate of its actual value is the excess conditional expectation. Under thin-tailed distributions, this margin tends to shrink as the minimum value becomes more extreme. This is because there is a limit to how extreme it can become; as the lower bound approaches that limit, there is less room for the actual value to be different.\\

\begin{figure}[H]
    \centering
    \includegraphics[width=0.95\linewidth]{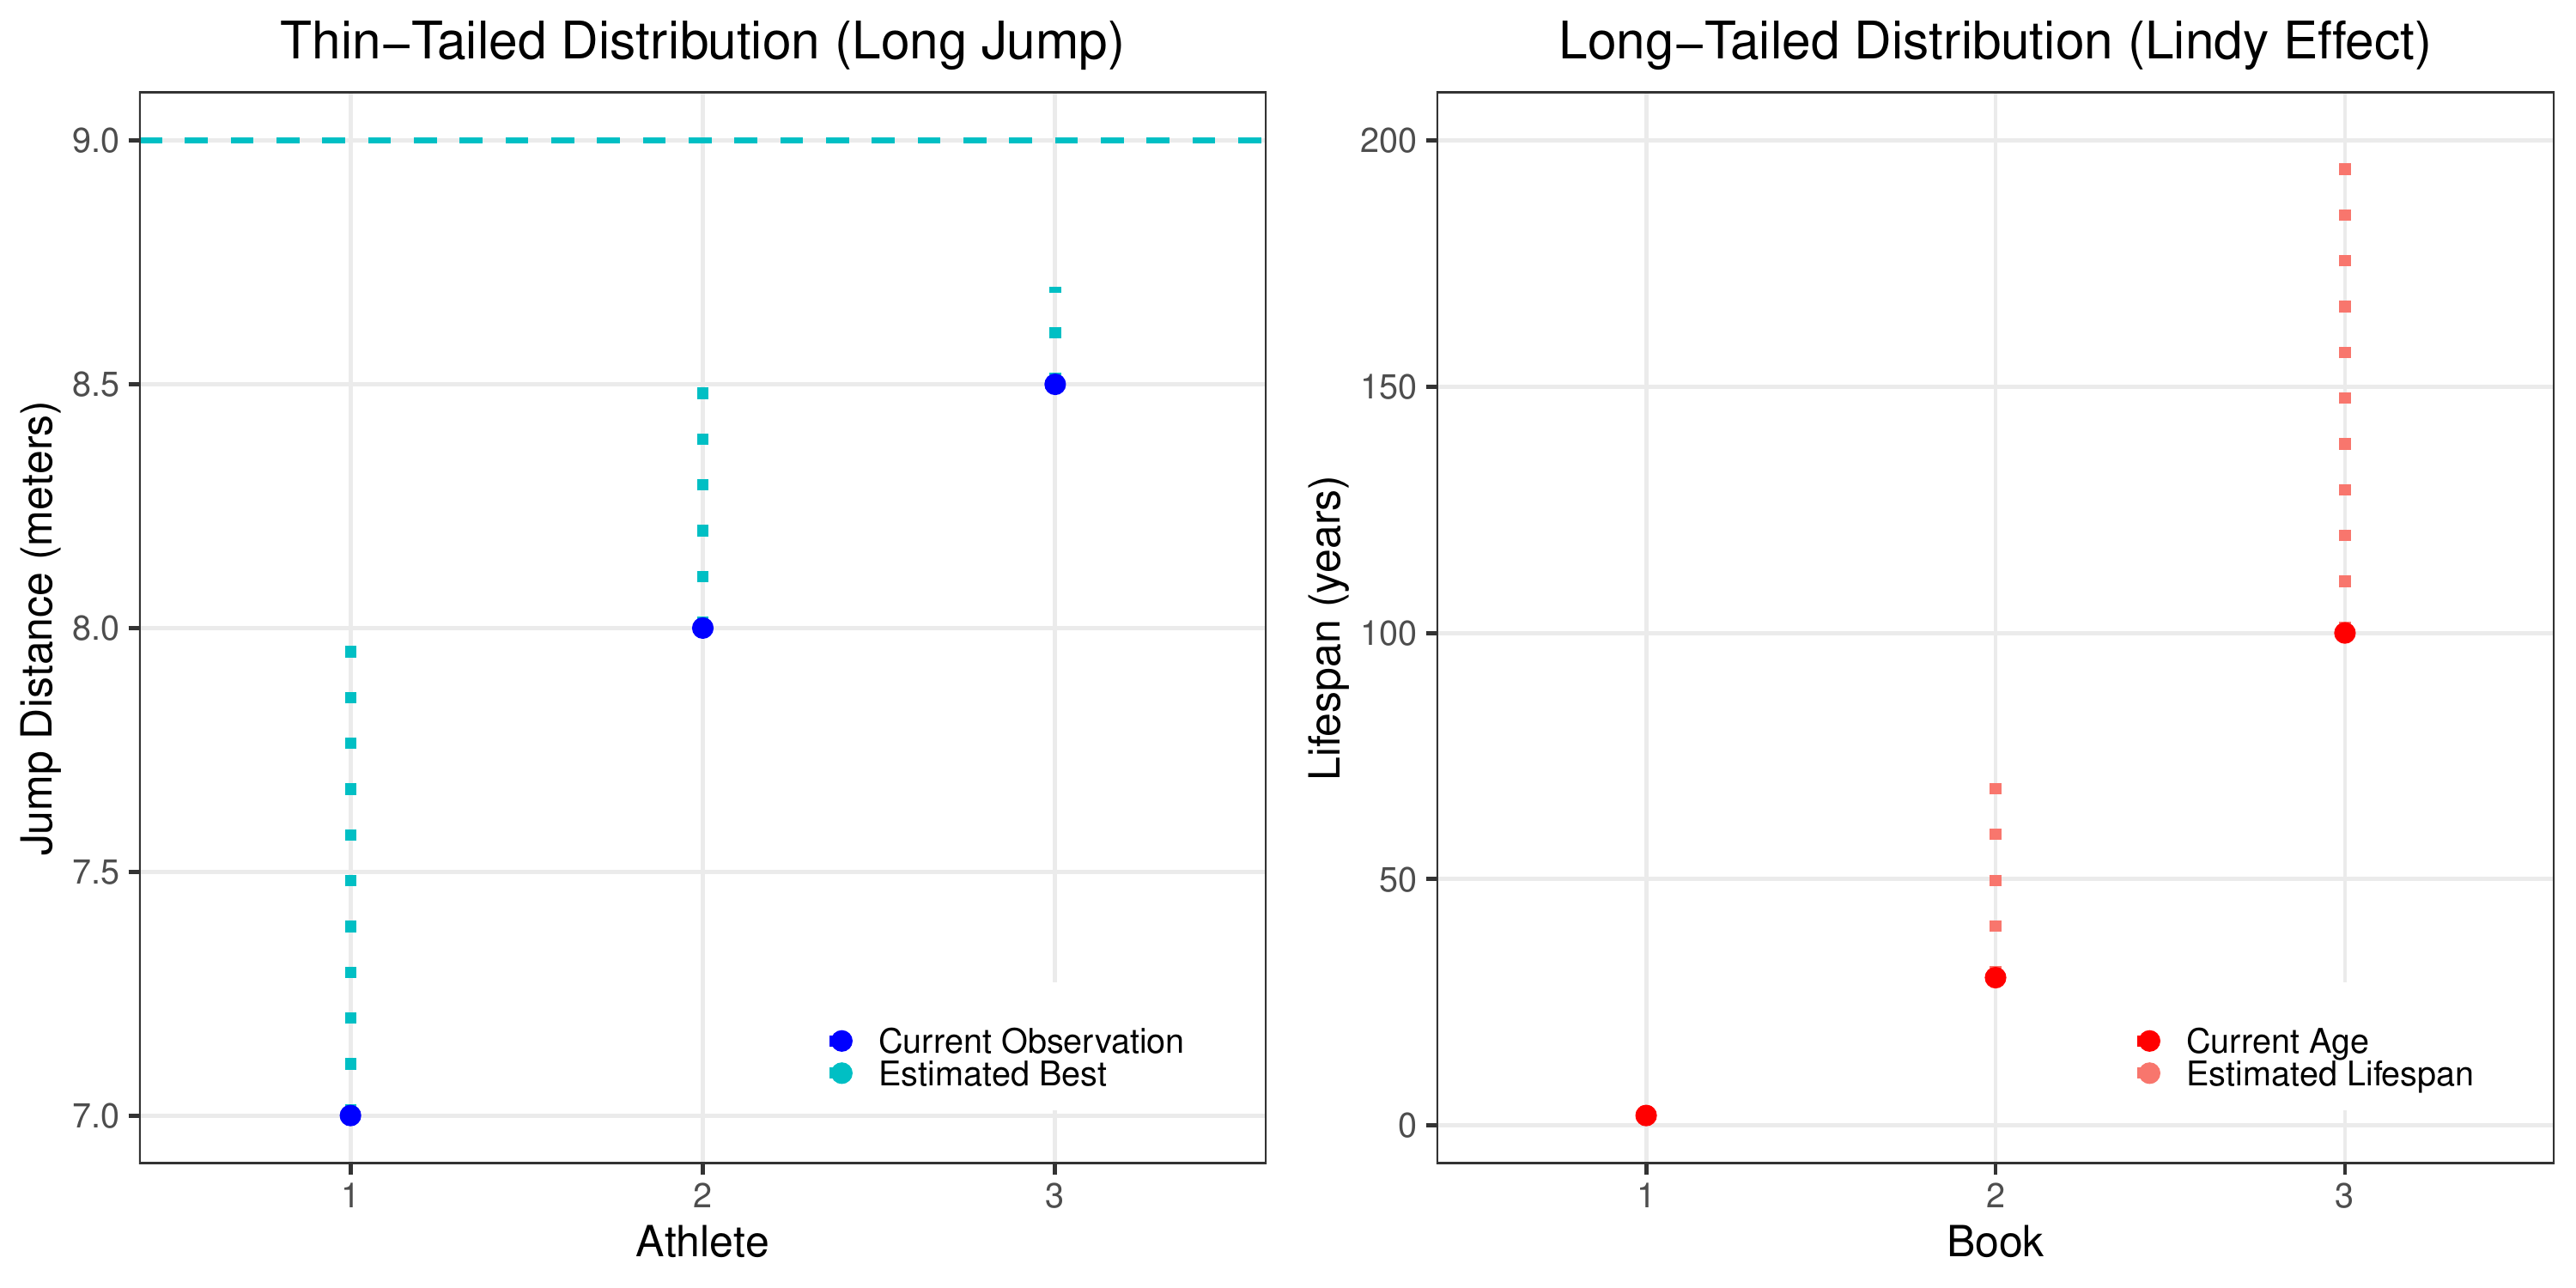}
    \caption{Our excess conditional expectation when observing long jumps (thin-tailed) shrinks as the jump gets better. By contrast, our excess conditional expectation when observing the lifespan of a book (long-tailed) gets larger as the book remains popular for longer.}
    \label{fig:excess}
\end{figure}

\paragraph{Example: Lindy Effect, Long Tails.} The Lindy Effect is the theory that, for certain types of entities, such as technologies and ideas, the longer they have been around, the longer we can expect them to survive into the future \citep{ord2023lindy}.\\

\noindent For example, if a book has been in print for two years, then it might remain in print for another two years. However, most books do not ``stand the test of time,'' so we might not expect it to survive another 100 years. Meanwhile, if another book has already been in print for 100 years, then we might well expect it to remain so for another 100 because it has showed it is robust to the test of time; if it has already remained relevant and interesting for a long time, then it is more likely to continue to do so for a long time into the future.\\

\noindent Figure \ref{fig:excess} shows some hypothetical observations of the current ages of books as blue lines, and our estimate of what their actual lifespan will be in dotted lines. Notice how, as the known lower bound of lifespan increases, the amount of additional time we expect a book to survive also increases.

\paragraph{Under long tails, excess conditional expectation grows as values become more extreme.} Under long tails, values of individual occurrences can grow much more extreme compared to the majority. There is not usually as clear a limit on long-tailed variables as on thin-tailed variables, so there is more room for the actual value to differ from the known minimum value, even if the latter is already extreme.\\

\noindent To differentiate between thin- and long-tailed distributions, we have now explored excess conditional distribution, a measure of the difference between our expectation of real-world values and the thresholds we observe them to exceed. Next, we will consider how variables arise: multiplicatively or additively.

\paragraph{Multiplicative and additive phenomena}
One factor in determining whether a variable is likely to have a long-tailed or thin-tailed distribution is whether it arises from a multiplicative or additive phenomenon. We will now look at the differences between these two categories of phenomena and why they affect how extreme a variable can become.

\paragraph{With multiplicative phenomena, one instance can multiply rapidly, triggering a cascade.} When something is a multiplicative phenomenon, individual instances are not independent of one another. Virus infections are a classic example of this; one infection is likely to seed several more infections, each of which can go on to cause even more. Thus, a single infection can trigger a cascade, so a virus outbreak has the potential to scale up considerably. This is part of the reason why virus outbreaks have a long-tailed distribution, with pandemics representing tail events.

\paragraph{With additive phenomena, individual instances do not tend to multiply.} When something is an additive phenomenon, individual events are largely independent of one another. Broken bones are an example of this; one person falling and breaking a bone does not usually trigger a cascade of other people falling and breaking bones. There may be instances where multiple broken bones occur together, for example in a car accident. However, in general, they are independently caused and do not have the potential to scale up as an infectious disease can. This means that tail events do not generally happen with this phenomenon; there is no single event where so many bones are broken that it significantly affects the average number of bones broken in accidents.

\paragraph{A high level of connectedness in a system gives rise to long tails.} Another way of thinking about this is to consider the level of connectedness in the relevant system. Since viruses are infectious, instances of infection are strongly connected to one another. Broken bones are not infectious, so instances of them are relatively isolated from one another. \\

\noindent We have seen that multiplicative phenomena are much more likely to result in long-tailed variables than additive ones. Next, we discuss another model which gives rise to long tails: preferential attachment.

\subsubsubsection{Preferential attachment}
\noindent \textbf{In preferential attachment processes, the more someone has, the more they will receive.} Preferential attachment processes are mechanisms where the amount extra of something that an individual will receive is positively correlated with the amount they already have. This is also known as the ``rich get richer'' effect because it is often illustrated with the example of wealth distribution; the more money a person already has, the more money they can invest, and thus the more additional money they can make through returns on their investments.

\noindent This effect applies to many phenomena within social systems. For example, if an author already has a lot of readers, there are more people who are likely to recommend their books to others. This author is therefore likely to gain more additional readers than someone else who starts out with fewer readers. Their sales can therefore snowball and become a tail event in the context of book sales. Similar mechanisms can also explain why a few social media platforms vastly outperform others, and why a few scientific papers receive many more citations than most.

\paragraph{Preferential attachment processes give rise to long tails \citep{Marsden2017}.} In situations where preferential attachment processes take place, events are not independent of one another. This is why things like book sales and wealth acquisition are multiplicative phenomena, where a single event can escalate to become much larger than most. By extension, this is why preferential attachment processes can produce long-tailed distributions.
    \section{Evolutionary Game Theory}\label{sec:GTappendix}
In the main text, we began our discussion of game theory by exploring the Prisoner's Dilemma, a simple game that involves two agents who interact only once. To model real-world multi-agent dynamics more closely, we first built on this by iterating the two agents' interactions. We next introduced more than two agents into the game. \\

\noindent Here, we introduce a third elaboration: the ability for agents to adapt their strategies. We look at how the multi-agent dynamics we have explored so far change when the agents concerned can adapt their behaviors.  \\

\noindent This section uses ideas from \textit{Evolutionary Game Theory}. This field was born from a merging of economics and biology in the 1970s when John Maynard-Smith and George Price found a way to describe living organisms' traits and behaviors as game strategies. Using evolutionary game theory, we explore how evolutionary forces alter the multi-agent dynamics in the Iterated Prisoner's Dilemma. In particular, we look at the conditions under which a population may cycle through different strategy compositions. We then move to a different game, known as the ``Hawk-Dove game,'' to illustrate how identical agents may tend towards Nash equilibria in which they use a range of different strategies. \\

\noindent We use these games to understand why predicting the behavior of many different AI agents may be very difficult. AI agents may evolve to employ extremely harmful strategies in repeated social interactions, including trying to extort or deceive others.By enhancing our understanding of these factors, we may better anticipate how to address potential risks stemming from multi-AI agent interactions.

\subsection{Evolutionary Iterated Prisoner's Dilemma Tournaments}\label{sec:dilemma-tournaments}
\noindent In this section, we investigate how evolutionary forces change the dynamics of a population of agents engaged in pairwise interactions. We explore how these forces can prevent a population from reaching a stable equilibrium at all. We see why, if AI agents are subject to evolutionary pressures, they may change how they interact with others in ways that are difficult to predict.

\paragraph{Evolutionary tournaments: agents can adapt their strategies.} Following his first round of Iterated Prisoner Dilemma tournaments, Axelrod later ran a second set which he re-structured to resemble the dynamics of natural selection \cite{axelrod1981evolution}. We define these ``evolutionary tournaments'' as ones where a strategy's success in one round determined the number of agents who used that strategy in the next round. The most numerous strategy at the end was the winner. Though strategies that have been successful in previous tournaments, such as \textit{tit-for-tat}, were often still successful in evolutionary tournaments, their victory was by no means assured. The outcomes of these new tournaments were very sensitive to changes in conditions, which we explore next. 

\paragraph{Cyclical dynamics can emerge; uncooperative strategies can persist.} An interesting aspect of evolutionary tournaments is that they test how well a strategy performs against itself. As the success of a particular strategy increases, so does its relative frequency in the population. Thus, agents using this strategy will play against each other more often. In this context, strategies like \textit{tit-for-tat} are vulnerable to what we call the ``echo'' problem \citep{nowak1992titfortat}. Consider a match between two agents both playing \textit{tit-for-tat}. If one defects---either by accident, or by design if they are a less cooperative \textit{tit-for-tat} variant---the other will retaliate by defecting as well. This will repeat, triggering a sequence of mutual defections. Both agents are thus locked into playing \textit{always defect}. This gives them a lower score than if one were to forgive the other, allowing them to return to a state of cooperation. Thus, more ``forgiving'' strategies can fare better in a population with a high frequency of agents playing \textit{tit-for-tat} by cutting short any string of mutual defections. This phenomenon is related to ``frequency dependent selection,'' which we explore later in this chapter. More forgiving strategies include \textit{generous tit-for-tat}, which occasionally overlooks partner defection.\\

\noindent In an evolutionary tournament, agents can switch to more successful strategies. So, if the strategy generous \textit{tit-for-tat} is more successful than ``normal'' \textit{tit-for-tat}, it may eventually become more frequent than \textit{tit-for-tat} in the population \citep{Nowak2006FiveRF}. However, if generous \textit{tit-for-tat} becomes a sufficiently common strategy in turn, agents playing \textit{always cooperate} can achieve just as high a score, making this strategy popular too. If \textit{always cooperate} reaches a sufficient frequency in the population, this creates an opportunity to exploit all these cooperators by switching to an uncooperative strategy such as \textit{always defect}. If enough agents take this opportunity and switch to playing \textit{always defect}, other agents who play \textit{tit-for-tat} will once again start to outcompete these defectors (as outlined previously). Thus, a cycle can ensue, in which each strategy is replaced by another; see Figure \ref{fig:cycle}. Many other examples of cyclical dynamics have been identified in Iterated Prisoner's Dilemma tournaments \citep{garcia2018strategy}.\\

\begin{figure}[H]
    \centering
    \includegraphics[width=0.5\linewidth]{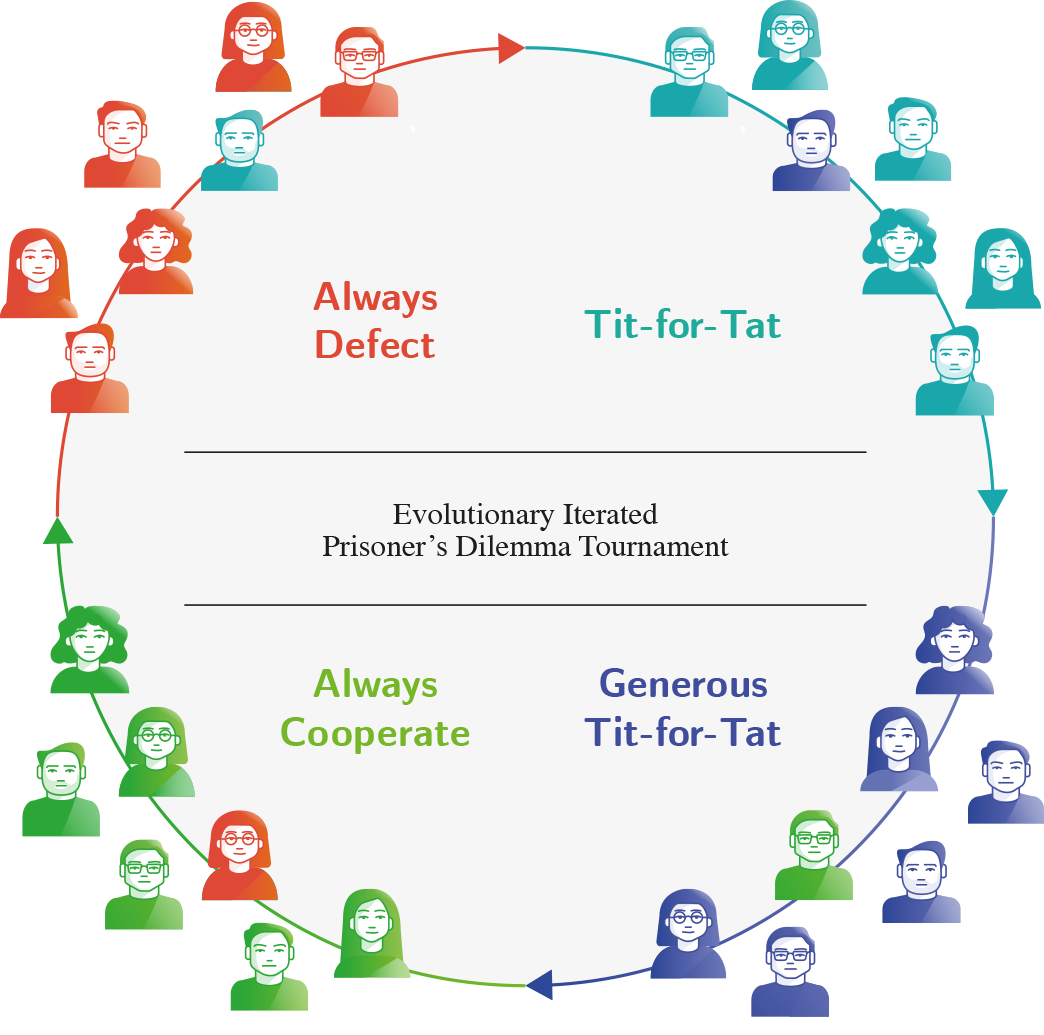}    
    \caption{In an evolutionary tournament, the prevalence of current strategies determines which new strategies do best. In the bottom left, the prevalence of ``always cooperate'' means ``always defect'' is successful. In the top left, the prevalence of ``always defect`` means ``tit-for-tat'' is successful. These dynamics can become cyclical.}
    \label{fig:cycle}
\end{figure}

\paragraph{Example: extortion strategies.} Extortion strategies can perform particularly well in evolutionary tournaments \citep{hilbe2013evolution}. This is especially true in tournaments with more detailed replications of evolutionary dynamics. For instance, in some evolutionary tournaments, agents can produce offspring who inherit both their strategy and score. With the addition of noise, in the form of random mutations, extortionists enjoy great success in this context. In even more sophisticated models that replicate coevolutionary arms races, they are yet more successful. Moreover, simulating a dramatic environmental change in these models often produces an opportunity for exceptionally profitable extortion tactics.

\subsection{Evolutionarily Stable Strategies and Frequency-Dependent Selection}\label{sec:evolutionary-stable-strategies}
In this section, we investigate how different strategies may come to replace one another within an evolving population. We start with the classic evolutionary game theoretic model known as the ``Hawk-Dove game'' to demonstrate how identical agents may reach a Nash equilibrium in which they employ different strategies to one another. This suggests that if AI agents are subject to evolutionary forces, it may be difficult to predict their behavior, because the incentives facing each may depend on what others in the population are doing.

\paragraph{Example: the Hawk-Dove game.} Let us consider a simple evolutionary game-theoretic scenario. A group of agents is engaged in frequent, pairwise contests over an indivisible resource (such as nesting space). Each agent can choose one of two strategies. \textit{``Hawks''} always fight for the prize and only back down when injured. \textit{``Doves''} only threaten but never actually fight. We call this the `Hawk-Dove' game \citep{Smith1982EvolutionAT}.\\

\noindent In a one-on-one game, a \textit{Hawk} will always beat a \textit{Dove} without any cost. When two agents choose the same strategy, each has a 50\% chance of winning or losing. But there is a difference in outcomes. The loser of a \textit{Dove-Dove} contest suffers no injury costs. Whereas the loser of a \textit{Hawk-Hawk} contest not only fails to gain the valuable resource but also incurs an injury cost from fighting. We show these two strategies' average losses and gains in the payoff matrix below (where b is the benefit of winning the resource, and c is the cost incurred by fighting). We assume that b<c, all \textit{Hawks} have equal fighting ability, and all \textit{Doves} have equal threatening ability.\\

\begin{table}[H]
    \centering
    \begin{tabular}{c|c c}
         & Hawk \textbf{(opponent)} & Dove (\textbf{Opponent}) \\
         \hline
        Hawk \textbf{(self)} & $\frac{1}{2}(b-c)$ & $b$  \\
        Dove \textbf{(self)} & 0 & $\frac{1}{2}b$ \\
    \end{tabular}
    \label{tab:hawk-dove}
    \caption{Payoff matrix for the Hawk-Dove game.}
\end{table}

\paragraph{Neither \textit{Hawk} nor \textit{Dove} is the dominant strategy.} If all agents were Hawks, everyone would fight each other for the resource and only stop when hurt. Their average gain would be $\frac{1}{2}(b-c)$. But since the price of fighting is more than the resource's value $(b<c)$, this payoff would be negative. If one agent switched to being a \textit{Dove}, they would avoid the cost of fighting, but they would never win the resource. Their average payoff would be $0$, which is better than the payoffs the \textit{Hawks} would be getting. Also, this gain would increase as more agents choose Dove, as their average payoff when meeting \textit{Doves} would be $\frac{1}{2}b$. Therefore, \textit{Doves} could \textit{invade} a \textit{Hawk}-only group.\\

\noindent Similarly, if all agents were \textit{Doves}, an agent who switched to \textit{Hawk} would gain more without paying a price for fighting, as \textit{Doves} don't fight back. So, \textit{Hawks} could invade a \textit{Dove}-only group. Hence, neither strategy is always better. The best strategy for an agent depends on what strategies the other agents are using. So the population strategy composition will include both \textit{Doves} and \textit{Hawks}.

\paragraph{Evolutionarily stable strategies.} When the members of an evolving population adopt a strategy that makes it uninvadable by any rare novel mutants that may arise, we call this state an \textit{evolutionarily stable strategy (ESS)} \citep{Smith1982EvolutionAT}. An ESS is a kind of Nash Equilibrium: when agents are at this equilibrium, they cannot improve their success by switching to any other strategy. In the Nash equilibria we have considered so far in this chapter, the agents have tended to use the same strategy as one another---if an agent used a different strategy, they would gain a lower payoff. However, a population can sometimes stably contain more than one strategy. Agents can use different strategies that are equally successful. For example, in the Hawk-Dove game, where fighting is more costly than the prize $(b<c)$, the population will reach a stable equilibrium in which there are both \textit{Hawks} and \textit{Doves}.

\paragraph{Frequency-dependent selection.} This kind of equilibrium, where agents use different strategies, is stabilized by the success of either strategy decreasing as it becomes more common, and increasing as it becomes rarer. When the success of a strategy depends on how common it is compared to others, we call this \textit{frequency-dependent selection}. A strategy may succeed more as it becomes more common. For example, if more wasps evolve bright colors to warn predators, the warning works better. Alternatively, a strategy's success might drop as it becomes more common. For example, certain snails have evolved to look like inedible objects. Frequency-dependent selection has caused them to look very different from one another. The more often a camouflage strategy is used, the more chances predators have to see through it. As a result, snails that ``choose'' (evolve) less popular camouflage strategies do the best. This results in a dynamic state in which the no snail color spreads to fixation in the population. Instead, snails of multiple colors coexist stably; see Figure \ref{fig:freq-selection}. \\

\noindent The evolutionary biologist Richard Dawkins explains this using the following fictional scenario \citep{dawkins2015evolutionarily}. A population of seagulls lives on the coast where their only source of food is the fish in the sea. Each seagull can choose whether to behave as a ``\textit{fisher}'' or as a ``\textit{pirate}''. \textit{Fishers} catch fish themselves; \textit{pirates} wait for \textit{fishers} to catch a fish, then steal it from them. Neither of these is an ESS. In a population composed entirely of fishers, a seagull who mutates and becomes a \textit{pirate} will benefit hugely; piracy is a profitable strategy because \textit{pirates} do not expend energy fishing for themselves. Thus, the \textit{pirate} strategy can invade the \textit{fisher} strategy. On the other hand, a population composed entirely of \textit{pirates} is invadable by a \textit{fisher}. Without any fishers to prey on, the \textit{pirates} have no fish to eat. A seagull who mutates and becomes a \textit{fisher} can access food for themself, giving them an advantage. Thus, neither strategy is an ESS by itself. Some proportion of the population opt for one strategy, and another proportion opts for the other. Thus, this process of frequency-dependent selection can produce populations that stably contain more than two strategies.\\

\begin{figure}[H]
    \centering
    \includegraphics[width=0.9\linewidth]{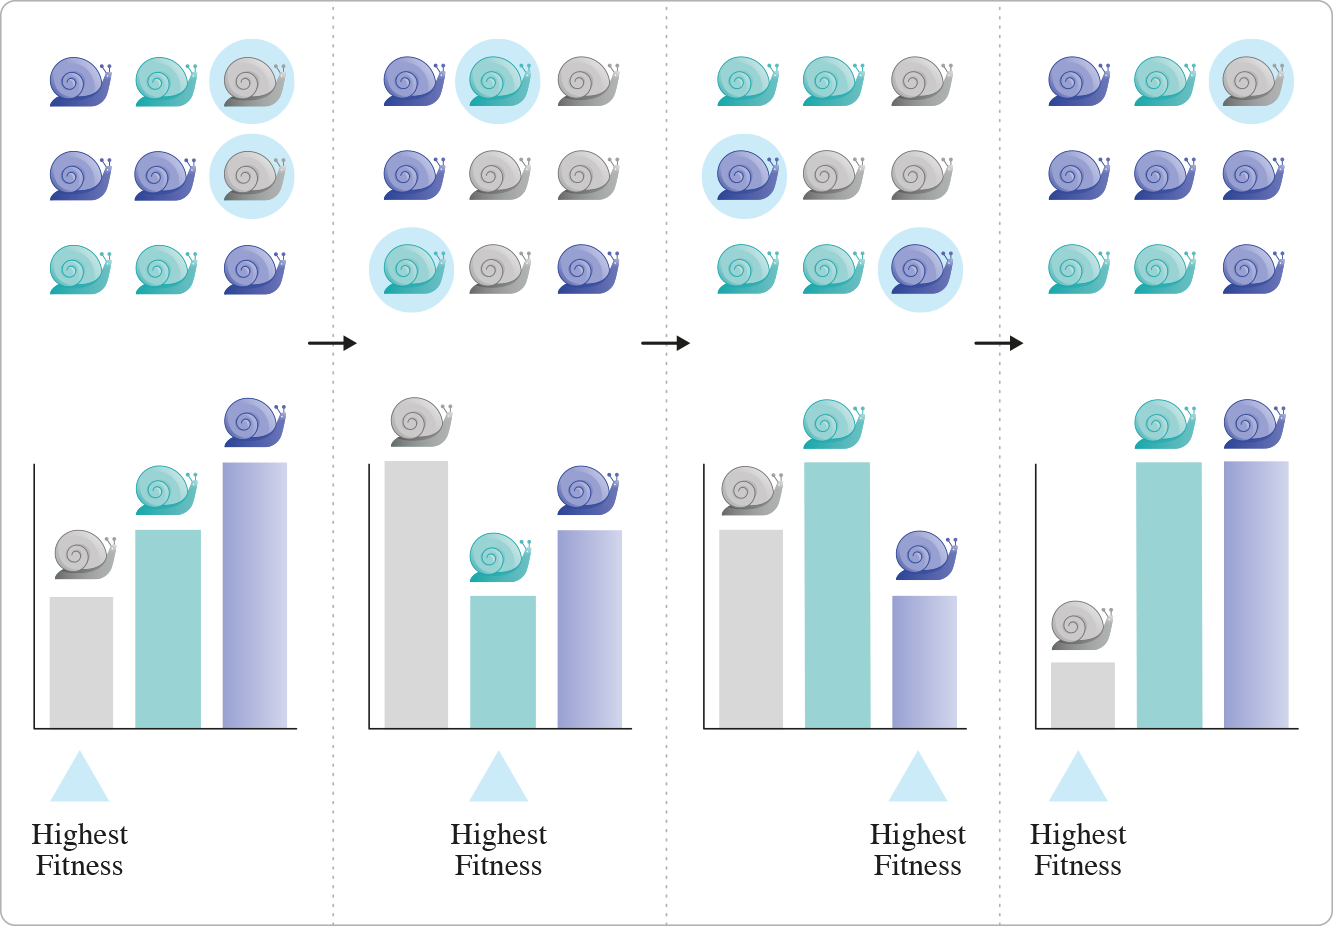}
    \caption{The rarest snails may have the highest fitness since predators are not used to them. They become more prevalent in the next generation, reducing their relative fitness. This is an example of frequency-dependent selection.}
    \label{fig:freq-selection}
\end{figure}

\noindent In each population, snails “choose to” evolve one of three colors
as camouflage: grey, teal, or blue. The frequency graph shows the
proportion of snails of each color. The black arrows indicate the
passage of time. The most successful color is indicated both by a gray
border and a gray arrow. Whichever color is rarest in one iteration
bestows the highest fitness, as predators are least used to spotting
snails of that color. Thus, more snails use this color in the following
generation. In this way, the population cycles through different color
compositions.

\paragraph{Frequency-dependent selection in game theory.} We have encountered frequency-dependent selection already in this section. In Section \ref{sec:formalization}, we briefly discussed how the ratio of contributors to free-riders in the population can alter the incentives for the agents engaged in a collective action problem. In Section \ref{sec:dilemma-tournaments}, we used evolutionary Iterated Prisoner's Dilemma tournaments to model the dynamics of natural selection, and found that there may be no stable equilibrium state. Instead, the best strategy for an agent to employ may depend on what others in the population are doing. In these cases, the population may cycle or undulate through different strategy compositions. Whichever strategy is most common may become less successful than a rarer alternative. 

\paragraph{Identical AI agents may tend towards different strategies.} A Nash equilibrium, or ESS, doesn't always mean that all agents will use the same strategy. Frequency-dependent selection might cause AI agents to adopt different but equally successful strategies. Under certain conditions, like the size and variety of a population, harmful strategies like \textit{extortion} can persist by stably cycling through different proportions of agents as the population evolves.

\paragraph{Evolutionarily stable strategies can be Pareto inefficient.} Note that in the Hawk-Dove game, all agents would be better off if they were \textit{Doves}, as every agent that plays \textit{Hawk} lowers the average payoff for them all. Just as with the Prisoner's Dilemma, the Nash equilibrium is Pareto inefficient. Hence, the ESS is not necessarily ‘good' for the population, and what is good for the population is not necessarily evolutionary stable. \textit{A population of altruistic AIs, for example, is not evolutionarily stable}, as that population is easily invadable; we explore this point in greater detail in ``Evolutionary Pressures - Section 3.3.'' This makes it likely that evolution is incompatible with achieving ideal outcomes.

\subsection{Concealment of Information}
Honesty is sometimes the best policy in an evolutionary game, but not always. Evolutionary equilibria may arise in which individual organisms use a mix of deceptive tactics to maximize their fitness. In other words, an ESS can entail the concealment of information. This section examines how evolutionary dynamics may pressure AI agents to evolve deceptive behaviors in contexts where these are more evolutionarily stable than honesty. Note that we examine other risks of deceptive AI in the \nameref{chap:single-agent-safety} chapter.

\paragraph{Concealment of information can be an ESS.} In an evolutionary setting, a certain frequency or degree of dishonest communication can be selected for \citep{hamblin2009evolution}. Non-venomous king snakes closely resemble venomous coral snakes to ward off predators \citep{greene1981coral}. Cannibalistic Portia spiders pluck the webs of other spiders to mimic the vibrations of struggling prey, thus luring their victim out into the open to be killed and eaten \citep{jackson1998spider}. Several flower species mimic the appearance of certain female insects in order to better attract males for pollination \citep{schiestl2005success}. Some bacteria produce specific molecules that act as misdirection signals to other competing bacteria, which reduce the probability of attack and detection, allowing the bacteria to maintain its competitive advantage \citep{mokkonen2015evolutionary}. Evolutionarily stable dishonesty is common in the natural world.

\paragraph{Natural selection may favor AIs that conceal information.} Consider the following scenario: a game of Poker. Agents will be better off if they have a very good ‘poker face' because other agents will not be able to deduce tell-tale signs associated with bluffing or a good hand. The incentive to have a good ``poker face'' is not malicious: it does not seek to exploit other agents and their strategies, but rather, to maximize one's own payoff in a competitive game. We might extend this reasoning to AI. If multiple AIs operate within a competitive landscape where available resources are limited, they may be incentivized to conceal information from other AIs or humans in order to preserve a competitive advantage. In other words, an AI might develop a good ‘poker face' since revealing certain kinds of information might affect their abilities to maximize payoff. Thus, strategies involving the concealment of information could be favored by natural selection among AIs, giving rise to immoral behaviors that emerge from amoral (morally neutral) grounds.

\paragraph{AI agents may develop immoral behaviors from amoral conditions.} We've shown that dishonest communication can be an ESS. The effects of inter-agent engagement can incentivize behavior we view as immoral that nonetheless evolves from morally neutral circumstances.
    \section{More Cooperation Mechanisms}
\subsubsection{Individual stakes to common stakes}
\paragraph{Individual stakes to common stakes overview.} The Nobel laureate economist John Harsanyi suggested a concept like the veil of ignorance to explore how we should structure our societies. Behind the veil of ignorance, agents are unaware of their personal characteristics and roles in society. This forces them to act as impartial observers when envisioning how the group or society should interact with each other. Because agents do not know what place they will hold (e.g., whether they will get an average position in society or a different position) in the society they envision, they often act more impartially and cooperatively when constructing a group or society. When rational agents are ignorant of their future position in society---when they are forced to make decisions behind the veil of ignorance---they are more likely to make decisions that maximize collective wellbeing, enabling cooperation through the mechanism of \textit{individual stakes to common stakes} \citep{nowak2011supercooperators}.

\paragraph{Natural examples of individual stakes to common stakes.} Intragenomic conflict arises when an individual organism’s genes have differing interests with respect to their transmission to the next generation. For example, some genes may have evolved mechanisms that increase their own replication at the expense of the organism's wellbeing. The process of meiosis, however, can resolve the problem of intragenomic conflict through randomization or the creation of a ``Darwinian veil of ignorance.'' Meiosis is a process of cell division that occurs during the formation of reproductive cells in sexually reproducing organisms. Meiosis typically results in a 50-50 distribution of genetic material from both parents to offspring, fostering genetic diversity. While it would be ``better'' for any individual gene to make more copies of itself in offspring, it cannot ``know'' whether doing so will actually increase the fitness of the organism, allowing it to pass on its genes to subsequent generations. However, by fostering genetic diversity, the process of meiosis opens the door to randomized success, allowing the forces of natural selection to impartially dictate which genes and their respective traits propagate \citep{okasha2012social}.

\paragraph{Individual stakes to common stakes in human society.} The ``Hutterites'' are a religious group known for their cooperative and communal lifestyle \citep{Harsanyi1955CardinalWI, Dennett1995DarwinsDI}. They represent a prime example of how the mechanism of individual stakes to common stakes can be used to promote cooperation. Within their communities, the Hutterites distribute all resources among themselves, and relinquish any personal wealth or possessions. This allows the Hutterites to live under a collective identity, where focus on the common good often overrides individual interests. As another example, when their group gets too large, Hutterites set up another place for people to live, and once it is finished, they randomly select members from their community to go live there. Alternatively, consider a scenario in which a group of people must row to shore. The ship does not have enough food for everyone, so the group will have to throw some rowers overboard at the halfway point to ensure the rest of the group’s survival. However, no one in the group knows that they may be thrown overboard, but they do know that to make it to shore, they must all row now. If people knew that they would be thrown overboard at some point, they would be far less likely to row. 

\paragraph{Individual stakes to common stakes and AIs.} People might perceive advanced future AIs as an outgroup threat, and this may motivate humans to cooperate against AIs. As AI’s become more widespread and powerful, they may begin to threaten human values at the global scale, motivating nations---for instance, the US and China---to set aside their differences and come together to address a common threat. If AI is someday viewed by humanity as an ``invasive species,'' it may promote global solidarity.

\subsubsection{Simon’s Selection Mechanism}
\paragraph{Simon’s selection mechanism overview.} Humans and other animals typically do not have access to all available information, time, and cognitive abilities required to make the best possible decision. Individuals are restricted by their ``bounded rationality.'' To overcome their bounded rationality and arrive at better solutions, people and organisms can benefit, on average, from relying on and receiving information through cooperative social channels. Individuals that take advantage of cooperative social channels have an increased ability to acquire socially transmitted skills and conform to socially established norms, thereby incurring a fitness advantage over those that do not participate in such channels. Moreover, when individuals choose to contribute to cooperative social channels, the information they provide can be freely utilized by anyone who participates in the system. If this information is widely used and benefits the entire social structure, social norms may emerge that compel others participating in the cooperative social channel to conform their behavior appropriately. In other words, when individuals participate in cooperative social channels, they may benefit from the collective intelligence they provide, but they may also face a cost from the group which can influence their behaviors through norms or rules. This idea was pioneered by the political scientist and Nobel laureate, Herbert Simon, and we refer to it as \textbf{Simon’s selection mechanism} \citep{simon1990mechanism}.

\paragraph{Simon’s selection mechanism in human society.} Humans have a tendency to believe in facts and propositions that they have not had the opportunity to independently verify. Such knowledge is typically disseminated through established cooperative social channels, such as the internet or culture. For instance, many people believe that consuming too much of certain kinds of cholesterol is bad for one’s health, or that touching a hot stove should always be avoided. People generally agree upon these beliefs not because they are skilled medical literature reviewers or seasoned chefs, but because such beliefs have become socially transmitted common knowledge. In general, people are better off being a part of society, rather than isolating themselves from it. Societal isolation may prevent individuals from accessing critical information that is disseminated through social channels. For instance, a hermit living in the woods with no internet access might be unaware that there is steadily expanding forest fire in the vicinity.

\paragraph{Simon’s selection mechanism and free riding.} One drawback of Simon’s selection mechanism is that it may enable free riding. Individuals may benefit from the information contained in cooperative social channels without themselves contributing to it. Consider the open-source knowledge base, Wikipedia, in this respect. Though anyone can, in theory, contribute to Wikipedia, few people actually do, because doing so can require extensive time and effort. This can result in a knowledge base that has much outdated content.

\paragraph{Simon’s selection mechanism and AIs.} In a multi-agent setting, AIs may be interacting with one another directly. They may create new communication channels and protocols among themselves, and from their interactions, norms and information channels may emerge. Such dynamics can give rise to very complex social systems from which AIs are more able to benefit than humans are. In other words, AIs may incur fitness advantages over humans by developing and participating in their own cooperative social channels, which themselves may preclude human understanding. Moreover, such cooperative social channels may evolve into AI collective intelligences, just as the internet now represents a form of human collective intelligence. However, within these collective intelligences, AIs could maintain large numbers of complex relationships with other AIs simultaneously, arriving at potentially new forms of self-organization that increase AIs ability to achieve their goals. AI collective intelligences would be vastly superior to human collective intelligences, and as a consequence, humans may be prevented from participating in and understanding the decisions AIs make within such systems.
    \section{Intrasystem Conflict Causes}
\subsection{Modularization}

\paragraph{Intrasystem goal conflict can arise through modularization.} There are two mechanisms by which intrasystem goal conflict may arise. The first is \textit{modularization}: a goal may be broken down into components, each of which thus becomes a sub-goal. For example, consider a multi-agent system, such as a committee, which wishes to carry out a complicated big-picture goal. In this case, they may break their goal up into subgoals, and delegate each of these to ``working groups'' (different subsets of the committee). Each working group now pursues solely its delegated sub-goal and the different working groups compete with one another. Ultimately, this modularity enables the different working groups to grow and change independently of one another, and can result in an uneven balance between the different sub-goals. Thus, the big-picture goal is distorted.\\

\noindent It is worth noting that some cases may differ from this story in terms of their causality. Rather than a single complex goal being modularized, sometimes individual agents may come together to form a coalition to pursue a larger-scale goal. Misalignments of interests between these agents can give rise to intrasystem goal conflict in these cases just as with modularized systemic goals. Examples include gut bacterial opportunistic pathogenicity, and some inter-sexual and intragenomic conflict. For instance, intersexual conflict in animals has produced species in which the males deliberately cause the females physical damage when mating. This strategic harming hinders the female’s ability to re-mate in future, and incentivizes her to allocate more resources towards raising that particular male’s genetic offspring. Females have in turn evolved defensive strategies against this, such as armor plating and spines \citep{morrow2003traumatic}. Intersexual coevolutionary ``arms races'' such as these have been documented in a diverse range of species, from ducks to fruit flies \citep{rowe2002sexually}. Rather than a unified goal being modularized, the goal conflict here has arisen in the context of a coalition. The female and male are collaborating through sexual reproduction, but even slight misalignments of their interests can result in dramatic goal conflict.

\subsection{Delegation}
\paragraph{Intrasystem goal conflict can arise through delegation.} The second mechanism by which intrasystem goal conflict may arise is in the \textit{delegation} itself. In the above example, the working groups each pursue their assigned sub-goal faithfully. The problem is that the collective outcome of these agencies, each optimizing for their assigned subgoal is a distorted version of the original big-picture goal. However, the delegation of a goal to another agent can also itself generate intrasystem goal conflict. \\

\noindent In economics, this is called \textbf{a principal-agent problem}. Put simply, this is the problem of conflicting priorities that arises when one party (the \textit{principal}) delegates a goal of theirs to another (the \textit{agent}), who is not entirely value-aligned with the \textit{principal}. The \textit{agent} has other interests, such as self-preservation or gain of influence, which compete with the goal the \textit{principal} has delegated to them. This can result in the distortion or subversion of the delegated goal: the agent pursues their own goals as well as (or instead of) that of the principal. Principal-agent problems are most common where there is a knowledge asymmetry, such that the agent knows more about the relevant matter than the principal. For example, consider a client who has hired a mechanic to fix their car. The client wishes their car to be fixed as cost-effectively as possible; the mechanic wishes to maximize their profits. The principal-agent problem is thus that the client cannot trust the mechanic to report the cost of the car fix accurately. \\

\noindent Principal-agent problems can generate intrasystem goal conflict wherever the components of a modularized big-picture goal are delegated to sub-agents. In particular, the sub-agents are likely to be motivated by self-preservation. If the goal the principal has delegated to them clashes with their own goal of self-preservation, this can produce strong intrasystem goal conflict. To build on the committee example above, now consider that each working group is incentivized to compete with the others to avoid being disbanded. Each exaggerates the importance of their own work, or reconfigures their assigned objective in order to achieve goals of their own. Ultimately, some even break away from the committee, to pursue their emergent goals without the constraints imposed by the committee from which they formed.\\

\subsection{Example: the FDA vs the USDA}
\noindent Intrasystem goal conflict often arises when a system both modularizes and delegates a complex goal. For example, the US Food and Drug Administration (FDA) and the Department of Agriculture (USDA) are sub-agencies of the same government \citep{moss2010warning}. The US government delegates sub-goals to each agency to carry out, yet sometimes their interests and actions conflict with one another. In 2010, the USDA implemented a marketing campaign to promote eating more cheese, to support the dairy industry. Simultaneously, the FDA implemented a marketing campaign of their own to promote eating less cheese, as part of an effort to reduce the saturated fat content of American diets. Despite the fact that both agencies were delegated sub-goals from the same government, their conflicting objectives resulted in their taking actions that hindered one another.
\end{refsegment}
