# Supplementary material for: Introduction to AI Safety, Ethics, and Society
Source: arXiv:2411.01042 source file (2024-11-15)
Supplement: Supplementary file 2 [file 2.5_Game_theory_appendix.tex]

\section{Evolutionary Game Theory}\label{sec:GTappendix}
In the main text, we began our discussion of game theory by exploring the Prisoner's Dilemma, a simple game that involves two agents who interact only once. To model real-world multi-agent dynamics more closely, we first built on this by iterating the two agents' interactions. We next introduced more than two agents into the game. \\

\noindent Here, we introduce a third elaboration: the ability for agents to adapt their strategies. We look at how the multi-agent dynamics we have explored so far change when the agents concerned can adapt their behaviors.  \\

\noindent This section uses ideas from \textit{Evolutionary Game Theory}. This field was born from a merging of economics and biology in the 1970s when John Maynard-Smith and George Price found a way to describe living organisms' traits and behaviors as game strategies. Using evolutionary game theory, we explore how evolutionary forces alter the multi-agent dynamics in the Iterated Prisoner's Dilemma. In particular, we look at the conditions under which a population may cycle through different strategy compositions. We then move to a different game, known as the ``Hawk-Dove game,'' to illustrate how identical agents may tend towards Nash equilibria in which they use a range of different strategies. \\

\noindent We use these games to understand why predicting the behavior of many different AI agents may be very difficult. AI agents may evolve to employ extremely harmful strategies in repeated social interactions, including trying to extort or deceive others.By enhancing our understanding of these factors, we may better anticipate how to address potential risks stemming from multi-AI agent interactions.

\subsection{Evolutionary Iterated Prisoner's Dilemma Tournaments}\label{sec:dilemma-tournaments}
\noindent In this section, we investigate how evolutionary forces change the dynamics of a population of agents engaged in pairwise interactions. We explore how these forces can prevent a population from reaching a stable equilibrium at all. We see why, if AI agents are subject to evolutionary pressures, they may change how they interact with others in ways that are difficult to predict.

\paragraph{Evolutionary tournaments: agents can adapt their strategies.} Following his first round of Iterated Prisoner Dilemma tournaments, Axelrod later ran a second set which he re-structured to resemble the dynamics of natural selection \cite{axelrod1981evolution}. We define these ``evolutionary tournaments'' as ones where a strategy's success in one round determined the number of agents who used that strategy in the next round. The most numerous strategy at the end was the winner. Though strategies that have been successful in previous tournaments, such as \textit{tit-for-tat}, were often still successful in evolutionary tournaments, their victory was by no means assured. The outcomes of these new tournaments were very sensitive to changes in conditions, which we explore next. 

\paragraph{Cyclical dynamics can emerge; uncooperative strategies can persist.} An interesting aspect of evolutionary tournaments is that they test how well a strategy performs against itself. As the success of a particular strategy increases, so does its relative frequency in the population. Thus, agents using this strategy will play against each other more often. In this context, strategies like \textit{tit-for-tat} are vulnerable to what we call the ``echo'' problem \citep{nowak1992titfortat}. Consider a match between two agents both playing \textit{tit-for-tat}. If one defects---either by accident, or by design if they are a less cooperative \textit{tit-for-tat} variant---the other will retaliate by defecting as well. This will repeat, triggering a sequence of mutual defections. Both agents are thus locked into playing \textit{always defect}. This gives them a lower score than if one were to forgive the other, allowing them to return to a state of cooperation. Thus, more ``forgiving'' strategies can fare better in a population with a high frequency of agents playing \textit{tit-for-tat} by cutting short any string of mutual defections. This phenomenon is related to ``frequency dependent selection,'' which we explore later in this chapter. More forgiving strategies include \textit{generous tit-for-tat}, which occasionally overlooks partner defection.\\

\noindent In an evolutionary tournament, agents can switch to more successful strategies. So, if the strategy generous \textit{tit-for-tat} is more successful than ``normal'' \textit{tit-for-tat}, it may eventually become more frequent than \textit{tit-for-tat} in the population \citep{Nowak2006FiveRF}. However, if generous \textit{tit-for-tat} becomes a sufficiently common strategy in turn, agents playing \textit{always cooperate} can achieve just as high a score, making this strategy popular too. If \textit{always cooperate} reaches a sufficient frequency in the population, this creates an opportunity to exploit all these cooperators by switching to an uncooperative strategy such as \textit{always defect}. If enough agents take this opportunity and switch to playing \textit{always defect}, other agents who play \textit{tit-for-tat} will once again start to outcompete these defectors (as outlined previously). Thus, a cycle can ensue, in which each strategy is replaced by another; see Figure \ref{fig:cycle}. Many other examples of cyclical dynamics have been identified in Iterated Prisoner's Dilemma tournaments \citep{garcia2018strategy}.\\

\begin{figure}[H]
    \centering
    \includegraphics[width=0.5\linewidth]{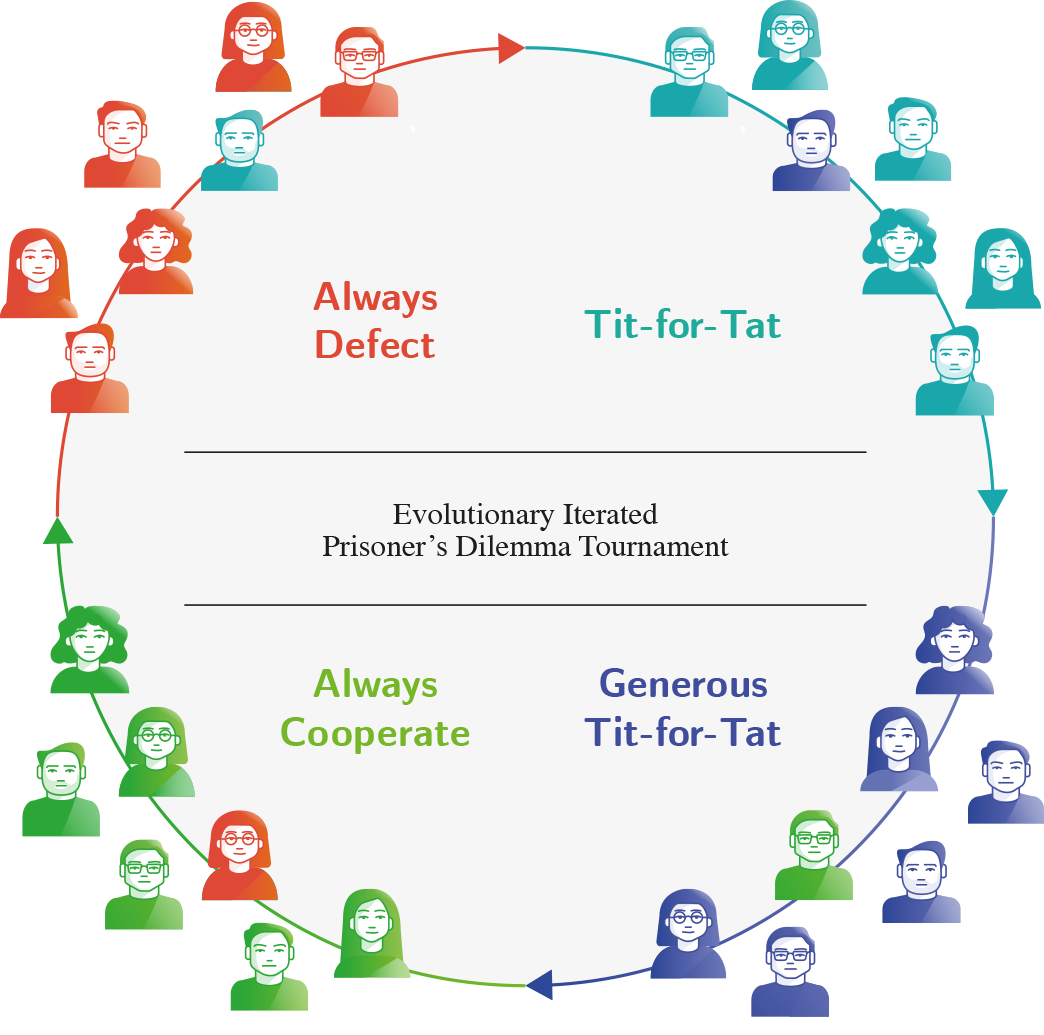}    
    \caption{In an evolutionary tournament, the prevalence of current strategies determines which new strategies do best. In the bottom left, the prevalence of ``always cooperate'' means ``always defect'' is successful. In the top left, the prevalence of ``always defect`` means ``tit-for-tat'' is successful. These dynamics can become cyclical.}
    \label{fig:cycle}
\end{figure}

\paragraph{Example: extortion strategies.} Extortion strategies can perform particularly well in evolutionary tournaments \citep{hilbe2013evolution}. This is especially true in tournaments with more detailed replications of evolutionary dynamics. For instance, in some evolutionary tournaments, agents can produce offspring who inherit both their strategy and score. With the addition of noise, in the form of random mutations, extortionists enjoy great success in this context. In even more sophisticated models that replicate coevolutionary arms races, they are yet more successful. Moreover, simulating a dramatic environmental change in these models often produces an opportunity for exceptionally profitable extortion tactics.

\subsection{Evolutionarily Stable Strategies and Frequency-Dependent Selection}\label{sec:evolutionary-stable-strategies}
In this section, we investigate how different strategies may come to replace one another within an evolving population. We start with the classic evolutionary game theoretic model known as the ``Hawk-Dove game'' to demonstrate how identical agents may reach a Nash equilibrium in which they employ different strategies to one another. This suggests that if AI agents are subject to evolutionary forces, it may be difficult to predict their behavior, because the incentives facing each may depend on what others in the population are doing.

\paragraph{Example: the Hawk-Dove game.} Let us consider a simple evolutionary game-theoretic scenario. A group of agents is engaged in frequent, pairwise contests over an indivisible resource (such as nesting space). Each agent can choose one of two strategies. \textit{``Hawks''} always fight for the prize and only back down when injured. \textit{``Doves''} only threaten but never actually fight. We call this the `Hawk-Dove' game \citep{Smith1982EvolutionAT}.\\

\noindent In a one-on-one game, a \textit{Hawk} will always beat a \textit{Dove} without any cost. When two agents choose the same strategy, each has a 50\% chance of winning or losing. But there is a difference in outcomes. The loser of a \textit{Dove-Dove} contest suffers no injury costs. Whereas the loser of a \textit{Hawk-Hawk} contest not only fails to gain the valuable resource but also incurs an injury cost from fighting. We show these two strategies' average losses and gains in the payoff matrix below (where b is the benefit of winning the resource, and c is the cost incurred by fighting). We assume that b<c, all \textit{Hawks} have equal fighting ability, and all \textit{Doves} have equal threatening ability.\\

\begin{table}[H]
    \centering
    \begin{tabular}{c|c c}
         & Hawk \textbf{(opponent)} & Dove (\textbf{Opponent}) \\
         \hline
        Hawk \textbf{(self)} & $\frac{1}{2}(b-c)$ & $b$  \\
        Dove \textbf{(self)} & 0 & $\frac{1}{2}b$ \\
    \end{tabular}
    \label{tab:hawk-dove}
    \caption{Payoff matrix for the Hawk-Dove game.}
\end{table}

\paragraph{Neither \textit{Hawk} nor \textit{Dove} is the dominant strategy.} If all agents were Hawks, everyone would fight each other for the resource and only stop when hurt. Their average gain would be $\frac{1}{2}(b-c)$. But since the price of fighting is more than the resource's value $(b<c)$, this payoff would be negative. If one agent switched to being a \textit{Dove}, they would avoid the cost of fighting, but they would never win the resource. Their average payoff would be $0$, which is better than the payoffs the \textit{Hawks} would be getting. Also, this gain would increase as more agents choose Dove, as their average payoff when meeting \textit{Doves} would be $\frac{1}{2}b$. Therefore, \textit{Doves} could \textit{invade} a \textit{Hawk}-only group.\\

\noindent Similarly, if all agents were \textit{Doves}, an agent who switched to \textit{Hawk} would gain more without paying a price for fighting, as \textit{Doves} don't fight back. So, \textit{Hawks} could invade a \textit{Dove}-only group. Hence, neither strategy is always better. The best strategy for an agent depends on what strategies the other agents are using. So the population strategy composition will include both \textit{Doves} and \textit{Hawks}.

\paragraph{Evolutionarily stable strategies.} When the members of an evolving population adopt a strategy that makes it uninvadable by any rare novel mutants that may arise, we call this state an \textit{evolutionarily stable strategy (ESS)} \citep{Smith1982EvolutionAT}. An ESS is a kind of Nash Equilibrium: when agents are at this equilibrium, they cannot improve their success by switching to any other strategy. In the Nash equilibria we have considered so far in this chapter, the agents have tended to use the same strategy as one another---if an agent used a different strategy, they would gain a lower payoff. However, a population can sometimes stably contain more than one strategy. Agents can use different strategies that are equally successful. For example, in the Hawk-Dove game, where fighting is more costly than the prize $(b<c)$, the population will reach a stable equilibrium in which there are both \textit{Hawks} and \textit{Doves}.

\paragraph{Frequency-dependent selection.} This kind of equilibrium, where agents use different strategies, is stabilized by the success of either strategy decreasing as it becomes more common, and increasing as it becomes rarer. When the success of a strategy depends on how common it is compared to others, we call this \textit{frequency-dependent selection}. A strategy may succeed more as it becomes more common. For example, if more wasps evolve bright colors to warn predators, the warning works better. Alternatively, a strategy's success might drop as it becomes more common. For example, certain snails have evolved to look like inedible objects. Frequency-dependent selection has caused them to look very different from one another. The more often a camouflage strategy is used, the more chances predators have to see through it. As a result, snails that ``choose'' (evolve) less popular camouflage strategies do the best. This results in a dynamic state in which the no snail color spreads to fixation in the population. Instead, snails of multiple colors coexist stably; see Figure \ref{fig:freq-selection}. \\

\noindent The evolutionary biologist Richard Dawkins explains this using the following fictional scenario \citep{dawkins2015evolutionarily}. A population of seagulls lives on the coast where their only source of food is the fish in the sea. Each seagull can choose whether to behave as a ``\textit{fisher}'' or as a ``\textit{pirate}''. \textit{Fishers} catch fish themselves; \textit{pirates} wait for \textit{fishers} to catch a fish, then steal it from them. Neither of these is an ESS. In a population composed entirely of fishers, a seagull who mutates and becomes a \textit{pirate} will benefit hugely; piracy is a profitable strategy because \textit{pirates} do not expend energy fishing for themselves. Thus, the \textit{pirate} strategy can invade the \textit{fisher} strategy. On the other hand, a population composed entirely of \textit{pirates} is invadable by a \textit{fisher}. Without any fishers to prey on, the \textit{pirates} have no fish to eat. A seagull who mutates and becomes a \textit{fisher} can access food for themself, giving them an advantage. Thus, neither strategy is an ESS by itself. Some proportion of the population opt for one strategy, and another proportion opts for the other. Thus, this process of frequency-dependent selection can produce populations that stably contain more than two strategies.\\

\begin{figure}[H]
    \centering
    \includegraphics[width=0.9\linewidth]{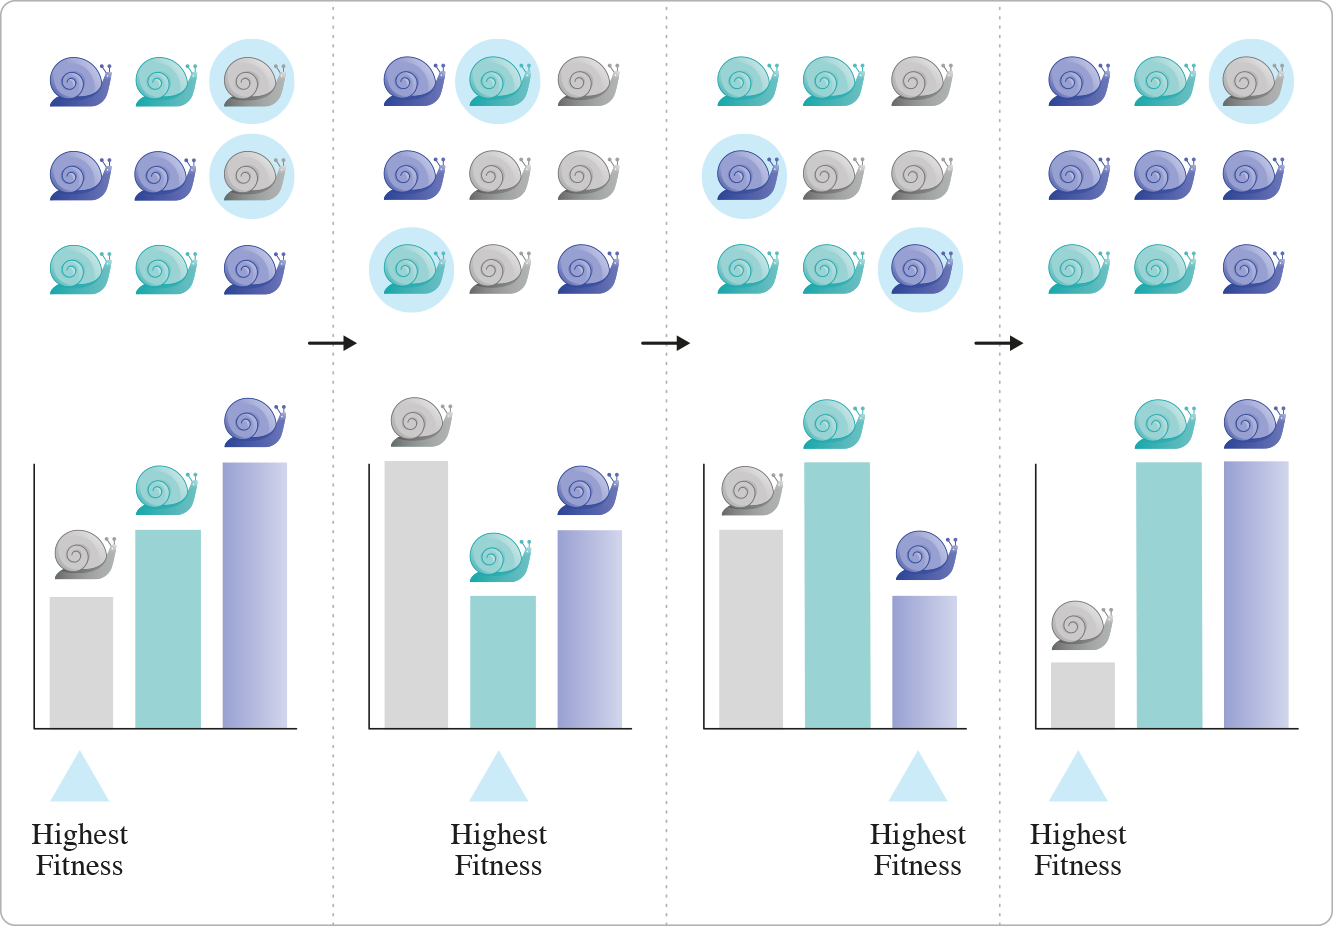}
    \caption{The rarest snails may have the highest fitness since predators are not used to them. They become more prevalent in the next generation, reducing their relative fitness. This is an example of frequency-dependent selection.}
    \label{fig:freq-selection}
\end{figure}

\noindent In each population, snails “choose to” evolve one of three colors
as camouflage: grey, teal, or blue. The frequency graph shows the
proportion of snails of each color. The black arrows indicate the
passage of time. The most successful color is indicated both by a gray
border and a gray arrow. Whichever color is rarest in one iteration
bestows the highest fitness, as predators are least used to spotting
snails of that color. Thus, more snails use this color in the following
generation. In this way, the population cycles through different color
compositions.

\paragraph{Frequency-dependent selection in game theory.} We have encountered frequency-dependent selection already in this section. In Section \ref{sec:formalization}, we briefly discussed how the ratio of contributors to free-riders in the population can alter the incentives for the agents engaged in a collective action problem. In Section \ref{sec:dilemma-tournaments}, we used evolutionary Iterated Prisoner's Dilemma tournaments to model the dynamics of natural selection, and found that there may be no stable equilibrium state. Instead, the best strategy for an agent to employ may depend on what others in the population are doing. In these cases, the population may cycle or undulate through different strategy compositions. Whichever strategy is most common may become less successful than a rarer alternative. 

\paragraph{Identical AI agents may tend towards different strategies.} A Nash equilibrium, or ESS, doesn't always mean that all agents will use the same strategy. Frequency-dependent selection might cause AI agents to adopt different but equally successful strategies. Under certain conditions, like the size and variety of a population, harmful strategies like \textit{extortion} can persist by stably cycling through different proportions of agents as the population evolves.

\paragraph{Evolutionarily stable strategies can be Pareto inefficient.} Note that in the Hawk-Dove game, all agents would be better off if they were \textit{Doves}, as every agent that plays \textit{Hawk} lowers the average payoff for them all. Just as with the Prisoner's Dilemma, the Nash equilibrium is Pareto inefficient. Hence, the ESS is not necessarily ‘good' for the population, and what is good for the population is not necessarily evolutionary stable. \textit{A population of altruistic AIs, for example, is not evolutionarily stable}, as that population is easily invadable; we explore this point in greater detail in ``Evolutionary Pressures - Section 3.3.'' This makes it likely that evolution is incompatible with achieving ideal outcomes.

\subsection{Concealment of Information}
Honesty is sometimes the best policy in an evolutionary game, but not always. Evolutionary equilibria may arise in which individual organisms use a mix of deceptive tactics to maximize their fitness. In other words, an ESS can entail the concealment of information. This section examines how evolutionary dynamics may pressure AI agents to evolve deceptive behaviors in contexts where these are more evolutionarily stable than honesty. Note that we examine other risks of deceptive AI in the \nameref{chap:single-agent-safety} chapter.

\paragraph{Concealment of information can be an ESS.} In an evolutionary setting, a certain frequency or degree of dishonest communication can be selected for \citep{hamblin2009evolution}. Non-venomous king snakes closely resemble venomous coral snakes to ward off predators \citep{greene1981coral}. Cannibalistic Portia spiders pluck the webs of other spiders to mimic the vibrations of struggling prey, thus luring their victim out into the open to be killed and eaten \citep{jackson1998spider}. Several flower species mimic the appearance of certain female insects in order to better attract males for pollination \citep{schiestl2005success}. Some bacteria produce specific molecules that act as misdirection signals to other competing bacteria, which reduce the probability of attack and detection, allowing the bacteria to maintain its competitive advantage \citep{mokkonen2015evolutionary}. Evolutionarily stable dishonesty is common in the natural world.

\paragraph{Natural selection may favor AIs that conceal information.} Consider the following scenario: a game of Poker. Agents will be better off if they have a very good ‘poker face' because other agents will not be able to deduce tell-tale signs associated with bluffing or a good hand. The incentive to have a good ``poker face'' is not malicious: it does not seek to exploit other agents and their strategies, but rather, to maximize one's own payoff in a competitive game. We might extend this reasoning to AI. If multiple AIs operate within a competitive landscape where available resources are limited, they may be incentivized to conceal information from other AIs or humans in order to preserve a competitive advantage. In other words, an AI might develop a good ‘poker face' since revealing certain kinds of information might affect their abilities to maximize payoff. Thus, strategies involving the concealment of information could be favored by natural selection among AIs, giving rise to immoral behaviors that emerge from amoral (morally neutral) grounds.

\paragraph{AI agents may develop immoral behaviors from amoral conditions.} We've shown that dishonest communication can be an ESS. The effects of inter-agent engagement can incentivize behavior we view as immoral that nonetheless evolves from morally neutral circumstances.
