# Supplementary material for: Introduction to AI Safety, Ethics, and Society
Source: arXiv:2411.01042 source file (2024-11-15)
Supplement: Supplementary file 3 [file 3.5_Cooperation_appendix.tex]

\section{More Cooperation Mechanisms}
\subsubsection{Individual stakes to common stakes}
\paragraph{Individual stakes to common stakes overview.} The Nobel laureate economist John Harsanyi suggested a concept like the veil of ignorance to explore how we should structure our societies. Behind the veil of ignorance, agents are unaware of their personal characteristics and roles in society. This forces them to act as impartial observers when envisioning how the group or society should interact with each other. Because agents do not know what place they will hold (e.g., whether they will get an average position in society or a different position) in the society they envision, they often act more impartially and cooperatively when constructing a group or society. When rational agents are ignorant of their future position in society---when they are forced to make decisions behind the veil of ignorance---they are more likely to make decisions that maximize collective wellbeing, enabling cooperation through the mechanism of \textit{individual stakes to common stakes} \citep{nowak2011supercooperators}.

\paragraph{Natural examples of individual stakes to common stakes.} Intragenomic conflict arises when an individual organism’s genes have differing interests with respect to their transmission to the next generation. For example, some genes may have evolved mechanisms that increase their own replication at the expense of the organism's wellbeing. The process of meiosis, however, can resolve the problem of intragenomic conflict through randomization or the creation of a ``Darwinian veil of ignorance.'' Meiosis is a process of cell division that occurs during the formation of reproductive cells in sexually reproducing organisms. Meiosis typically results in a 50-50 distribution of genetic material from both parents to offspring, fostering genetic diversity. While it would be ``better'' for any individual gene to make more copies of itself in offspring, it cannot ``know'' whether doing so will actually increase the fitness of the organism, allowing it to pass on its genes to subsequent generations. However, by fostering genetic diversity, the process of meiosis opens the door to randomized success, allowing the forces of natural selection to impartially dictate which genes and their respective traits propagate \citep{okasha2012social}.

\paragraph{Individual stakes to common stakes in human society.} The ``Hutterites'' are a religious group known for their cooperative and communal lifestyle \citep{Harsanyi1955CardinalWI, Dennett1995DarwinsDI}. They represent a prime example of how the mechanism of individual stakes to common stakes can be used to promote cooperation. Within their communities, the Hutterites distribute all resources among themselves, and relinquish any personal wealth or possessions. This allows the Hutterites to live under a collective identity, where focus on the common good often overrides individual interests. As another example, when their group gets too large, Hutterites set up another place for people to live, and once it is finished, they randomly select members from their community to go live there. Alternatively, consider a scenario in which a group of people must row to shore. The ship does not have enough food for everyone, so the group will have to throw some rowers overboard at the halfway point to ensure the rest of the group’s survival. However, no one in the group knows that they may be thrown overboard, but they do know that to make it to shore, they must all row now. If people knew that they would be thrown overboard at some point, they would be far less likely to row. 

\paragraph{Individual stakes to common stakes and AIs.} People might perceive advanced future AIs as an outgroup threat, and this may motivate humans to cooperate against AIs. As AI’s become more widespread and powerful, they may begin to threaten human values at the global scale, motivating nations---for instance, the US and China---to set aside their differences and come together to address a common threat. If AI is someday viewed by humanity as an ``invasive species,'' it may promote global solidarity.

\subsubsection{Simon’s Selection Mechanism}
\paragraph{Simon’s selection mechanism overview.} Humans and other animals typically do not have access to all available information, time, and cognitive abilities required to make the best possible decision. Individuals are restricted by their ``bounded rationality.'' To overcome their bounded rationality and arrive at better solutions, people and organisms can benefit, on average, from relying on and receiving information through cooperative social channels. Individuals that take advantage of cooperative social channels have an increased ability to acquire socially transmitted skills and conform to socially established norms, thereby incurring a fitness advantage over those that do not participate in such channels. Moreover, when individuals choose to contribute to cooperative social channels, the information they provide can be freely utilized by anyone who participates in the system. If this information is widely used and benefits the entire social structure, social norms may emerge that compel others participating in the cooperative social channel to conform their behavior appropriately. In other words, when individuals participate in cooperative social channels, they may benefit from the collective intelligence they provide, but they may also face a cost from the group which can influence their behaviors through norms or rules. This idea was pioneered by the political scientist and Nobel laureate, Herbert Simon, and we refer to it as \textbf{Simon’s selection mechanism} \citep{simon1990mechanism}.

\paragraph{Simon’s selection mechanism in human society.} Humans have a tendency to believe in facts and propositions that they have not had the opportunity to independently verify. Such knowledge is typically disseminated through established cooperative social channels, such as the internet or culture. For instance, many people believe that consuming too much of certain kinds of cholesterol is bad for one’s health, or that touching a hot stove should always be avoided. People generally agree upon these beliefs not because they are skilled medical literature reviewers or seasoned chefs, but because such beliefs have become socially transmitted common knowledge. In general, people are better off being a part of society, rather than isolating themselves from it. Societal isolation may prevent individuals from accessing critical information that is disseminated through social channels. For instance, a hermit living in the woods with no internet access might be unaware that there is steadily expanding forest fire in the vicinity.

\paragraph{Simon’s selection mechanism and free riding.} One drawback of Simon’s selection mechanism is that it may enable free riding. Individuals may benefit from the information contained in cooperative social channels without themselves contributing to it. Consider the open-source knowledge base, Wikipedia, in this respect. Though anyone can, in theory, contribute to Wikipedia, few people actually do, because doing so can require extensive time and effort. This can result in a knowledge base that has much outdated content.

\paragraph{Simon’s selection mechanism and AIs.} In a multi-agent setting, AIs may be interacting with one another directly. They may create new communication channels and protocols among themselves, and from their interactions, norms and information channels may emerge. Such dynamics can give rise to very complex social systems from which AIs are more able to benefit than humans are. In other words, AIs may incur fitness advantages over humans by developing and participating in their own cooperative social channels, which themselves may preclude human understanding. Moreover, such cooperative social channels may evolve into AI collective intelligences, just as the internet now represents a form of human collective intelligence. However, within these collective intelligences, AIs could maintain large numbers of complex relationships with other AIs simultaneously, arriving at potentially new forms of self-organization that increase AIs ability to achieve their goals. AI collective intelligences would be vastly superior to human collective intelligences, and as a consequence, humans may be prevented from participating in and understanding the decisions AIs make within such systems.
