# Supplementary material for: Introduction to AI Safety, Ethics, and Society
Source: arXiv:2411.01042 source file (2024-11-15)
Supplement: Supplementary file 4 [file 5.5_Evolutionary_pressures_appendix.tex]

\section{Intrasystem Conflict Causes}
\subsection{Modularization}

\paragraph{Intrasystem goal conflict can arise through modularization.} There are two mechanisms by which intrasystem goal conflict may arise. The first is \textit{modularization}: a goal may be broken down into components, each of which thus becomes a sub-goal. For example, consider a multi-agent system, such as a committee, which wishes to carry out a complicated big-picture goal. In this case, they may break their goal up into subgoals, and delegate each of these to ``working groups'' (different subsets of the committee). Each working group now pursues solely its delegated sub-goal and the different working groups compete with one another. Ultimately, this modularity enables the different working groups to grow and change independently of one another, and can result in an uneven balance between the different sub-goals. Thus, the big-picture goal is distorted.\\

\noindent It is worth noting that some cases may differ from this story in terms of their causality. Rather than a single complex goal being modularized, sometimes individual agents may come together to form a coalition to pursue a larger-scale goal. Misalignments of interests between these agents can give rise to intrasystem goal conflict in these cases just as with modularized systemic goals. Examples include gut bacterial opportunistic pathogenicity, and some inter-sexual and intragenomic conflict. For instance, intersexual conflict in animals has produced species in which the males deliberately cause the females physical damage when mating. This strategic harming hinders the female’s ability to re-mate in future, and incentivizes her to allocate more resources towards raising that particular male’s genetic offspring. Females have in turn evolved defensive strategies against this, such as armor plating and spines \citep{morrow2003traumatic}. Intersexual coevolutionary ``arms races'' such as these have been documented in a diverse range of species, from ducks to fruit flies \citep{rowe2002sexually}. Rather than a unified goal being modularized, the goal conflict here has arisen in the context of a coalition. The female and male are collaborating through sexual reproduction, but even slight misalignments of their interests can result in dramatic goal conflict.

\subsection{Delegation}
\paragraph{Intrasystem goal conflict can arise through delegation.} The second mechanism by which intrasystem goal conflict may arise is in the \textit{delegation} itself. In the above example, the working groups each pursue their assigned sub-goal faithfully. The problem is that the collective outcome of these agencies, each optimizing for their assigned subgoal is a distorted version of the original big-picture goal. However, the delegation of a goal to another agent can also itself generate intrasystem goal conflict. \\

\noindent In economics, this is called \textbf{a principal-agent problem}. Put simply, this is the problem of conflicting priorities that arises when one party (the \textit{principal}) delegates a goal of theirs to another (the \textit{agent}), who is not entirely value-aligned with the \textit{principal}. The \textit{agent} has other interests, such as self-preservation or gain of influence, which compete with the goal the \textit{principal} has delegated to them. This can result in the distortion or subversion of the delegated goal: the agent pursues their own goals as well as (or instead of) that of the principal. Principal-agent problems are most common where there is a knowledge asymmetry, such that the agent knows more about the relevant matter than the principal. For example, consider a client who has hired a mechanic to fix their car. The client wishes their car to be fixed as cost-effectively as possible; the mechanic wishes to maximize their profits. The principal-agent problem is thus that the client cannot trust the mechanic to report the cost of the car fix accurately. \\

\noindent Principal-agent problems can generate intrasystem goal conflict wherever the components of a modularized big-picture goal are delegated to sub-agents. In particular, the sub-agents are likely to be motivated by self-preservation. If the goal the principal has delegated to them clashes with their own goal of self-preservation, this can produce strong intrasystem goal conflict. To build on the committee example above, now consider that each working group is incentivized to compete with the others to avoid being disbanded. Each exaggerates the importance of their own work, or reconfigures their assigned objective in order to achieve goals of their own. Ultimately, some even break away from the committee, to pursue their emergent goals without the constraints imposed by the committee from which they formed.\\

\subsection{Example: the FDA vs the USDA}
\noindent Intrasystem goal conflict often arises when a system both modularizes and delegates a complex goal. For example, the US Food and Drug Administration (FDA) and the Department of Agriculture (USDA) are sub-agencies of the same government \citep{moss2010warning}. The US government delegates sub-goals to each agency to carry out, yet sometimes their interests and actions conflict with one another. In 2010, the USDA implemented a marketing campaign to promote eating more cheese, to support the dairy industry. Simultaneously, the FDA implemented a marketing campaign of their own to promote eating less cheese, as part of an effort to reduce the saturated fat content of American diets. Despite the fact that both agencies were delegated sub-goals from the same government, their conflicting objectives resulted in their taking actions that hindered one another.
