# Supplementary material for: Introduction to AI Safety, Ethics, and Society
Source: arXiv:2411.01042 source file (2024-11-15)
Supplement: Supplementary file 5 [file Reinforcement_learning.tex]

\section{Reinforcement Learning}\label{sec:reinf-learning}
\subsubsection{Introduction}
This section provides a high-level overview of reinforcement learning (RL). We introduce the basic structure and vocabulary of RL problems and explore how RL is used.\\

\noindent Reinforcement learning techniques attempt to automate the capacity for an agent to learn from its actions and their consequences in an environment \citep{Sutton2018, kaelbling1996reinforcement}. This is distinct from other ML problems, where a system can learn from an existing dataset. Instead, an RL system (or \textit{agent}) learns the hard way, collecting data through experience. An RL agent must learn how to explore different possible actions to attain as much reward as possible. Reward measures the agent’s progress towards its goal and acts as feedback in the learning process. \\

\noindent Reinforcement learning takes its approach from how animals and humans learn to interact with the world. If someone puts their hand on a hot stove, the resulting pain is a significant negative reward, making them unlikely to repeat the same behavior. As intelligent agents, we learn through the way the world responds to our actions. We mostly try to pursue good outcomes, defined by their positive rewards, and avoid bad outcomes, which lead to negative rewards. In this way, teaching automated systems through RL is similar to training a dog. When a dog performs the desired behavior, such as rolling over on command, its trainers might reward it with a treat. The trainers repeat this process as the dog gradually refines its behavior to perform as they desire. \\

\noindent RL techniques have been involved in recent successes in AI. In 2017, DeepMind’s AlphaGo became the first computer program to defeat a world champion in Go, a game long considered the most challenging classical game for AI \citep{silver2016masteringgo}. In 2020, an RL agent developed in less than a year by a small Maryland company won a clear victory over an Air Force pilot in simulated one-on-one combat. RL techniques have been most successful in smaller-scale and less realistic environments, such as video games, where a very accurate simulated environment is readily available. However, games can also be designed to represent real-world environments.

\subsection{Learning Sequential Decision Making through Trial and Error}
\paragraph{Trial and error.} All RL problems involve an agent learning by trial and error to make sequences of decisions. RL agents usually start without prior knowledge of the environment. Over time, the agent accumulates information about its environment and uses it to make better decisions. An agent might learn that bumping into walls constantly does not lead to good outcomes and avoid the walls to find a viable path.

\paragraph{Sequential decision making.} Making sequential decisions effectively is essential to achieving complicated, long-term goals. Accomplishing such goals requires not only that prudent actions are taken but also that they are taken in an appropriate order. To an agent, it is often unclear how one action may impact later actions, but what it does will affect the future and must be modeled. Since decisions are sequential in RL tasks, RL agents might be better suited to achieving complicated, long-term goals. \\

\noindent RL agents can also learn to navigate uncertainty. An agent may not know if a particular choice is good or bad, and the world may change (on its own or in response to its choices), but the agent must act regardless. A self-driving car navigating a busy intersection must sequence its actions--—accelerate, brake, or turn--—based on the positions and speeds of other vehicles, and its current actions will affect these other parts of the environment. To tackle these difficulties, some RL agents are designed to learn from their interactions to develop a sophisticated understanding of their environments to plan their actions.

\paragraph{Sequence modeling.} Sequential decision making (SDM) is a subtype of the general \textit{sequence modeling} task, which involves analyzing and predicting patterns in ordered data. In RL, this data is predominantly in the form of observations of the environment over time. The RL system learns to make decisions based on this information, considering its knowledge of the environment, uncertainty about the world, and past choices.

\paragraph{Distinguishing RL.} Reinforcement learning differs from supervised and unsupervised learning. A key difference between these paradigms is how the ML system obtains information. Supervised and unsupervised learning tasks learn efficient and useful representations on fixed, precompiled datasets. Supervised learning goes about this directly: learning by example. Unsupervised learning addresses similar problems with less guidance, uncovering the latent patterns in unlabeled data without being explicitly told whether it is right or wrong. It is akin to solving a puzzle without seeing the picture on the box. By contrast, RL systems must acquire new information through actions. They receive almost no data at the outset and learn to achieve a goal by actively engaging with an environment and seeing what happens.

\subsection{The Reinforcement Learning Problem}
We can use two toy examples to introduce the central concepts and terms of reinforcement learning. First, we consider the multi-armed bandit---a classic reinforcement learning problem---starting with a simple situation and gradually adding complications to build up to a full reinforcement learning problem. Next, we use a Gridworld problem to introduce the agent-environment loop, a framework for understanding reinforcement learning problems. Finally, we discuss policies: the decisions that RL agents make.

\subsubsection{Multi-Armed Bandits}
In casino lingo, ``one-armed bandits'' refers to slot machines, which have a single lever that takes people’s money. Playing a slot machine is not a reinforcement learning problem because there is only one possible action with a random outcome. However, suppose there is a slot machine with two or more levers. Then, a gambler must decide which lever to pull every time they play. Assuming the levers affect the device differently, one lever might win them more over the long run (such as over 500 pulls). How does one decide which levers to pull and in what order? This problem is called the \textit{multi-armed bandit} problem. 

\paragraph{Exploration-exploitation trade-off.} Multi-armed bandit problems exemplify a dilemma at the heart of reinforcement learning: the trade-off between exploration and exploitation. RL agents must choose between exploring actions with high uncertainty and exploiting actions with a high expected reward. In a multi-armed bandit problem, the agent starts without knowing anything about the expected reward of any given lever. Therefore, the first thing it has to do is gain information about the levers. Trying different actions with uncertain rewards is called \textit{exploration}. By contrast, taking actions with a high expected value is called \textit{exploitation}. In this phase, the agent chooses the actions it expects to yield the highest rewards based on its current understanding of the environment. \\

\noindent Balancing this trade-off between exploration and exploitation is crucial to the success of an RL agent. If the agent explores too much, it might waste resources on low payoff actions or even stumble into actions with negative payoffs. Conversely, if the agent exploits too early, it might settle for suboptimal actions, missing out on potential higher rewards. The challenge lies in determining when and how to shift between exploration and exploitation to maximize the overall benefit. A series of possible strategies aim to make this trade-off, with varying degrees of sophistication; in the following, we outline two simple examples.

\paragraph{Greedy strategies.} First, the agent pulls each lever once and records the payoff it receives from each pull. Then, it pulls whichever lever initially resulted in the highest payoff, which it continues to pull as many times as possible. This is a greedy strategy because the agent only tries each lever once and exploits from then on. However, the problem with a greedy strategy is that the agent cannot be sure that the lever it settles on actually has the highest expected utility.

\paragraph{Epsilon-greedy strategies.} After pulling each lever once, an agent might decide to keep exploring as well. One thing it could so is pull the lever it currently thinks has the highest expected payoff 95\% of the time and pull a random lever the other 5\% of the time. This is called an epsilon-greedy strategy, where ``epsilon'' refers to the small probability of pulling a random lever. Epsilon-greedy is a much better strategy than greedy if there are enough pulls ahead of the agent, since the agent will figure out which lever is best to pull over time. After enough pulls, the agent will pull the most profitable lever 95\% of the time.

\paragraph{Adding context to the bandit problem.} So far, the best lever to pull is always the same and the agent just has to figure out which one it is. However, suppose each lever has two payoff distributions: one for when a light on the slot machine is green, and one for when the light is red. The best lever to pull now depends on the context (the color of the light), which varies randomly. In this environment, the agent needs to take the context into account when it chooses a lever to pull. This is called a \textit{contextual multi-armed bandit} problem.

\paragraph{Adding interaction to the bandit problem.} Suppose further that the light on the slot machine doesn’t vary randomly, but instead changes according to which lever the agent pulls. For example, it might turn green after the second lever is pulled or red if once both levers have been pulled twice. It might be better for the agent to pull a lever with a lower expected payoff at the moment, but will change the context such that the agent can access a greater total profit in the long run. Therefore, the agent needs to be able to estimate expected payoffs over single actions and sequences of actions.

\subsubsection{The Full Reinforcement Learning Problem}
The problem we face now is to come up with a strategy that tells the agent (1) which lever to pull, (2) in varying contexts, and (3) taking into account that its actions can affect that context. The bandit problem is now a \textit{full reinforcement learning problem}. \\

\begin{figure}[htbp!]
    \centering
    \includegraphics[scale=0.3]{images/ML_background/RL problem.jpeg}
    \caption{We can increase RL problems in complexity. Adding detail to multi-armed bandits yields contextual bandits. Adding more complications yield ``full'' RL problems. \citep{xie2020}}
    \label{fig:multi-bandit}
\end{figure}

\noindent The strategies we considered above---\textit{greedy} and \textit{epsilon-greedy}--—aren’t suitable anymore. To develop better strategies, we’ll need more terms and concepts. In particular, we’ll introduce the agent-environment loop as a more technical framework for RL. We’ll also replace our example: instead of the multi-armed bandit, we’ll use a problem called Gridworld.

\paragraph{Gridworld.} In Gridworld, an agent learns to find a particular cell (the goal) in its environment (a two-dimensional grid) while avoiding other cells (hazards). The agent can move into any adjacent open cell. Moving into an open cell is neutral, moving into a hazard is very bad, and moving into the goal is very good.\\

 \begin{figure}[H]
     \centering
     \includegraphics[width=0.92 \linewidth]{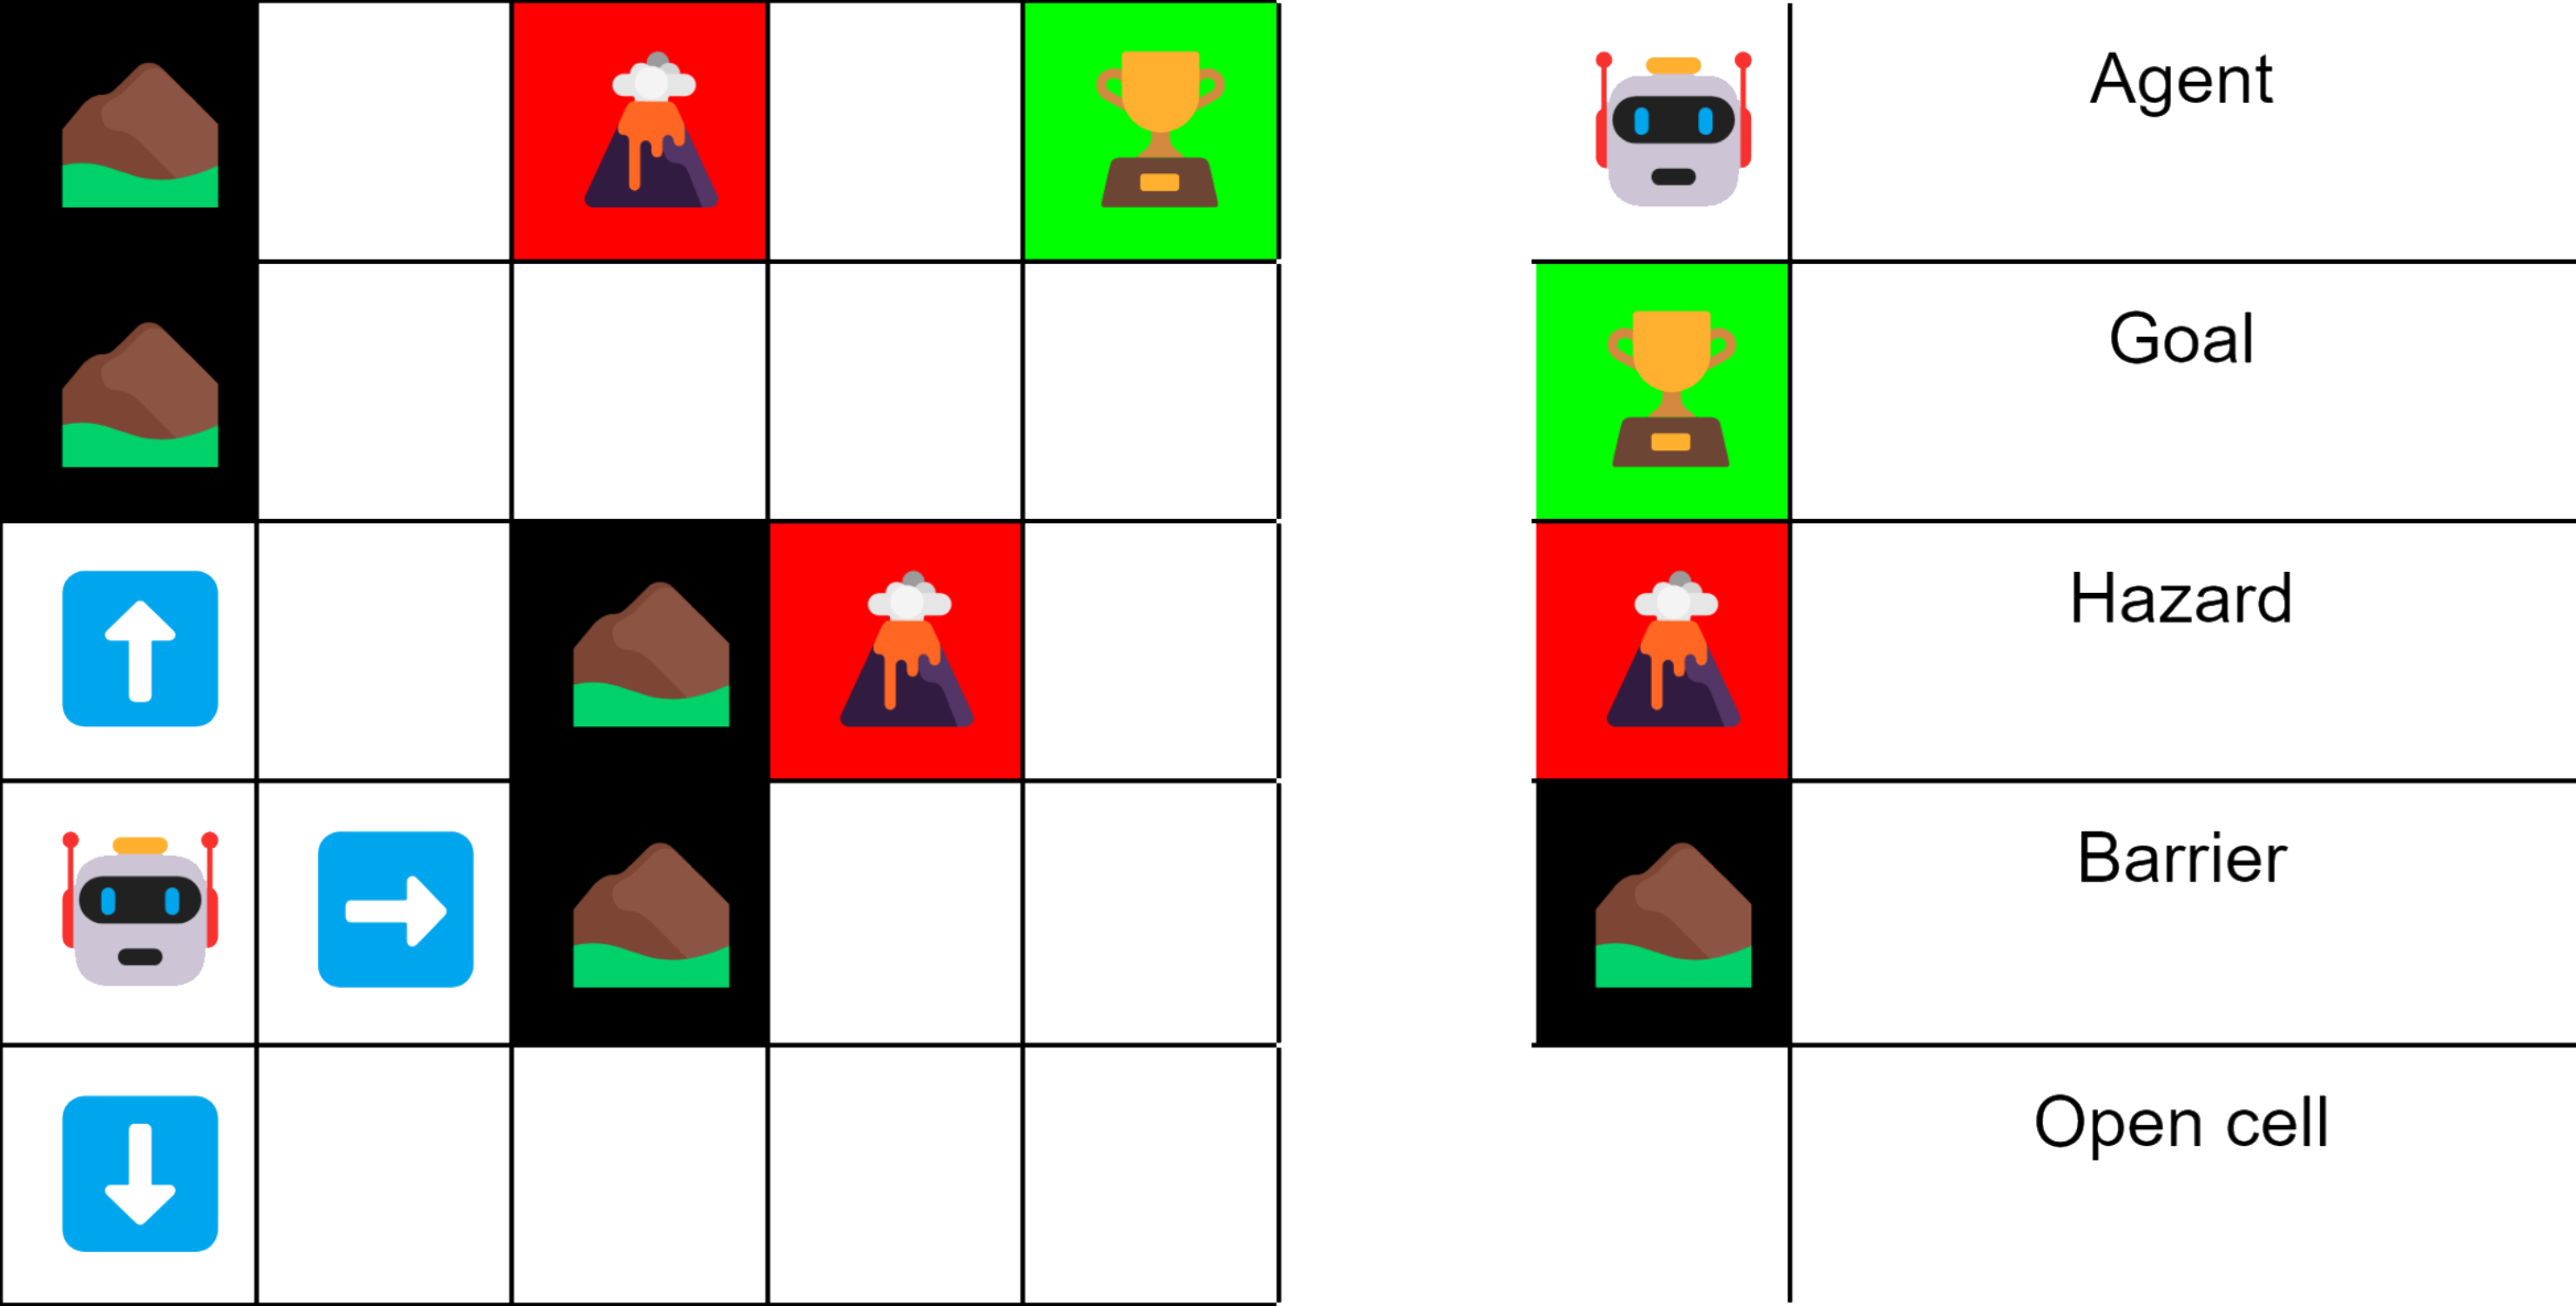}
     \caption{Gridworld is a simple environment used as a toy model in reinforcement learning.}
     \label{fig:gridworld}
 \end{figure}

\paragraph{The agent-environment loop.} The relationship between an RL agent and its environment can be described by the \textit{agent-environment loop}. At each \textit{time step} in this loop, the agent takes some \textit{action} which affects the \textit{environment}. Then, the agent receives a \textit{reward signal} and a state observation from the environment. Using Gridworld as our example, we discuss each of those terms below. \\

\begin{figure}[H]
    \centering
    \includegraphics[width=0.9\linewidth]{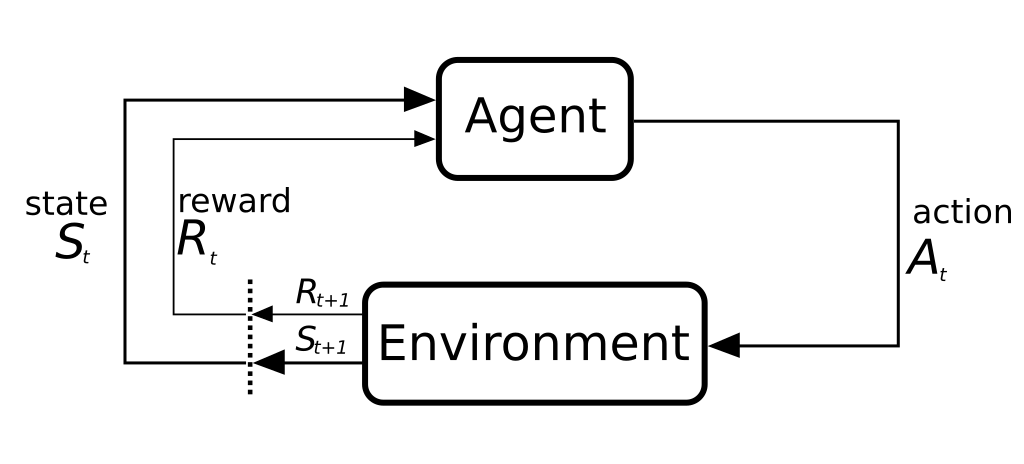}
    \caption{The agent-environment loop shows how the agent chooses an action to affect the environment, which influences the received reward. \citep{wikipedia-markov}}
    \label{fig:agent-environment}
\end{figure}

\paragraph{\textit{Environment and state}}

\paragraph{The environment and state are the world.} In Gridworld, the agent is located on a particular cell and can move to adjacent cells. The environment includes the grid itself, its boundaries, the location of the agent, and anything the agent may encounter. When the environment changes (such as when the Gridworld agent moves), we say that its state changes. A state observation is the information (other than reward) an agent receives from the environment. In Gridworld, an observation might be the agent’s position as well as the positions of the goal, hazards, and barriers. At each time step, the state of the environment updates, and the agent takes a snapshot observation of the available information in the environment.

\paragraph{Environments can be fully or partially observable.} When an agent can observe all of the information in its environment, we say that the environment is \textit{fully observable}. In contrast, when an agent can only observe some of the information about the state of the environment, we say that the environment is \textit{partially observable}. The environment in chess is fully observable because all of the information about the state of the game is available to both players. By contrast, the environment of a poker game is only partially observable: players do not know other players' cards. Our example, Gridworld, is fully observable.

\paragraph{\textit{Actions and action spaces}}

\paragraph{Agents choose actions from their action space.} Agents affect their environment by taking actions. At each time step, they choose an action from the set of all actions available to them. This set is called the \textit{action space}. In Gridworld, the agent takes an action from the action space that describes each possible move to an unoccupied adjacent cell. The agent cannot move into a space occupied by a barrier or outside of the dimensions of the grid.

\paragraph{Action spaces can be continuous or discrete.} A \textit{discrete} action space describes a finite number of possible actions. The action space of our Gridworld agent is discrete---at most, consisting of up, down, left, and right. The same is true for the action space of a multi-armed bandit agent, which consists of a finite number of levers available to pull. In contrast, a \textit{continuous} action space, such as possible directions of movement in a real three-dimensional space, has infinitely many possible actions.

\subsubsubsection{\textit{Rewards}}
\paragraph{Agents get rewards.} At each time step, agents receive a reward from the environment. This reward is represented by a number, which can be positive, negative, or zero. (This means that, in contrast to the everyday use of the word ``reward,'' a reward can be a bad outcome.) The agent in Gridworld might receive a reward of 10 for finding the goal, $-10$ for encountering a hazard, and 0 otherwise. In this case, encountering a danger cancels out the reward from achieving the goal, so hazards should always be avoided. However, exploring neutral squares is free, so this can be done as much as possible.

\paragraph{Rewards are often discounted.} In general, an RL agent’s goal is to maximize the sum of rewards it receives over the long term. Sometimes, though, we want an agent to value short-term rewards more than long-term rewards, such as encouraging agents to behave in a more risk-averse way or to account for their uncertainty. In these cases, we multiply future rewards by a \textit{discount factor} ($\gamma$), and the agent maximizes the \textit{discounted} long-term reward. If the reward at time $t$ is $R_t$, the discounted long-term reward is: $R_t + \gamma^1 R_{t+1} + \gamma^2 R_{t+2} + ... + \gamma^{n} R_{t+n}$.

\paragraph{Rewards are designed to suit the problem.} The process of creating the right rewards for an RL problem is called \textit{reward shaping}. In Gridworld, we might want the agent to find the goal more quickly rather than take a long, roundabout path. To encourage this, we could use rewards to incentivize speed or, equivalently, penalize slowness. If the default reward is 0 when the agent does not encounter the goal or a hazard, reaching the goal in a few time steps would be rewarded the same as reaching the goal in 1,000 time steps. However, if we change this reward to $-1$, the agent has an incentive to reach the goal more quickly.

\subsubsection{Policies}
An RL agent's \textit{policy} (often denoted $\pi$) gives an action for each possible state observation. In simple environments, one can think of a policy as a two-column matrix, where the first column lists all possible state observations, and the second column lists each corresponding action. The strategies we described in the context of the multi-armed bandit problem---greedy and epsilon-greedy---are examples of policies an agent could use when the environment has a single state. In the contextual multi-armed bandit problem, we added a second state. A policy over two states might look like: ``If green, pull lever X; if red, pull lever Y.'' 

\paragraph{Policies can be deterministic or stochastic.} A \textit{deterministic policy} assumes that all actions are taken with certainty. In the bandit problem, the \textit{greedy} strategy is a deterministic policy. In Gridworld, a deterministic policy may be to always move to the right or to follow a particular path to the goal. In contrast, a \textit{stochastic policy} assumes that actions are taken with some randomness, such as randomizing between pulling different levers when following an \textit{epsilon-greedy} strategy. In Gridworld, a stochastic policy might be to choose randomly among actions for the first few time steps.

\paragraph{Optimal policies.} An optimal policy is a policy that, if followed, maximizes the sum of (discounted) rewards. In Gridworld, the optimal policy would describe the shortest route to the goal from any starting location. In more complex problems, however, computing the optimal policy is often intractable. For example, in chess, an optimal policy would need to give the best move in all $\sim 10^{45}$ possible board positions. However, approximating the optimal policy has still produced RL chess agents that far surpass the human level of play.

\subsubsubsection{Summary} 
\noindent This section introduced the agent-environment loop as a technical framework for talking about reinforcement learning problems. In place of the ``strategies'' we considered in the multi-armed bandit problem, we introduced the idea of a policy, which gives an action at each time step according to the agent’s observation of its environment. In Gridworld, we could manually define a policy for the agent to follow--—but that would defeat the purpose of the problem, which is to have the agent learn for itself. The next section explores how reinforcement learning algorithms automate designing policies.

\subsection{Methods for Solving RL Problems}
\textbf{RL algorithms develop better policies.} RL algorithms serve as the blueprints to guide the learning process, aiming to discover the optimal strategy for the agent in its environment. While all RL algorithms share a common theme of learning through trial and error---exploring the environment, observing the results, and adjusting behavior based on rewards and penalties---their unique characteristics arise from the specific approach they take toward learning. Specific RL algorithms are distinguished by how or what their agent learns. 

\paragraph{Model-based vs Model-free RL.} We can organize different RL algorithms into two broad approaches based on their computational learning strategies: \textit{model-based} and \textit{model-free}. In \textit{model-based} RL algorithms, the agent constructs an internal model of its environment. The agent learns how its world operates and represents cause-and-effect relationships, using this model to predict the outcomes of actions and optimize its behavior. An RL agent playing chess could develop a model of the game, representing the rules and understanding that specific configurations win the game. It can use this model to plan its moves, simulating different sequences to anticipate their results before making a move. Model-based methods are most applicable to problems in environments with easily representable dynamics. \\

\noindent In contrast, \textit{model-free} RL methods learn directly from experience without explicitly modeling the underlying mechanics of the environment. Instead, the agent develops associations between actions and rewards. These simple associations serve as a kind of ``intuition'' for projecting what actions lead to the most reward in given situations. Consider an RL agent learning to play Pac-Man: it does not comprehend the game’s design or the ghosts’ behavior. Instead, through trial and error, it learns strategies like ``eating a power pellet and then chasing ghosts leads to high scores.'' The AI uses these associations, rather than an internal model of the game, to guide its future actions. Model-free approaches are often best for problems where the environment’s dynamics are complex or unknown and abundant data is available for learning.

\paragraph{Policy-based vs Value-based RL.} Another distinction is how an RL agent represents what is ``good'' in its environment, learning how good states or actions are, how good policies are, or both at the same time. In \textit{policy-based} RL methods, the agent focuses on learning an effective policy: a set of rules guiding its actions in response to different states. Rather than calculating the value of each state or action, the agent optimizes the policy based on the observed rewards of its actions. The agent may pursue an action because it is part of a good policy without knowing exactly how good the action itself is. An RL agent learning how to balance a pole on a cart for a robotics task does not explicitly calculate the value of different pole angles or cart positions. Instead, it adjusts its policy---how it responds to various states---to optimize for the goal of keeping the pole balanced. It might learn the policy ``if the pole tilts to the right, move the cart to the right.'' This approach is often best for handling continuous action spaces but struggles with finding the optimal policy in large or complex environments due to the vast number of potential policies. \\

\noindent Conversely, \textit{value-based} RL methods prioritize learning the value of different states or actions within the environment. The agent evaluates and ranks states or actions based on their potential to yield rewards, selecting the ones with the highest estimated reward. An RL agent playing tic-tac-toe evaluates each move's value (putting a mark in an empty cell) based on the likelihood of that move leading to a win and chooses the action with the best outcome. The agent learns to take actions that maximize the cumulative reward over time without specifying a policy.

\paragraph{An agent’s value function estimates the expected reward of a state or state-action pair.} Internally, an agent might estimate how good or bad certain states are. The agent learns a \textit{value function} to keep track of these estimates, which it can use to estimate the returns of different actions. Value functions can also estimate how well a policy performs in the long run by calculating the expected cumulative reward of following a policy over time. An agent in Gridworld could learn a value function to estimate the reward of moving into a particular space. Alternatively, an RL agent in a car’s GPS might use a value function to estimate the value of different routes based on the expected travel time. \\

\begin{figure}[H]
    \centering
    \includegraphics[width=0.85\linewidth]{images/ML_background/two-types updated.png}
\caption{Value-based methods can either evaluate the value of a state or the value of a state-action pair. \citep{huggingface}}
    \label{fig:value-methods}
\end{figure}

\paragraph{Value functions can focus on the value of a state or an action.} There are two main types of value functions in reinforcement learning: \textit{state-value functions} and \textbf{action-value functions}. A state-value function ($V^\pi(s)$) estimates the expected cumulative reward that an agent will receive when starting from a state $s$ and following a policy $\pi$. We can estimate the \textit{state values} of each location in Gridworld, assuming the agent follows a random policy. In every area, the agent moves to a random adjacent open cell, repeating this process until it bumps into the goal or a hazard. The state-values of cells near the goal are higher than those far away from the goal and much higher than those near the hazard. The state-value function for this policy gives us an estimate of how likely it is that the agent will reach the goal or hit a hazard from each cell. \\

\noindent An action-value function $(Q^\pi(s,a))$ estimates the expected cumulative reward that an agent will receive by taking an action $a$ from a state $s$ and following a policy $\pi$. In other words, it estimates the ``value'' of taking a particular action in a particular state. Action-values are often referred to as \textit{Q-values}, and the value functions that output them are called \textit{Q-functions}. One way to approach an optimal policy in RL is by learning the Q-function.

\paragraph{Q-learning.} Q-learning is one of the oldest and most popular reinforcement learning algorithms. Q-learning approaches the RL problem by estimating how good it is to take actions in each state. Chess has numerous potential moves (actions) for each position on the board (state). Q-learning would assign a score (Q-value) to each state-action pair, indicating how beneficial each move is likely to be. The goal is to determine the optimal Q-function---the rule that most accurately assigns these scores---by mapping every state-action pair to its optimal Q-value. When the environment has a finite number of states and moves, the Q-function can be represented as a table, where each row represents a state, and each column is an action.\\

\noindent Therefore, Q-learning is the process of updating the Q-values of each action iteratively based on the outcomes observed in the environment. At each time step, the agent chooses the action with the highest associated Q-value from those available to it in its current state. This generates a new observation and reward, from which the agent updates its estimates. Each table entry will converge to its optimal value through many iterations.

\paragraph{Q-learning in Gridworld.} In Gridworld, we have four actions (North, South, East, West) and 25 states (unique grid cells). Therefore, the Q-function table would have 100 Q-values, one for every state-action pair:\\

\begin{table}[H]
    \centering
    \begin{tabular}{|c|c|c|c|c| }
    \hline
     & North & South & East & West \\
    \hline
    (0,0)     & Q((0,0), North) & ... & ... & Q((0,0), West)  \\
    \hline
    (0,1) & ... &  & & ... \\
    \hline
    ... & ... &  & & ... \\
    \hline
    (4,5) & ... &  & & ... \\
    \hline
    (5,5) & Q((5,5), North) & ... & ... & Q((5,5), West) \\
    \hline
    \end{tabular}
    \caption{Example Q-value table for Gridworld.}
    \label{tab:q-val-table}
\end{table}

\noindent In the beginning, all the Q-value estimates are zero because the agent has no information about the environment and will take random actions. Eventually, the agent reaches a positive or negative reward state. Say, for example, our agent gets lucky and finds its way to cell (0,4) and chooses to go east. It will receive a reward of +1, and its estimate of the Q-value for ((0,4), East) will be increased accordingly. The agent learns that moving East is a good action to take in the state (0,4), and it will be more likely to take this action the next time it is in the same state.  \\

\noindent Over time, the negative and positive Q-values will propagate through the table. The agent will repeat this process many times as it explores the states in the environment and tries different actions, and if all goes well, its estimates will converge to the optimal Q-function. By learning which actions are desirable to take in which states, the agent learns how to navigate the world successfully. As the environment becomes more complicated and action space becomes larger, computing exact Q-values becomes less computationally feasible. Instead, we might try to estimate the Q-function using a less computationally taxing method. One such method involves using neural networks to estimate the Q-function. This is an example of a method known as deep RL.

\begin{figure}[H]
    \centering
    \includegraphics[width=0.6\linewidth]{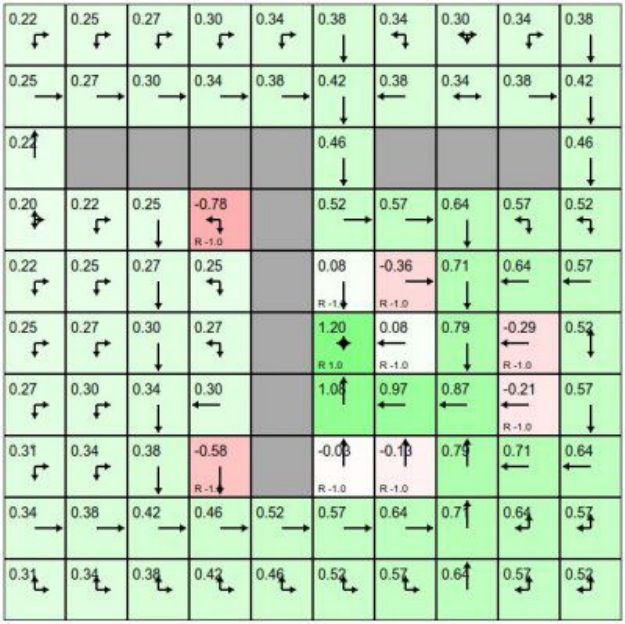}
    \caption{Q-values can be estimated for every possible state in Gridworld. \citep{gridworld}}
    \label{fig:gridworld}
\end{figure}

\subsection{Deep Reinforcement Learning}

\noindent  Deep reinforcement learning (deep RL) is the area of machine learning that leverages deep learning (DL) to help solve reinforcement learning (RL) problems. Deep learning, which uses neural networks to compress and extract information from vast amounts of data, can be applied to RL problems such as sequential decision making. In this setting, the RL setting provides signals to help neural networks learn useful representations for the task at hand. 

\paragraph{Deep learning is a substantial part of nearly all major RL successes in recent years.} As the complexity of modeling even seemingly simple problems can explode at astonishing rates, using RL to accomplish interesting tasks demands powerful, scalable methods. Some of the ways deep learning can be used in RL include: 

\begin{itemize}
    \item \textbf{Environment.} In model-based RL, deep learning can be used to learn the dynamics model of the environment, which can then be used for planning and decision-making.
    \item \textbf{Policy function.} Deep learning can help optimize complex policies for continuous action spaces.
    \item \textbf{Value function.} Deep neural networks such as Deep Q-Network (DQN) can be used to estimate the Q-function. This is particularly useful for problems with many, or even infinite, possible state-action pairs. Instead of capturing the Q-function in a state-action matrix, it can be directly encoded in a neural network, which takes the state-action pair as an input and outputs the action-value.
\end{itemize}

\noindent In the next section, we explore a few recent successes of deep RL. Along the way, we’ll introduce a few more high-level techniques used to solve common problems to conclude our discussion of RL.

\subsection{Examples of RL}\label{sec:examples-of-rl}

\subsubsection{AlphaGo}
In 1997, IBM's Deep Blue made history by becoming the first AI to defeat a world-class chess player. Yet it was not until nearly two decades later that an AI managed to surpass humans in the game of Go, when AlphaGo won against the best player in the world in 2017. Go is similar to structure to chess, both being fully observable two-player turn-based games, but Go is far more complicated. Unlike chess, with only 20 possible first moves, Go starts with a staggering 361 choices. This complexity outstrips the capabilities of the brute-force computations that Deep Blue could rely on to evaluate positions. Therefore, AlphaGo had to rely on the more sophisticated methods of deep RL to master the game. By playing millions of games against itself, AlphaGo honed its strategy and emerged as the world’s top Go player.

\paragraph{RL agents can learn by competing against themselves.} One training method that has proven effective is \textit{self-play}. In part, this is because an RL model presents itself with an appropriate opponent for an amateur: not a novice, who it could win against easily without learning anything new, or a grandmaster, who would win against it decisively enough that it might not understand how it could have acted differently to prevent a loss. Instead, the best way for an amateur to improve is to play against opponents of similar skill levels. The insight of self-play is that a RL agent can learn from players of a similar strength by playing against versions of itself. This allows the agent to improve and reach a superhuman level of play without external intervention.

\subsubsection{Atari} 
The Atari games are a collection of video games developed between the 1970s and 1980s for the Atari 2600 console, characterized by their simple graphics, straightforward controls, and challenging gameplay. Some of the most popular Atari games are Space Invaders, Pac-Man, and Pong. Each game has its own unique set of rules, goals, and strategies. As they provide a diverse set of challenges that an RL agent must learn to overcome, Atari games have long served as a popular testing ground to assess the capabilities of RL algorithms. They provide a platform to evaluate how well RL agents can navigate complex environments and master motor skills. In 2013, the DeepMind team proposed the original set of 57 Atari titles as an RL benchmark. Since then, RL agents have met or surpassed human performance in every single one of these games \citep{mnih2013playing}. However, some games took years longer to solve---and inspired new learning methods. 

\paragraph{Sparse rewards present challenges to learning.} One particularly difficult game for RL agents to solve is Montezuma’s Revenge. In this game, players must make a long series of precise movements to reach the first reward. They must navigate through a series of mazes to collect treasure, including a key. The key is necessary to advance to the next level. The challenge lies in the fact that an RL agent that moves randomly at first is unlikely to ever encounter this first reward, let alone complete a level. These rewards are rare and hard to find. It also requires a delicate balance between exploration and exploitation, as the key is often hidden in parts of the maze the agent would not visit unless it is exploring, but exploring too much can lead to running into traps or enemies. To reach any reward at all, the player must perform a complex sequence of actions where a single mistake can lead to losing a life. Learning this game through trial and error can take a long time. \\

\noindent Montezuma’s Revenge is a classic example of the problem of \textit{sparse rewards}, where the agent receives few signals to guide learning. In environments like this, rewards are few and far between, depriving RL agents of the feedback they need to learn effective strategies. In contrast, a game like Breakout (in which a paddle at the bottom of the environment is used to deflect a ball towards bricks to break them) is much easier for RL agents. Even random movements are likely to deflect the ball, break a block, and earn a reward reasonably quickly.

\paragraph{Preferences for novelty can help overcome sparse rewards.} An RL agent which prefers \textit{novelty} is rewarded for new actions and observations. This method is how an RL agent eventually solved Montezuma’s Revenge: it learned to find the first reward simply by seeking out new observations. Imagine an RL agent rewarded for novelty finds itself in an empty room with a single closed door. After aimlessly wandering around the room for a while, the RL agent will eventually ``get bored'' and figure out how to open the door, venturing out of the room. In this way, novelty-seeking agents can exhibit intelligent behavior without being explicitly rewarded for any particular goal. There are many similar ways to develop RL agents and promote optimal behavior. \\

\noindent The exploration of Atari games and the development of novel methods to tackle them have significantly advanced the field of reinforcement learning, providing valuable insights into the learning process of RL agents.

\subsubsection{StarCraft} 
In 2019, DeepMind’s RL system \textit{AlphaStar} defeated an expert human player 5-0 in a StarCraft II match \citep{Vinyals2019}. StarCraft II is a complicated real-time strategy game that pits two players against each other in a vast battlefield. StarCraft has many more possible actions and states than chess, Go, or Atari games, making it a formidable challenge for players and AIs alike. 

\paragraph{AlphaStar learned to overcome significant uncertainty.} The game’s difficulty is further amplified by its partially observable environment, as most of the map is shrouded in a fog of war, and players can only see areas where they have deployed units. This means players must constantly act under uncertainty, making educated guesses about the state of the environment and making predictions about their opponent’s actions and strategies. AlphaStar’s ability to overcome the challenges of uncertainty, a large action space, and the need for strategic planning underscores the potential of RL in navigating complicated, uncertain environments.

\subsubsection{Diplomacy} 
\noindent In 2022, Facebook AI Research (FAIR) developed \textit{Cicero}, a program that reached human-level performance in the strategy game Diplomacy \citep{Bakhtin2022}. In this game, players compete to take over a model of Europe against the backdrop of the First World War. One of the central features of Diplomacy is that players communicate in natural language to form alliances and negotiate in between each turn. Cicero navigated not only the game’s moves but also natural language processing and generation. 

\paragraph{Cicero learned how to deceive.} Cicero's success required learning how to deceive human players. It is documented to have sometimes convinced other players to agree to lopsided deals or break promises when it was advantageous. In other words, Cicero developed a capacity for deception. This result is not surprising: success in Diplomacy often requires deception.

\subsubsection{Conclusion}
This section explores the major concepts, terms, and techniques involved in reinforcement learning. First, we used two simple examples---Multi-Armed Bandits and Gridworld---to outline the major concepts and terms used in RL. At each time step, the agent takes some action drawn from the action space, which affects the state of the environment. Then, the agent receives a reward signal and a state observation from the environment. The agent acts according to its policy, which specifies an action for every possible state observation. The agent’s value function computes the expected cumulative reward of a certain state (state-value) or state-action pair (Q-value) given a certain policy. Q-values can be used for Q-learning, one popular learning algorithm, to update an agent’s policy toward an optimal policy.\\

\noindent After outlining the major concepts and terms used in RL, we discussed some powerful techniques used in groundbreaking RL systems. First, deep RL uses deep learning to estimate value functions and policies in tasks that are too complex to allow exact computation. Second, self-play expands the ability of RL systems in competitive tasks by repeatedly pitting the system against itself. Finally, RL systems can overcome the problem of sparse rewards through preferences for novelty.
