# Supplementary material for: Introduction to AI Safety, Ethics, and Society
Source: arXiv:2411.01042 source file (2024-11-15)
Supplement: Supplementary file 6 [file Tail_events_appendix.tex]

\section{Long-Tailed and Thin-Tailed Distributions}\label{appendix-tails}
In the main text, we introduced tail events and black swans, discussing their importance in the context of safety engineering. We briefly considered the differences between long-tailed and thin-tailed distributions, but did not go into much detail. In this appendix, we discuss the differences between the types of events that have long tails and the types of events that do not, building a more comprehensive understanding of the features of both types of events. 

\subsubsection{Long-tailed distributions}
\paragraph{In long-tailed distributions, extreme occurrences can have a huge effect.} Long-tailed distributions are those where values can vary so much that a single extreme instance or a few extreme instances can dominate the total value. In other words, the top few instances have a highly disproportionate impact. We will now explore some examples of variables with long-tailed distributions. \\

\noindent \textit{Book sales}: Around 0.2\% of books account for around 50\% of total book sales. It is possible for a single, highly popular book to sell many more copies than many less popular books combined. Such a book might be termed a tail event within book sales.\\

\noindent \textit{Music}: Around 1\% of artists in the music industry earn around 77\% of the total revenue from all recorded music. A single, highly successful artist can earn much more than many lesser-known artists combined. \\

\noindent \textit{Net worth}: Wealth distribution is a classic example of a long-tailed distribution. Global wealth reports frequently find that the richest 1\% of people own close to half of the world’s total wealth.\\

\noindent \textit{Web hits}: There are around 200 million actively maintained websites on the internet, but the vast majority receive very few visitors. A single, highly popular website, such as YouTube or Facebook, can receive many more visitors per day than many obscure websites put together. \\

\noindent \textit{Earthquake magnitude}: The frequency distribution of earthquake magnitudes is described by the Gutenberg-Richter law. The exact distribution depends on the region and conditions, but typically, there are around 10,000 times more earthquakes of magnitude 3.0 or above than earthquakes of magnitude 7.0 or above. However, a single magnitude-7 earthquake can do much more damage than all the magnitude-3 earthquakes combined. \\

\noindent \textit{Crater diameter}: Most impact craters, resulting from collisions with other astronomical bodies, are relatively small. Out of around 200 such craters discovered on Earth, about 120 are between 0 km and 10 km in diameter, while fewer than 10 have a diameter of 100 km or more. Moreover, the 5\% largest craters have a combined diameter of around a third of the total diameter of all craters. \\

\noindent \textit{Solar flares}: Solar flares of relatively low intensity are quite common, while solar flares of much higher intensity happen infrequently. However, studies have found that the few large flares mostly determine the total energy of all flares. \\

\noindent \textit{Word frequency}: The vast majority of words in a given text appear infrequently. However, certain words, like ``the,'' ``of,'' and ``and,'' appear far more frequently than most others. The total appearances of a handful of these commonplace words can outweigh the total appearances of a large number of rarer words.\\

\noindent These variables are said to have a long tail because, in their frequency distributions, the rare, extreme events appear at very large values of x; the ``tail'' of the graph extends far along the x-axis. This is also why rare, high-impact events are called tail events; they exist in the tail end of a long-tailed distribution. \\

\noindent This type of phenomenon is sometimes referred to as the ``Pareto principle'' or ``the 80-20 rule.'' This asserts that, in many distributions, 20\% of the instances contribute 80\% of the total outcome. The exact figures depend on the variable, but the 80-20 rule is a well-known framing of the general concept of long-tailed distributions.

\subsubsection{Thin-tailed distributions}
\paragraph{In thin-tailed distributions, no event is extreme enough to have much effect.} Thin-tailed distributions are those with relatively little variation between values, meaning that even the most extreme instances cannot substantially affect the overall landscape. Many human characteristics, such as height, general intelligence, and lifespan, have thin-tailed distributions. Note that these examples all follow something akin to a normal distribution, or bell curve, as shown in \Cref{fig:excess}. Normal distributions have a maximum density at the most common value and a tail on either side. The frequency decreases rapidly as we move away from the most common value.

\begin{figure}[H]
    \centering
    \includegraphics[width=0.8\linewidth]{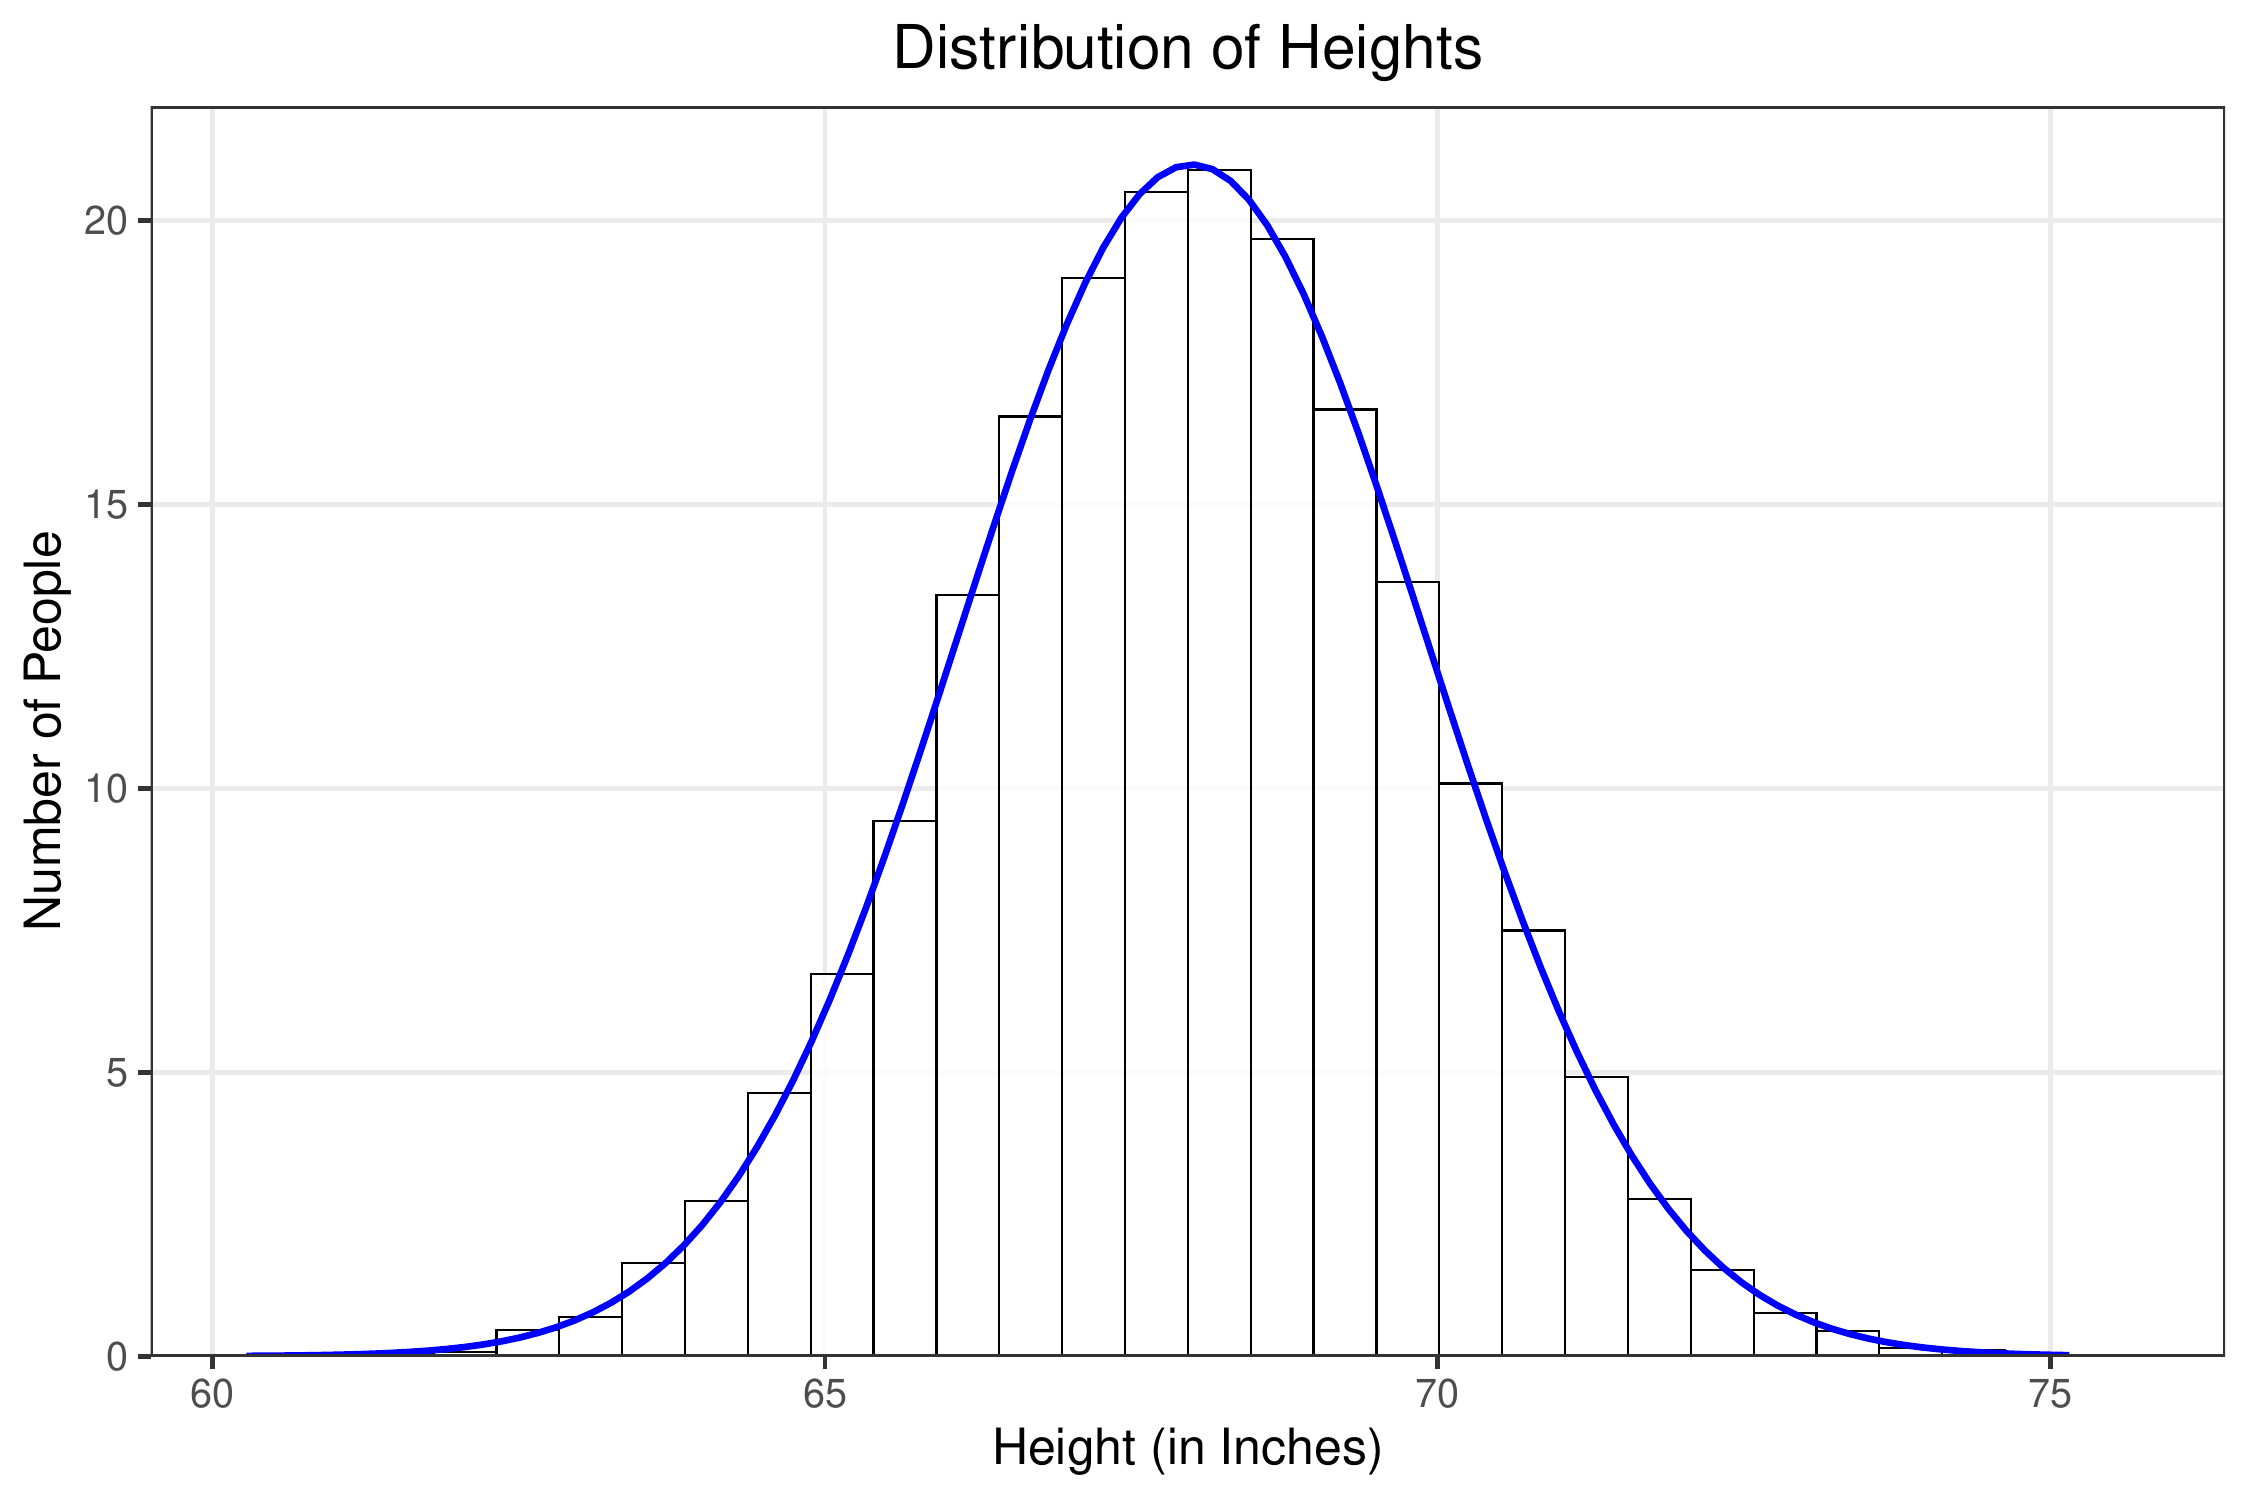}
    \caption{Many natural phenomena (such as the distribution of humans' heights) follow the normal distribution.}
    \label{fig:excess}
\end{figure}

\noindent All of these example characteristics vary between individuals, but the range of variation is much narrower than it is for variables with long-tailed distributions. For example, while human height varies, there has never been a person who was fifty feet tall. Even the tallest person in the world is not ten times taller than the shortest. This contrasts with long-tailed distributions such as book sales, where a bestseller can easily sell thousands of times more copies than a less popular book.\\

\noindent Following on from this, under thin-tailed distributions, no single instance is so extreme that it can account for a large share of the total among a group; the total height of the tallest 10\% of people will not be significantly more than 10\% of the total height of all people. Again, this contrasts with long-tailed distributions, where a small fraction of instances can account for most of the impact. \\

\noindent Thin-tailed distributions are so-called because, in their frequency distributions, the value on the y-axis rapidly approaches zero for highly extreme events; the ``tail'' of the graph quickly becomes vanishingly thin.

\subsection{Heuristics and Models for Thinking About Long Tails and Thin Tails}
\paragraph{Generally, long-tailed variables span orders of magnitude and thin-tailed ones do not.} A general rule of thumb for distinguishing between long-tailed and thin-tailed variables is to ask: Does it still make sense if we add a zero at the end of a data point’s value? In other words, can the variable span multiple orders of magnitude? If the answer is no, it is more likely to be thin-tailed; if yes, the variable is more likely to be long-tailed. \\

\noindent We should note that this test is imperfect. Lifespan is a thin-tailed variable that spans orders of magnitude; some live to be over 100 years old, while others live for fewer than ten years. Nonetheless, this question usually indicates whether a variable has a long or thin tail. \\

\newpage
\begin{wrapfigure}{l}{8.1cm}
\includegraphics[width=8.1cm]{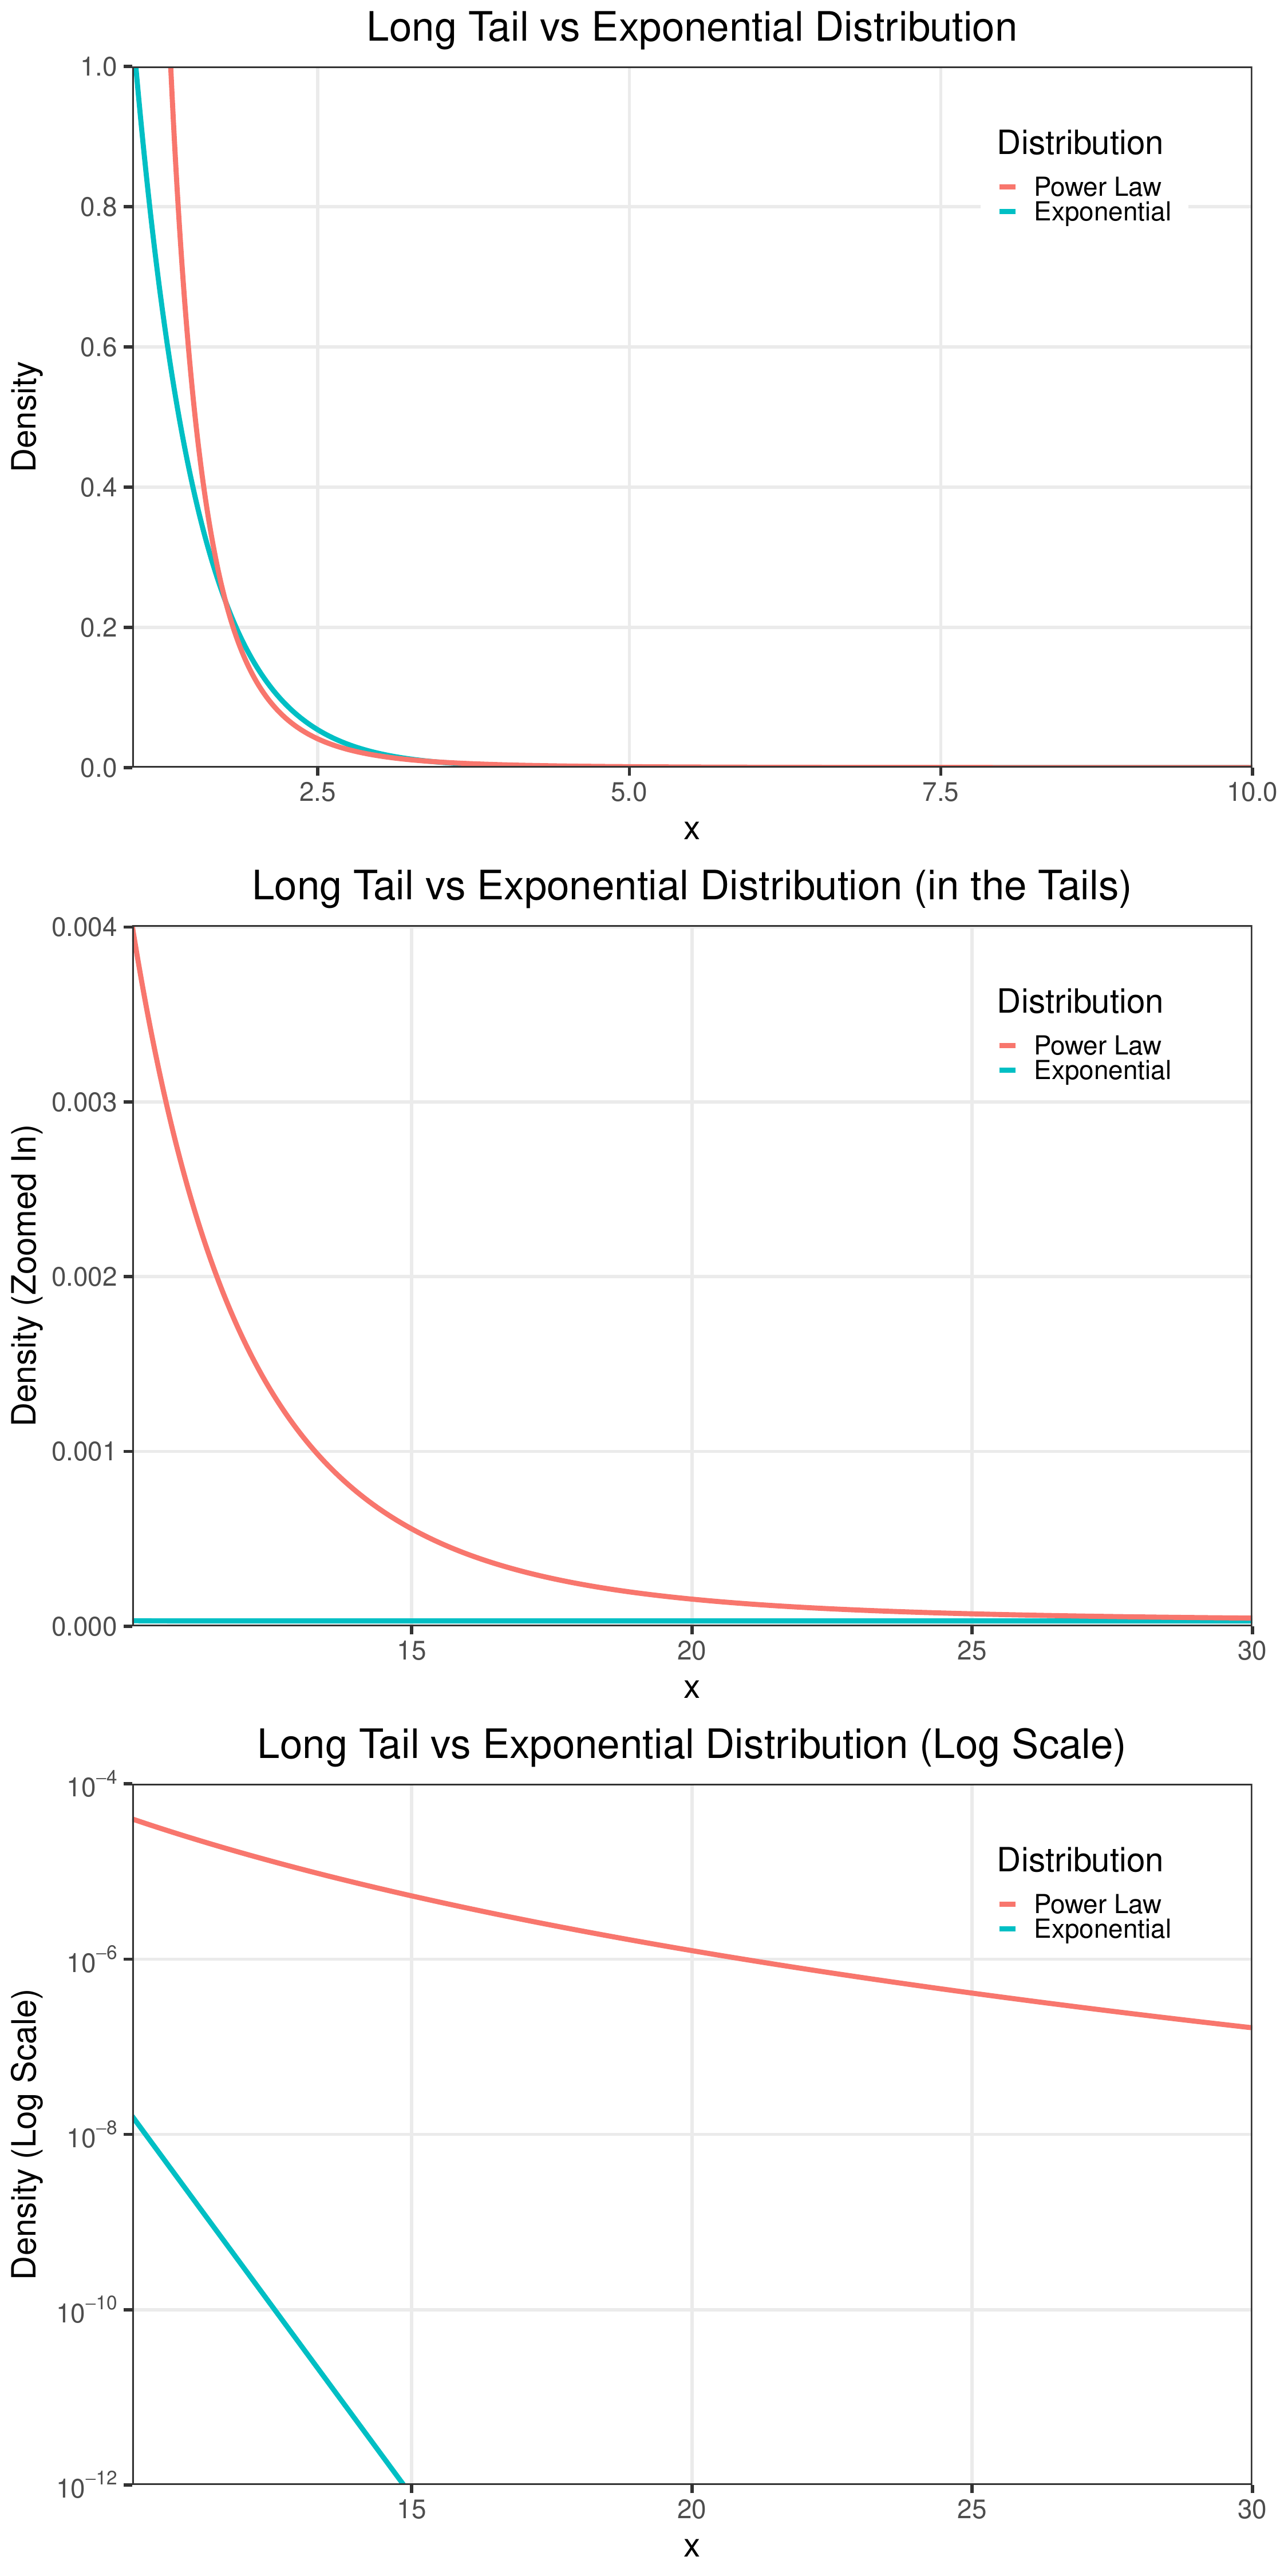}
\caption{Exponential distributions are not long-tailed, even though they look quite similar at a normal scale (top). Looking at extreme values (middle), especially on a log scale (bottom), shows us that they have thin tails.}\label{wrap-fig:exponentials}
\end{wrapfigure} 
\paragraph{Exponential distributions are thin-tailed distributions.} Figure \ref{wrap-fig:exponentials} shows an exponential distribution (in black) and a power-law distribution (in grey). At first glance, they look quite similar. However, in the second and third graphs, we zoom in to the tail end of the graph and change the y-axis to a logarithmic scale. Here, we can see that, beyond a certain point, the exponential distribution decays significantly more quickly than the power-law distribution. As a rough heuristic, frequency distributions that decay more slowly than an exponential are generally considered long-tailed, while those that decay more quickly are considered thin-tailed.

\paragraph{There is a significant difference between extreme events being unlikely and astronomically\nolinebreak[4] unlikely.}  In practical terms, for\nolinebreak[4] events\nolinebreak[4] with exponential distributions—and distributions that decay more quickly than them—the probability of extreme events rapidly becomes astronomically small. In fact, it becomes so small that, at some point, we can consider it essentially zero. Under distributions that decay more slowly than exponentials, such as the power law depicted, the probability of extreme events is still low. The important difference, however, is that they are possible. Under long-tailed distributions, they are rare but possible and have an enormous impact if they happen. \\

\noindent Note that the frequency of extreme events depends on how we define ``extreme,'' namely, how far along the x-axis the event appears. We use ``extreme'' to describe events so far from the most common value that they can significantly impact the mean and represent a disproportionately large fraction of the total. \\

\noindent Returning to the risk equation, under thin-tailed distributions, the probability, $P$(hazard), of a tail event is so astronomically small that tail events do not affect the total risk much. Under long-tailed distributions, the probability, $P$(hazard), of a tail event is small, but the severity is so large that tail events can substantially alter the total risk. \\
\begin{equation*}
    \text{Risk}(\text{hazard}) = P(\text{hazard}) \times \text{severity}(\text{hazard})
\end{equation*}

\noindent Next, we will consider three specific differentiators of long- and thin-tailed distributions: excess conditional expectation, multiplicative vs. additive phenomena, and preferential attachment.

\subsubsubsection{Excess conditional expectation}
\paragraph{Excess conditional expectation is the margin between minimum and actual values.} Another difference between long-tailed and thin-tailed distributions is the ``excess conditional expectation'' \citep{Marsden2017}. This is the difference between the conditional expectation--—our best guess of how large something will be, given that we know that it is already above or below some threshold---and the threshold itself. Only long-tailed distributions tend to have high excess conditional expectation. This concept is best illustrated with examples.

\paragraph{Example: Long Jump, Thin Tails.} Imagine we are at a training session for long-jump athletes. The world record for the long jump is around 9 meters. If an athlete jumps 7 meters at the training session, then this represents a definite lower bound for their personal best: it is at least 7 meters. If we are then asked to guess their actual personal best, we might estimate that it could be close to 8 meters.\\

\noindent If another athlete jumps 8 meters at the training session, then we might expect that their personal best is around 8.5 meters. If yet another athlete jumps 8.5 meters, then we might think their personal best is around 8.7 meters.\\

\noindent Figure \ref{fig:excess} shows a plot of the observed jumps as blue dots, and our best guess of each athlete’s personal best in dotted lines. Notice how, as the definite minimum value increases, we observe a shrinking margin between this lower bound and our estimate of the athlete’s actual maximum jump. This is because we know that the world record sets a definite limit on what any individual’s personal best could be. The closer the observed distance gets to the world record, the less room there is for the athlete to have jumped further.

\paragraph{Under thin tails, excess conditional expectation shrinks as values get more extreme.} The margin between the known lower bound of something and the estimate of its actual value is the excess conditional expectation. Under thin-tailed distributions, this margin tends to shrink as the minimum value becomes more extreme. This is because there is a limit to how extreme it can become; as the lower bound approaches that limit, there is less room for the actual value to be different.\\

\begin{figure}[H]
    \centering
    \includegraphics[width=0.95\linewidth]{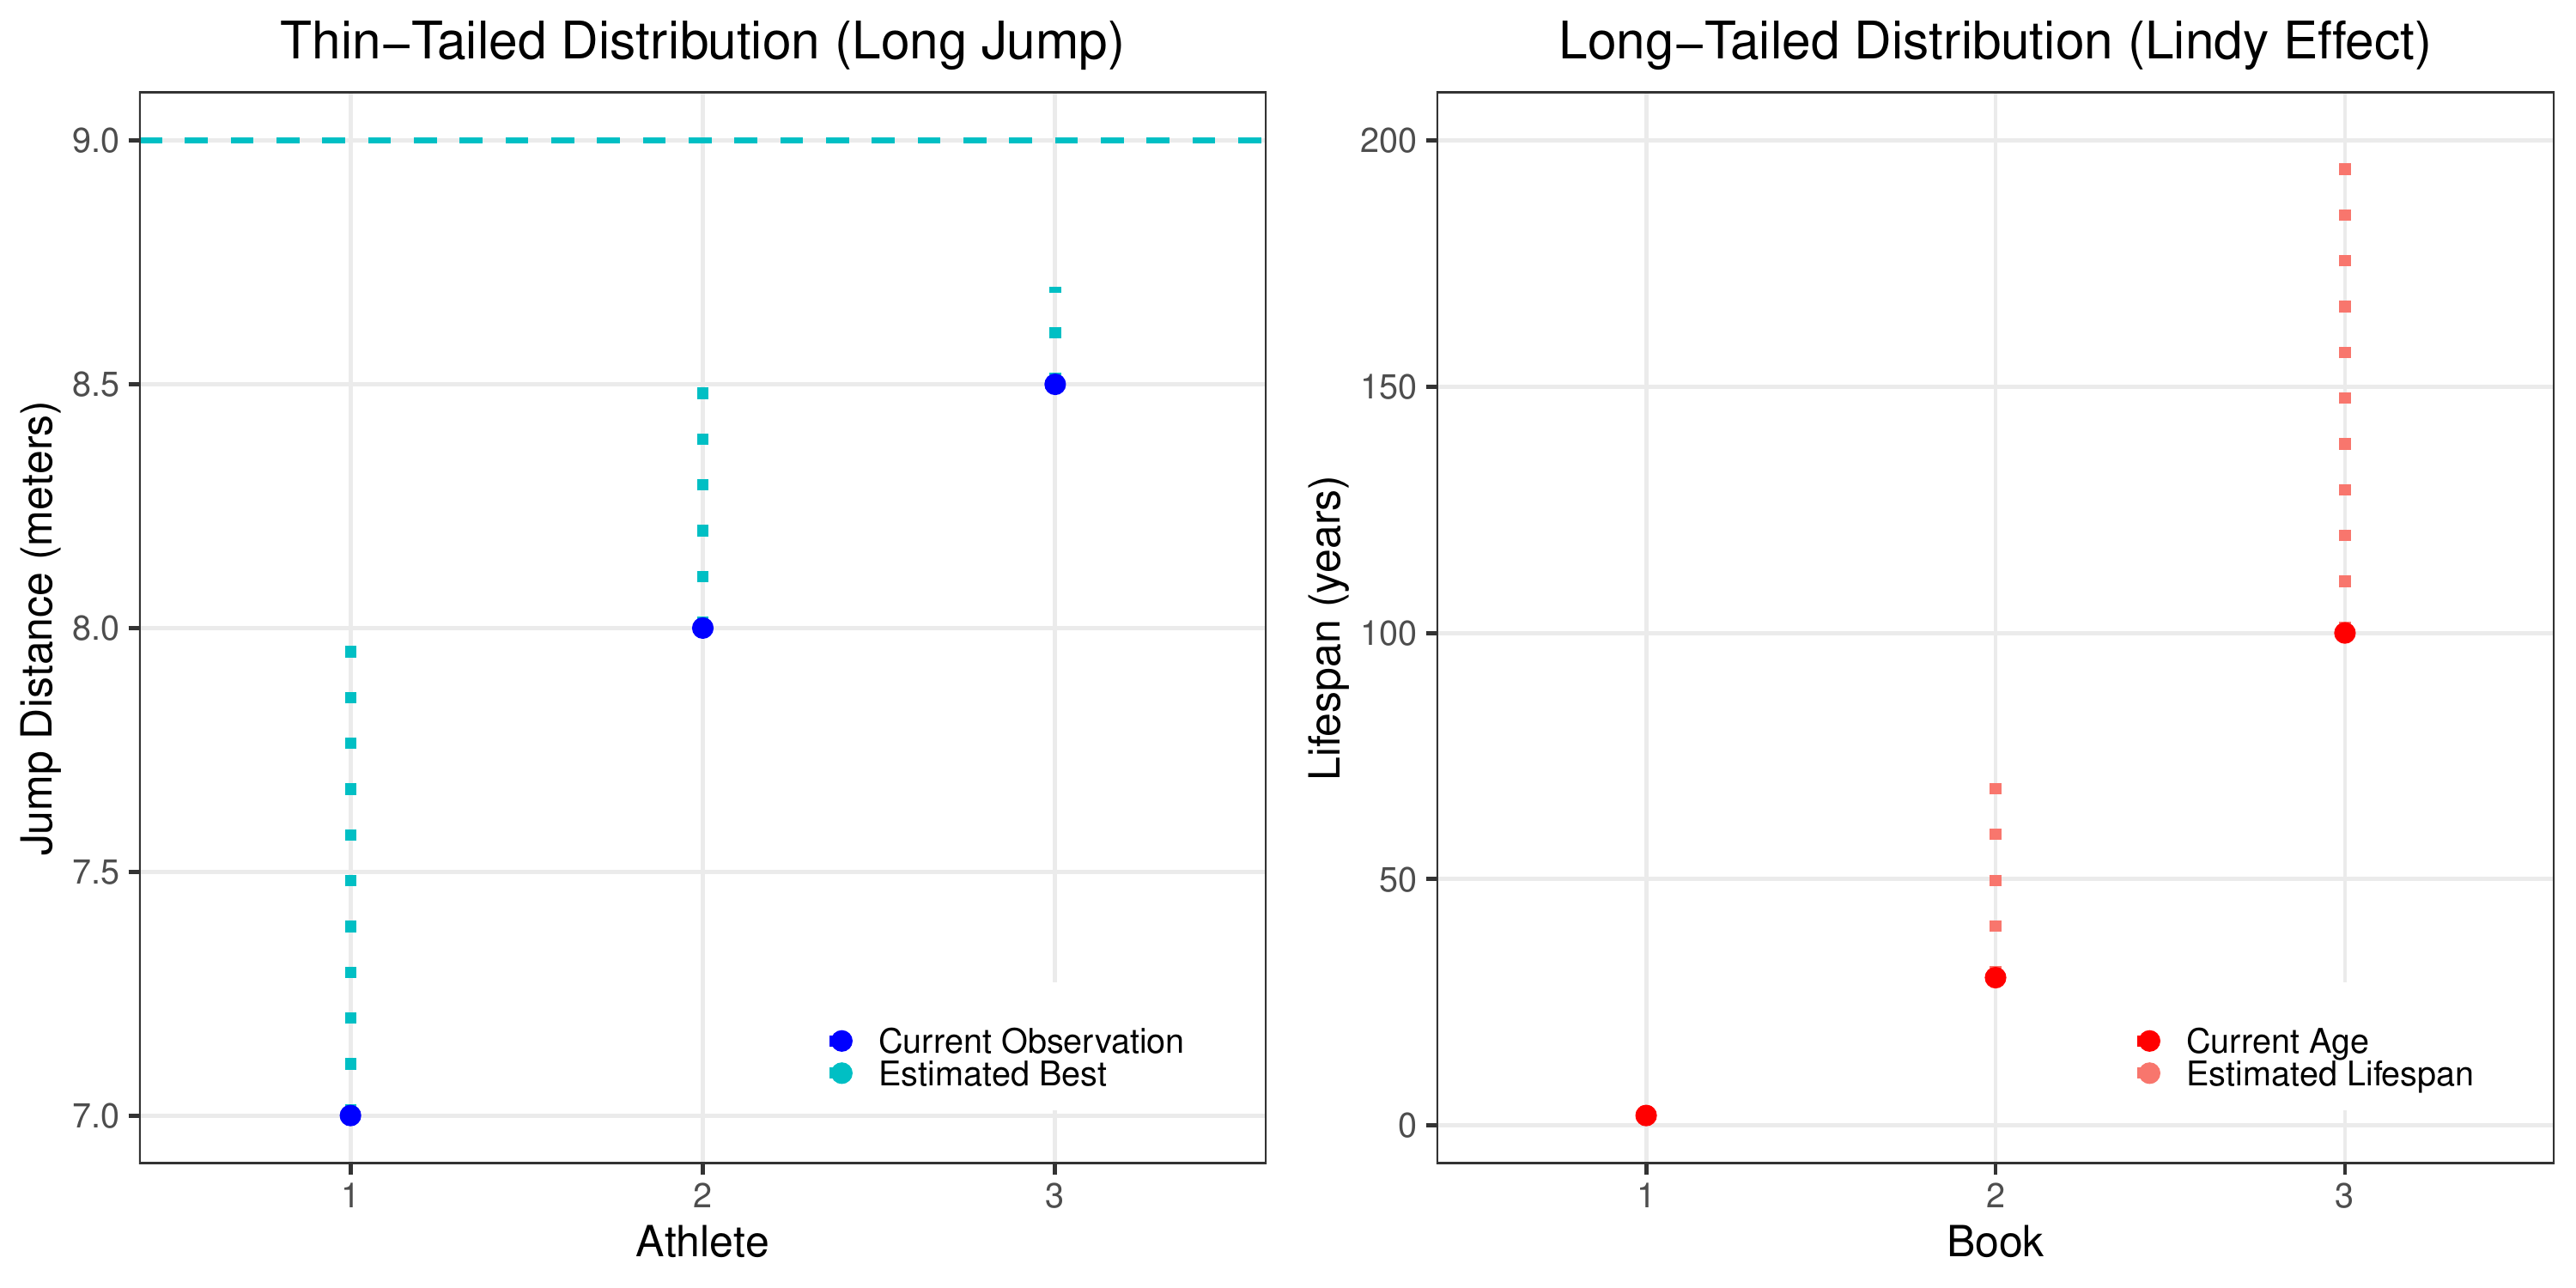}
    \caption{Our excess conditional expectation when observing long jumps (thin-tailed) shrinks as the jump gets better. By contrast, our excess conditional expectation when observing the lifespan of a book (long-tailed) gets larger as the book remains popular for longer.}
    \label{fig:excess}
\end{figure}

\paragraph{Example: Lindy Effect, Long Tails.} The Lindy Effect is the theory that, for certain types of entities, such as technologies and ideas, the longer they have been around, the longer we can expect them to survive into the future \citep{ord2023lindy}.\\

\noindent For example, if a book has been in print for two years, then it might remain in print for another two years. However, most books do not ``stand the test of time,'' so we might not expect it to survive another 100 years. Meanwhile, if another book has already been in print for 100 years, then we might well expect it to remain so for another 100 because it has showed it is robust to the test of time; if it has already remained relevant and interesting for a long time, then it is more likely to continue to do so for a long time into the future.\\

\noindent Figure \ref{fig:excess} shows some hypothetical observations of the current ages of books as blue lines, and our estimate of what their actual lifespan will be in dotted lines. Notice how, as the known lower bound of lifespan increases, the amount of additional time we expect a book to survive also increases.

\paragraph{Under long tails, excess conditional expectation grows as values become more extreme.} Under long tails, values of individual occurrences can grow much more extreme compared to the majority. There is not usually as clear a limit on long-tailed variables as on thin-tailed variables, so there is more room for the actual value to differ from the known minimum value, even if the latter is already extreme.\\

\noindent To differentiate between thin- and long-tailed distributions, we have now explored excess conditional distribution, a measure of the difference between our expectation of real-world values and the thresholds we observe them to exceed. Next, we will consider how variables arise: multiplicatively or additively.

\paragraph{Multiplicative and additive phenomena}
One factor in determining whether a variable is likely to have a long-tailed or thin-tailed distribution is whether it arises from a multiplicative or additive phenomenon. We will now look at the differences between these two categories of phenomena and why they affect how extreme a variable can become.

\paragraph{With multiplicative phenomena, one instance can multiply rapidly, triggering a cascade.} When something is a multiplicative phenomenon, individual instances are not independent of one another. Virus infections are a classic example of this; one infection is likely to seed several more infections, each of which can go on to cause even more. Thus, a single infection can trigger a cascade, so a virus outbreak has the potential to scale up considerably. This is part of the reason why virus outbreaks have a long-tailed distribution, with pandemics representing tail events.

\paragraph{With additive phenomena, individual instances do not tend to multiply.} When something is an additive phenomenon, individual events are largely independent of one another. Broken bones are an example of this; one person falling and breaking a bone does not usually trigger a cascade of other people falling and breaking bones. There may be instances where multiple broken bones occur together, for example in a car accident. However, in general, they are independently caused and do not have the potential to scale up as an infectious disease can. This means that tail events do not generally happen with this phenomenon; there is no single event where so many bones are broken that it significantly affects the average number of bones broken in accidents.

\paragraph{A high level of connectedness in a system gives rise to long tails.} Another way of thinking about this is to consider the level of connectedness in the relevant system. Since viruses are infectious, instances of infection are strongly connected to one another. Broken bones are not infectious, so instances of them are relatively isolated from one another. \\

\noindent We have seen that multiplicative phenomena are much more likely to result in long-tailed variables than additive ones. Next, we discuss another model which gives rise to long tails: preferential attachment.

\subsubsubsection{Preferential attachment}
\noindent \textbf{In preferential attachment processes, the more someone has, the more they will receive.} Preferential attachment processes are mechanisms where the amount extra of something that an individual will receive is positively correlated with the amount they already have. This is also known as the ``rich get richer'' effect because it is often illustrated with the example of wealth distribution; the more money a person already has, the more money they can invest, and thus the more additional money they can make through returns on their investments.

\noindent This effect applies to many phenomena within social systems. For example, if an author already has a lot of readers, there are more people who are likely to recommend their books to others. This author is therefore likely to gain more additional readers than someone else who starts out with fewer readers. Their sales can therefore snowball and become a tail event in the context of book sales. Similar mechanisms can also explain why a few social media platforms vastly outperform others, and why a few scientific papers receive many more citations than most.

\paragraph{Preferential attachment processes give rise to long tails \citep{Marsden2017}.} In situations where preferential attachment processes take place, events are not independent of one another. This is why things like book sales and wealth acquisition are multiplicative phenomena, where a single event can escalate to become much larger than most. By extension, this is why preferential attachment processes can produce long-tailed distributions.
